# Supplementary material for: Non-circular motions and the diversity of dwarf galaxy rotation curves
Source: arXiv:1706.07478 source file (2018-11-02)
Supplement: Supplementary file 1 [file supplementary.pdf]

# Apparent cores and non-circular motions in the H I discs of simulated galaxies: Supplementary materials

Kyle A. Oman[1,2⋆], Antonino Marasco[2,3], Julio F. Navarro[1,4], Carlos S. Frenk[5], Joop Schaye[6], Alejandro Benítez-Llambay[5]
[1] *Department of Physics & Astronomy, University of Victoria, Victoria, BC, V8P 5C2, Canada*
[2] *Kapteyn Astronomical Institute, University of Groningen, Postbus 800, NL-9700 AV Groningen, The Netherlands*
[3] *ASTRON, Netherlands Institute for Radio Astronomy, Postbus 2, 7900 AA, Dwingeloo, The Netherlands*
[4] *Senior CIfAR Fellow*
[5] *Institute for Computational Cosmology, Department of Physics, University of Durham, South Road, Durham DH1 3LE, United Kingdom*
[6] *Leiden Observatory, Leiden University, PO Box 9513, NL-2300 RA Leiden, the Netherlands*

20 August 2018

In the figures below we pick a single random orientation ($\Phi = 0$) for each of the 33 APOSTLE galaxies in our sample and show the first 3 moment maps, the position-velocity diagram and a summary of the $^{3\mathrm{D}}$BAROLO rotation curve fit for this orientation.

### Moment maps

Panels and symbols are as in Fig. 2 of the main article.

### Position-velocity diagrams

The left and right panels correspond to a 30 arcsec-wide ($\sim 500\,\mathrm{pc}$) slice along the kinematic major and minor axes, respectively. The filled contours show the flux in the synthetically observed data cube while the open contours show the same for the model data cube created using $^{3\mathrm{D}}$BAROLO. Contours are drawn at signal-to-noise levels of 0.3, 3 and 30, assuming a fiducial noise level of $0.4\,\mathrm{mJy\,beam}^{-1}$, similar to that of the THINGS survey. The heavy black line is the circular velocity curve, scaled by a factor of $\sin i$. The solid red line is the rotation curve as recovered using $^{3\mathrm{D}}$BAROLO. The dotted lines are the rotation curves recovered by modelling the approaching and receding sides separately.

### Rotation curve fit summaries

Panels and lines are as in Fig. 5 of the main article.

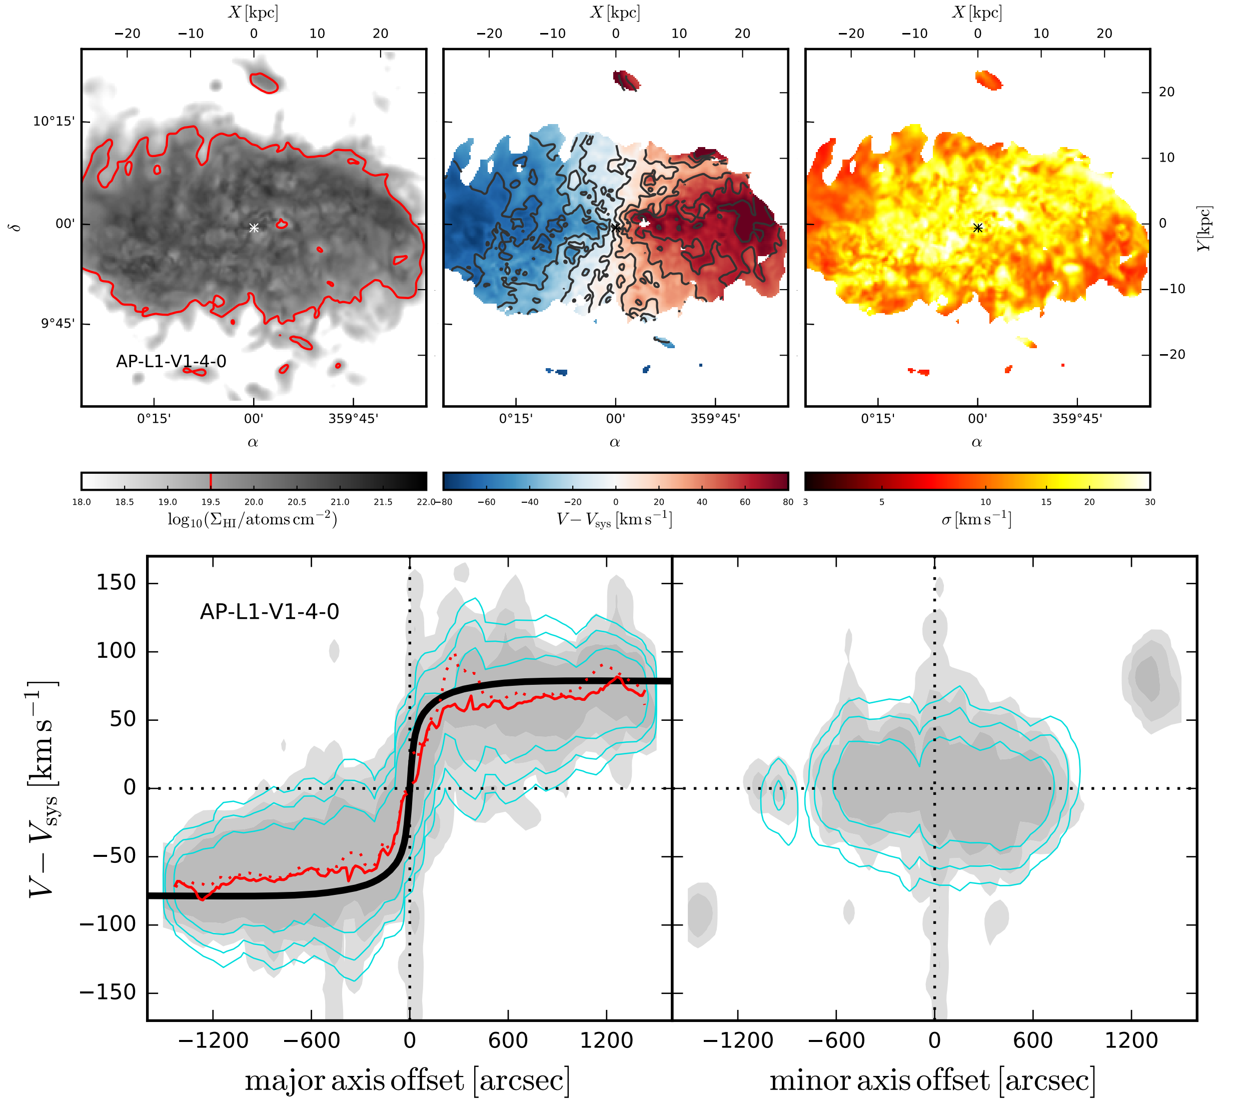


**Figure 1.** Moment maps, position-velocity diagrams and rotation curve fit summary (next page) for AP-L1-V1-4-0. See text for detailed description.

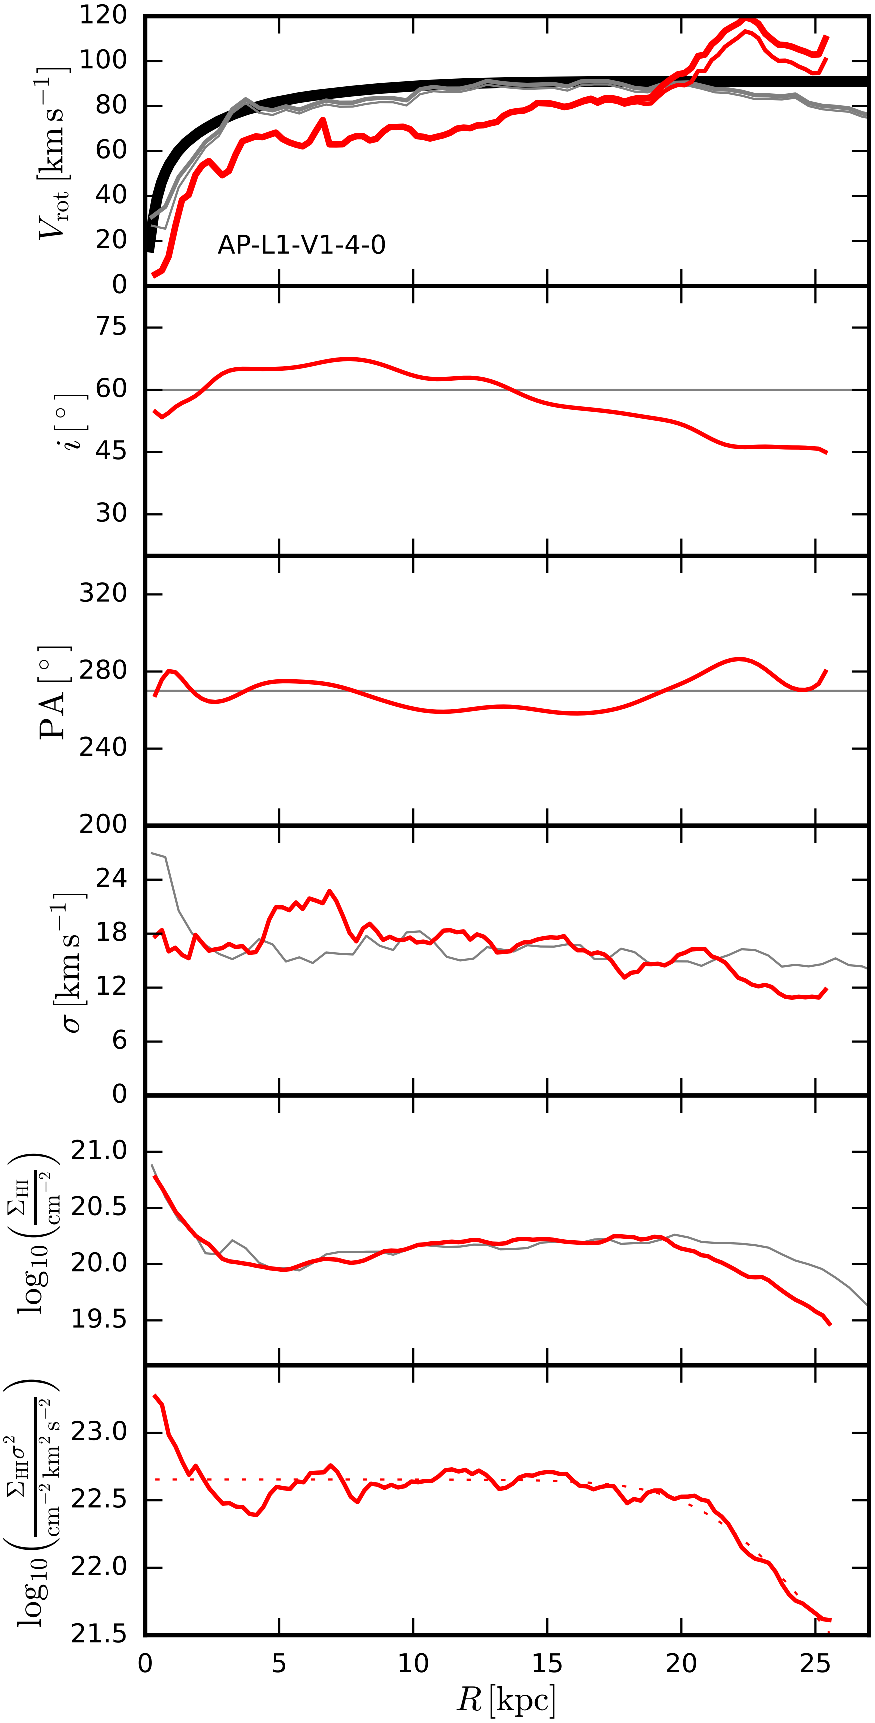


**Figure 1** – *continued*

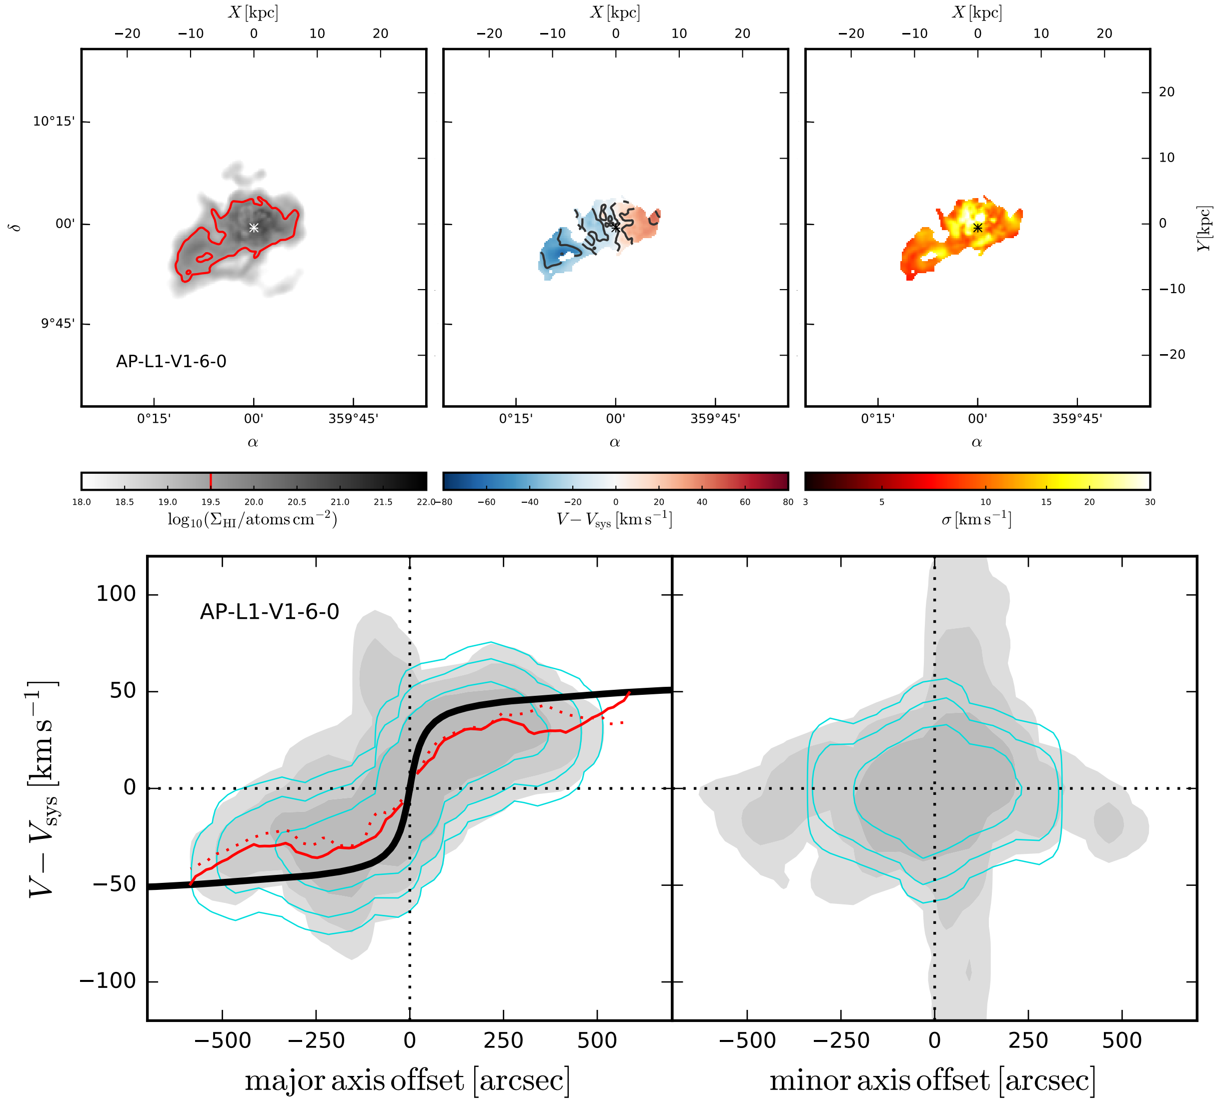


**Figure 2.** Moment maps, position-velocity diagrams and rotation curve fit summary (next page) for AP-L1-V1-6-0. See text for detailed description.

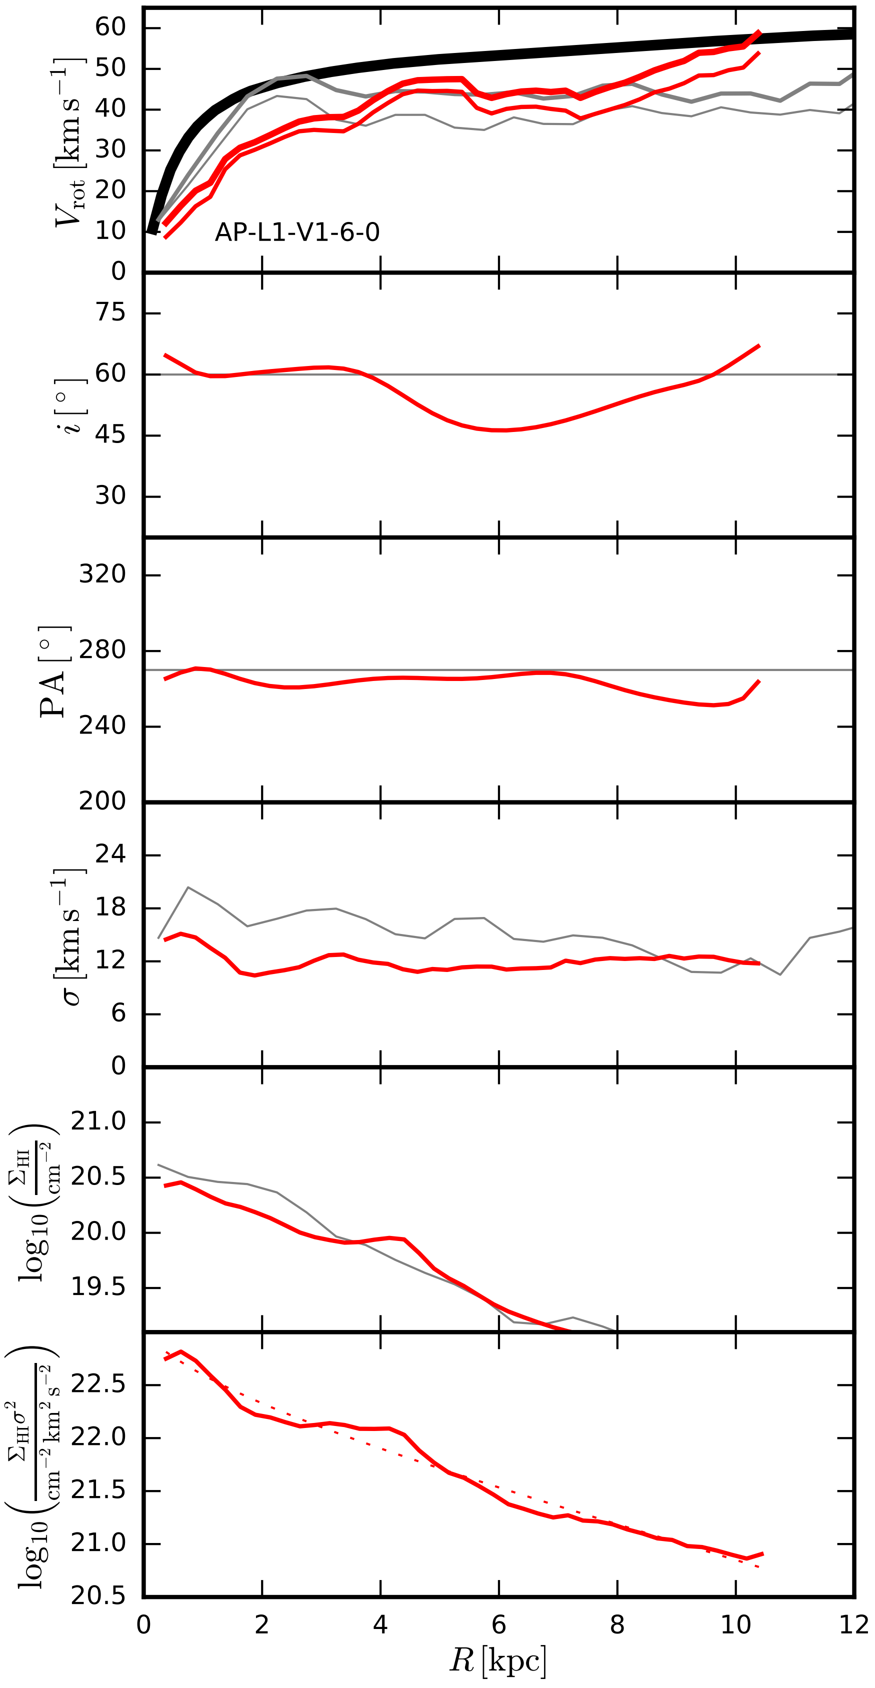


**Figure 2** – *continued*

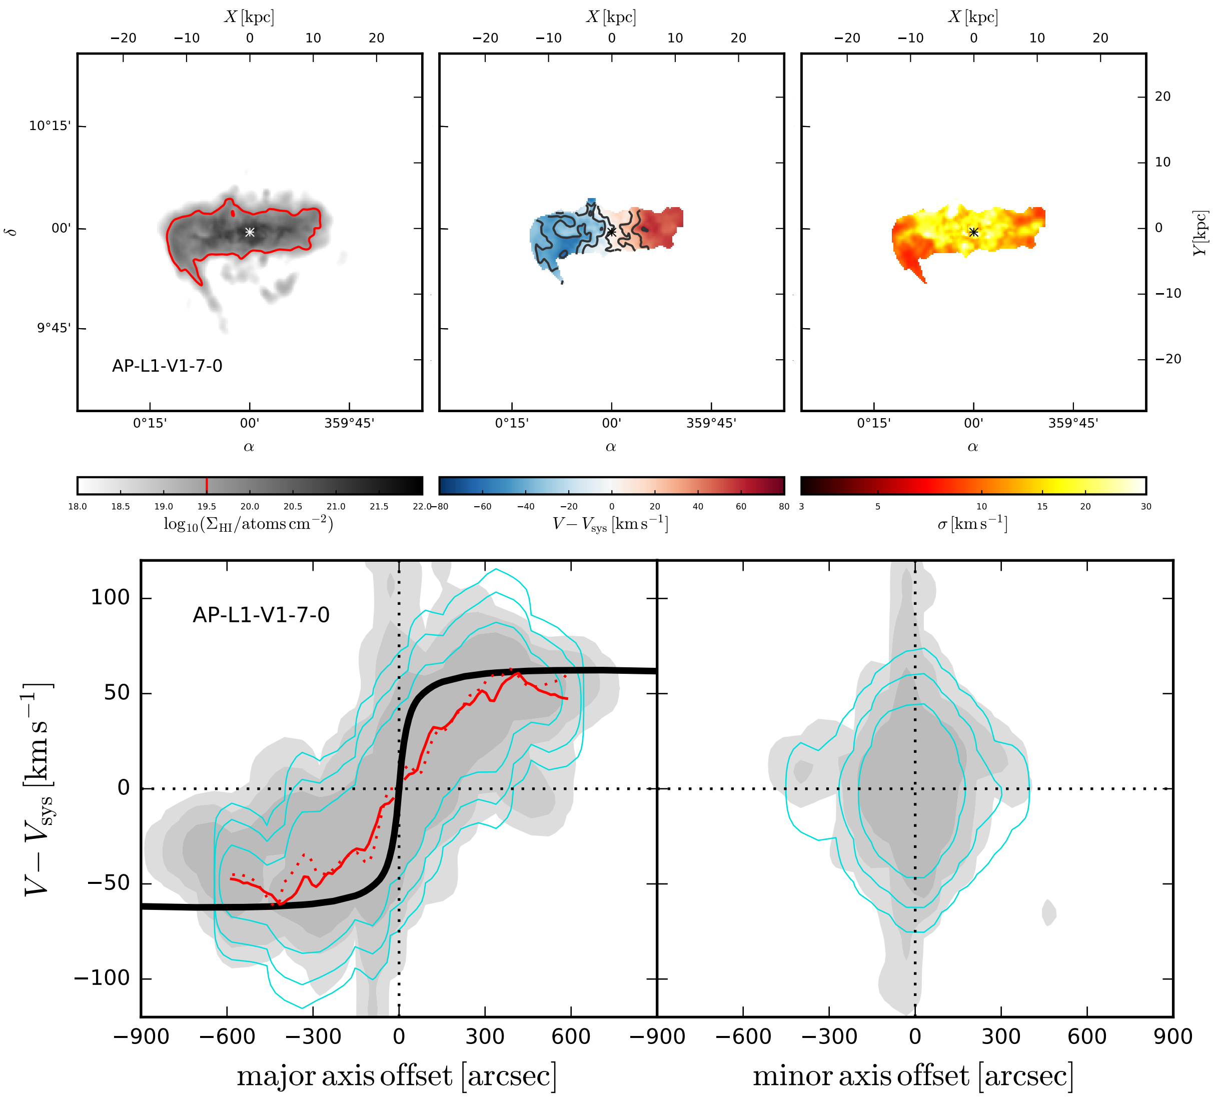


**Figure 3.** Moment maps, position-velocity diagrams and rotation curve fit summary (next page) for AP-L1-V1-7-0. See text for detailed description.

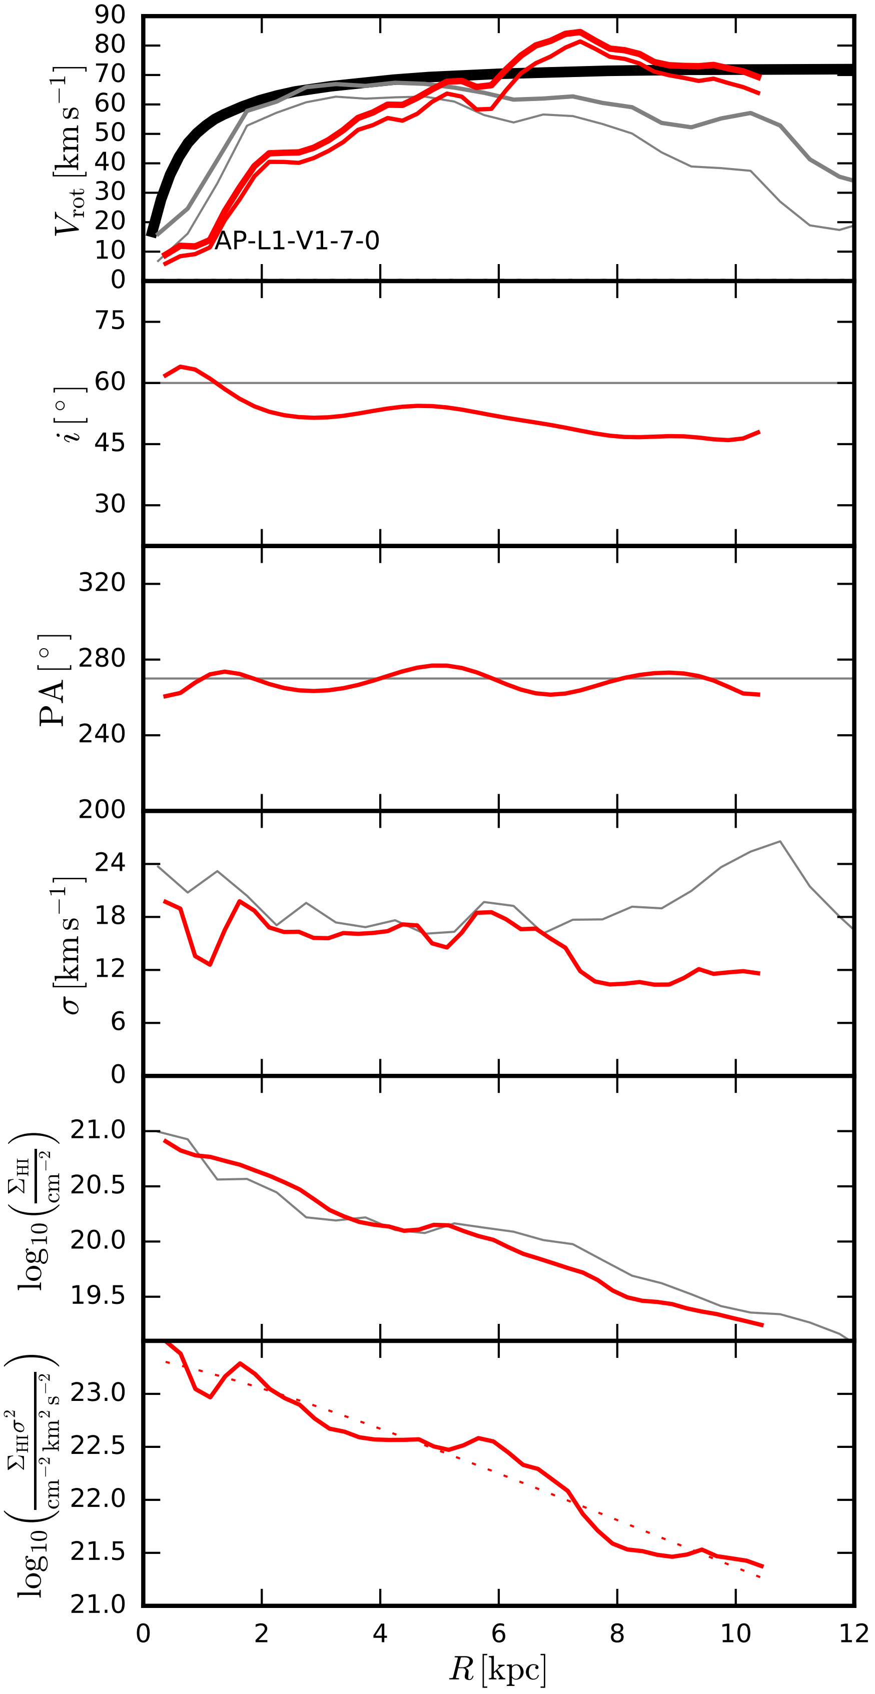


**Figure 3** – *continued*

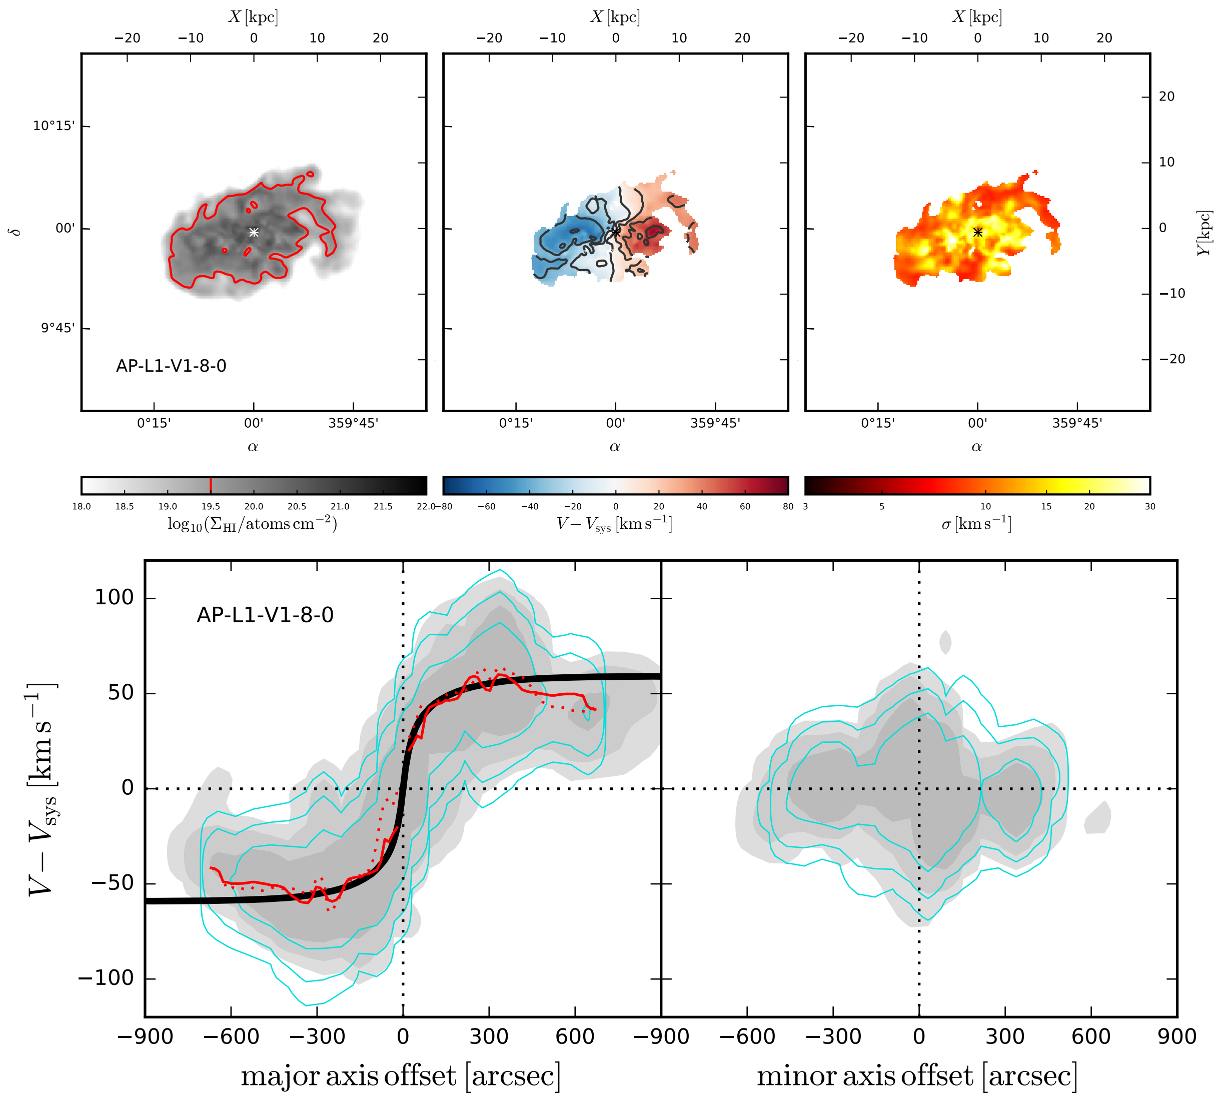


**Figure 4.** Moment maps, position-velocity diagrams and rotation curve fit summary (next page) for AP-L1-V1-8-0. See text for detailed description.

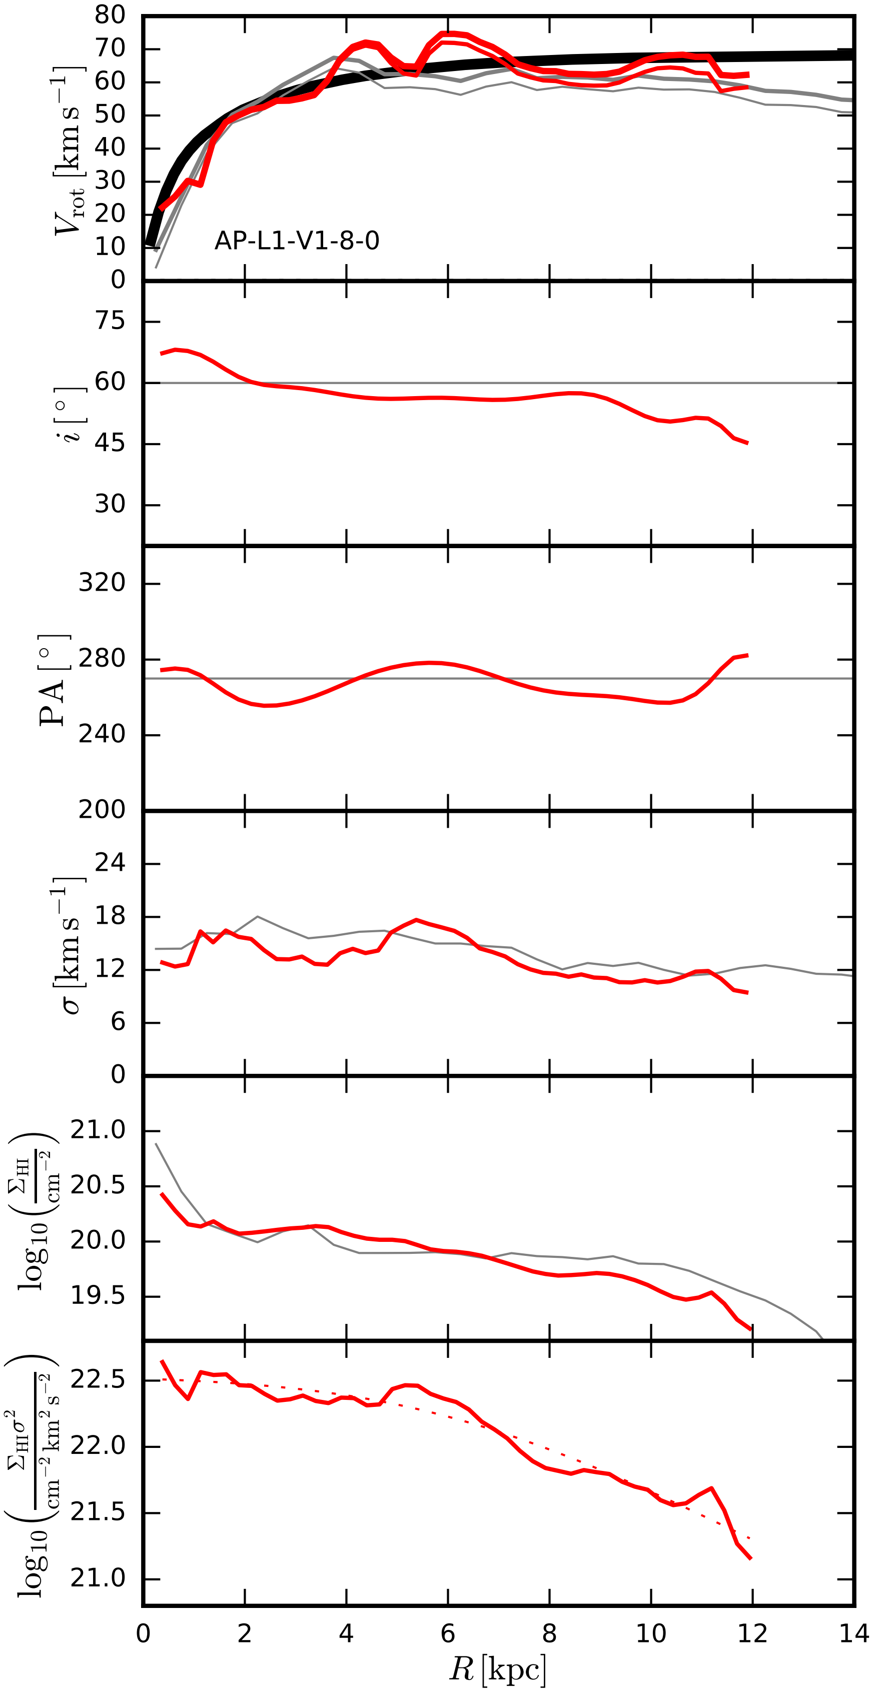


**Figure 4** – *continued*

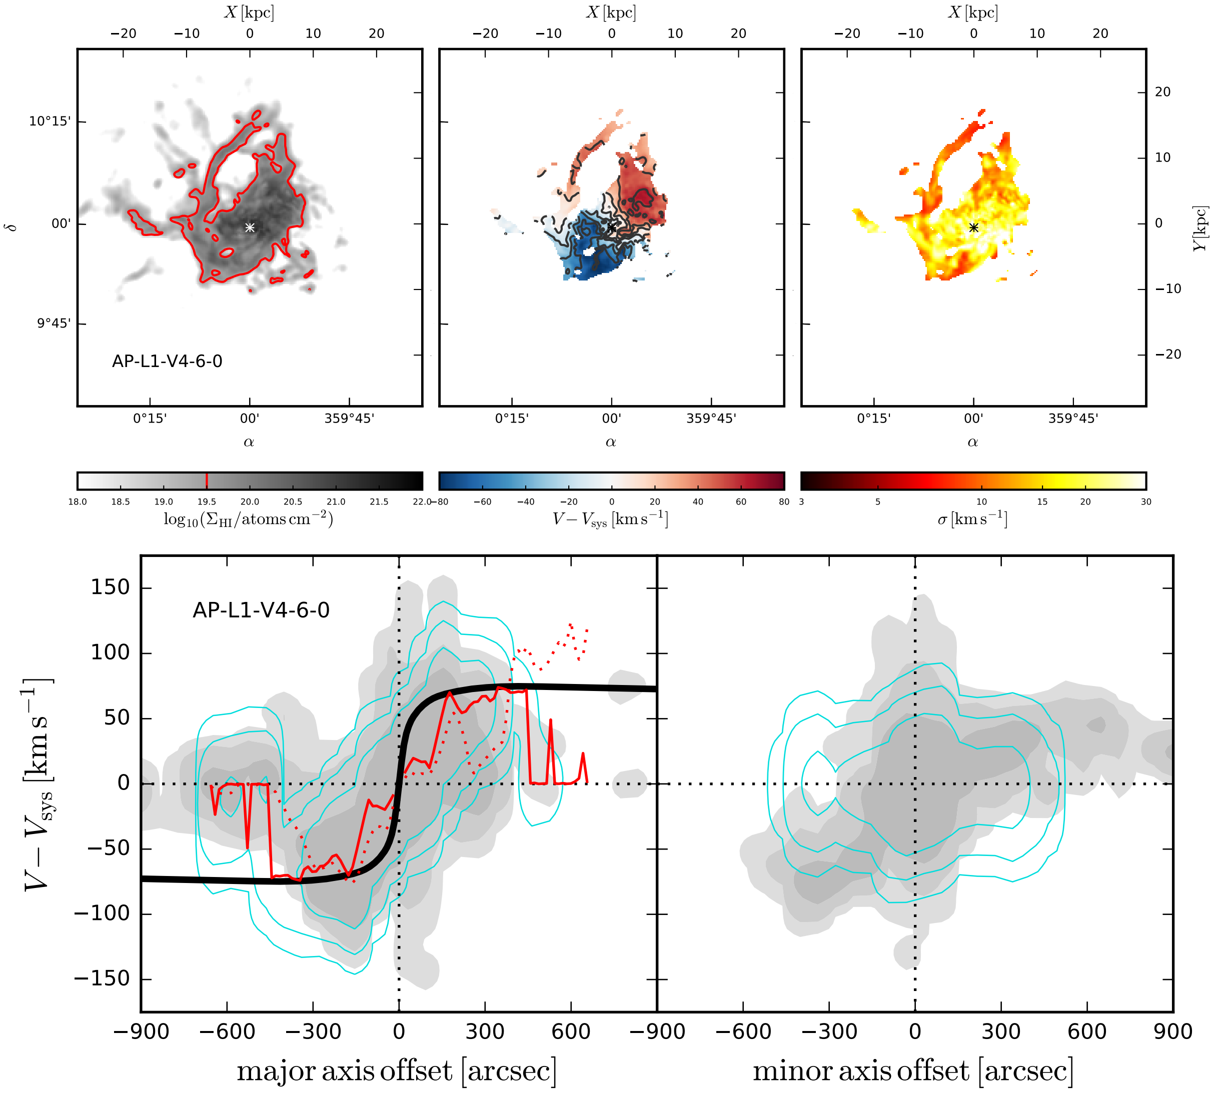


**Figure 5.** Moment maps, position-velocity diagrams and rotation curve fit summary (next page) for AP-L1-V4-6-0. See text for detailed description.

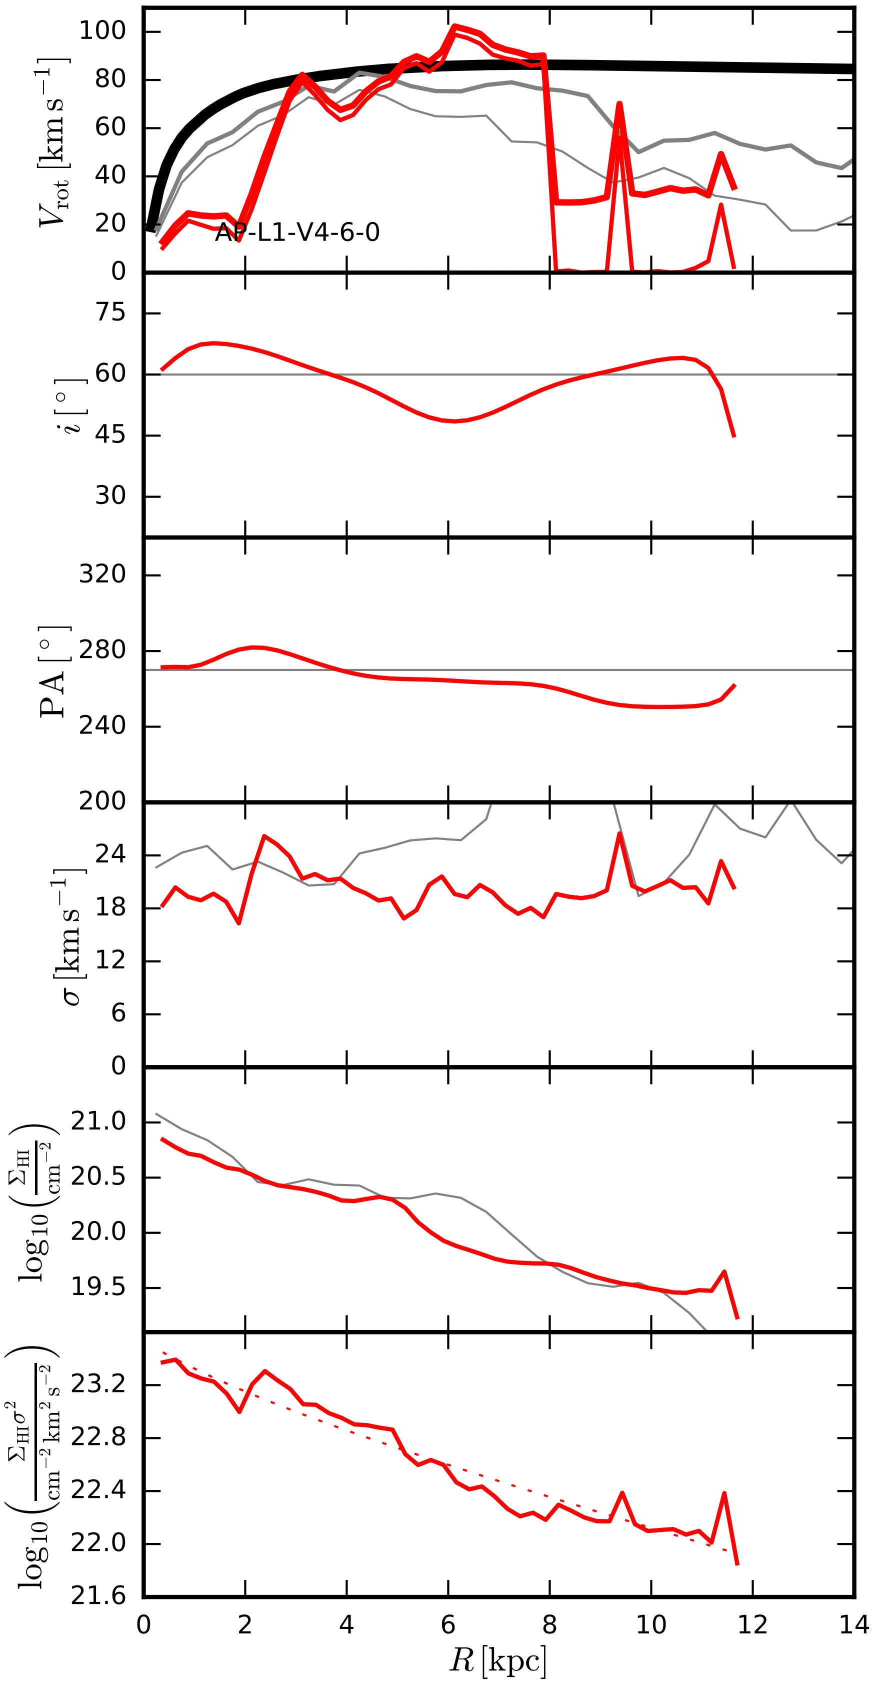


**Figure 5** – *continued*

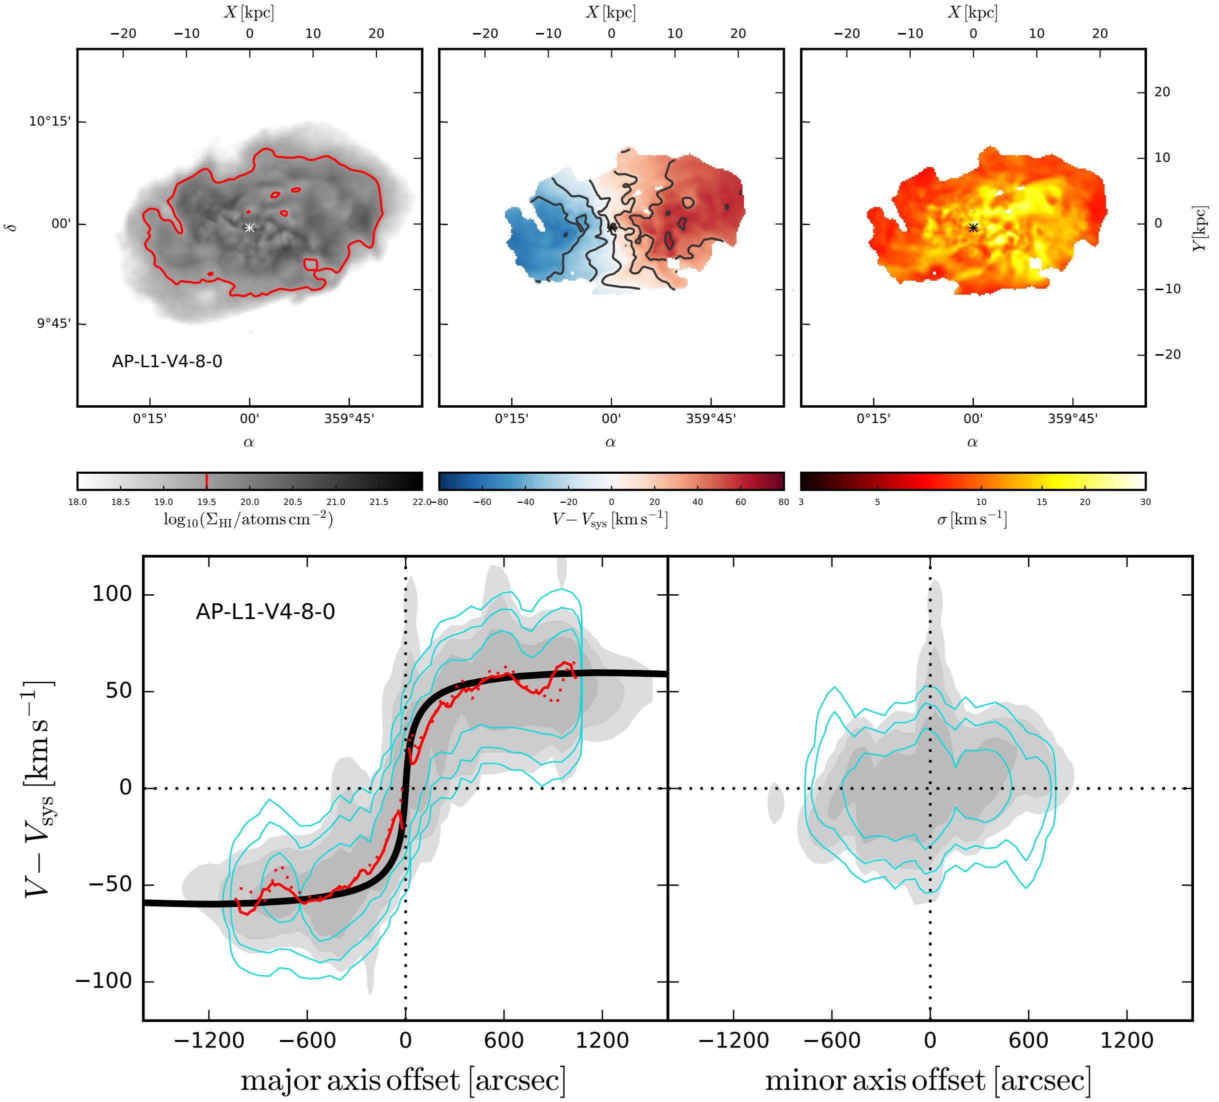


**Figure 6.** Moment maps, position-velocity diagrams and rotation curve fit summary (next page) for AP-L1-V4-8-0. See text for detailed description.

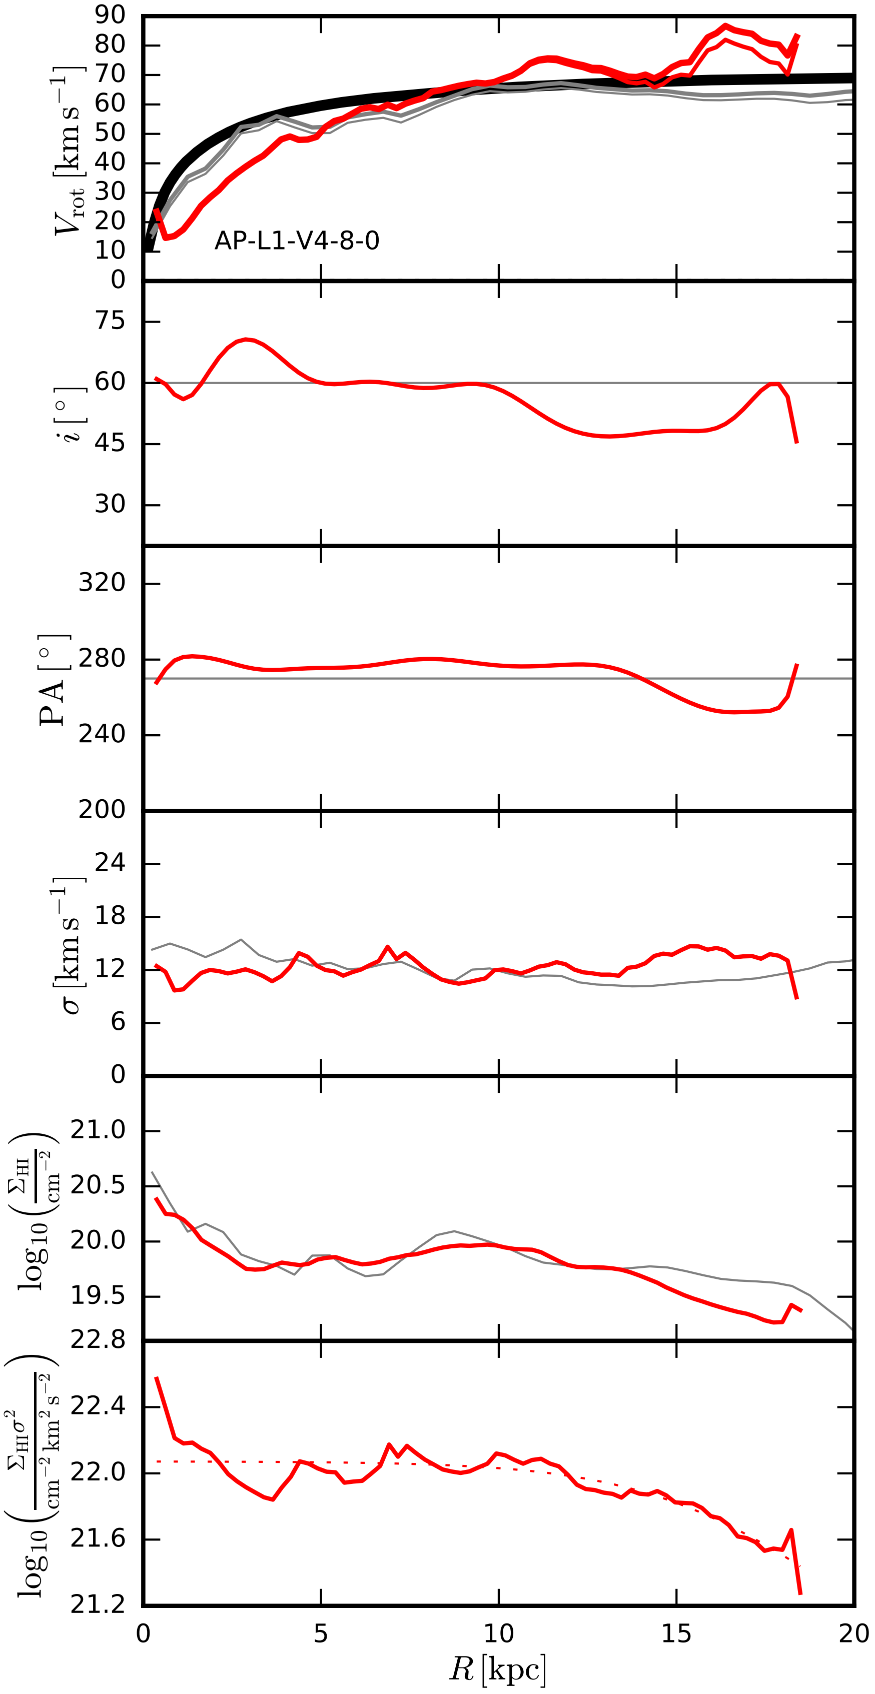


**Figure 6** – *continued*

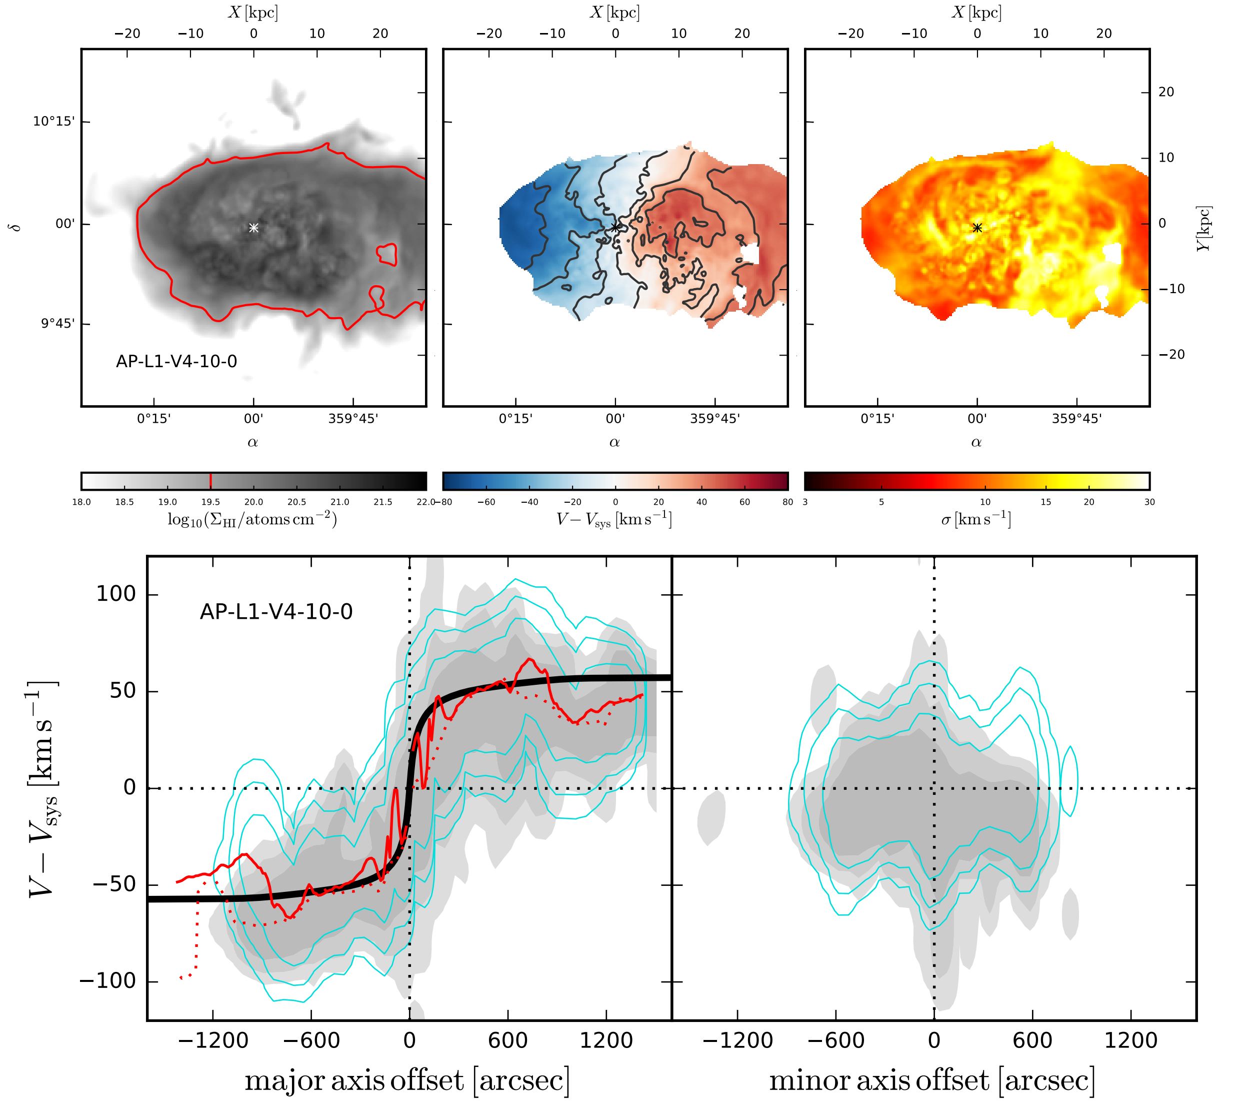


**Figure 7.** Moment maps, position-velocity diagrams and rotation curve fit summary (next page) for AP-L1-V4-10-0. See text for detailed description.

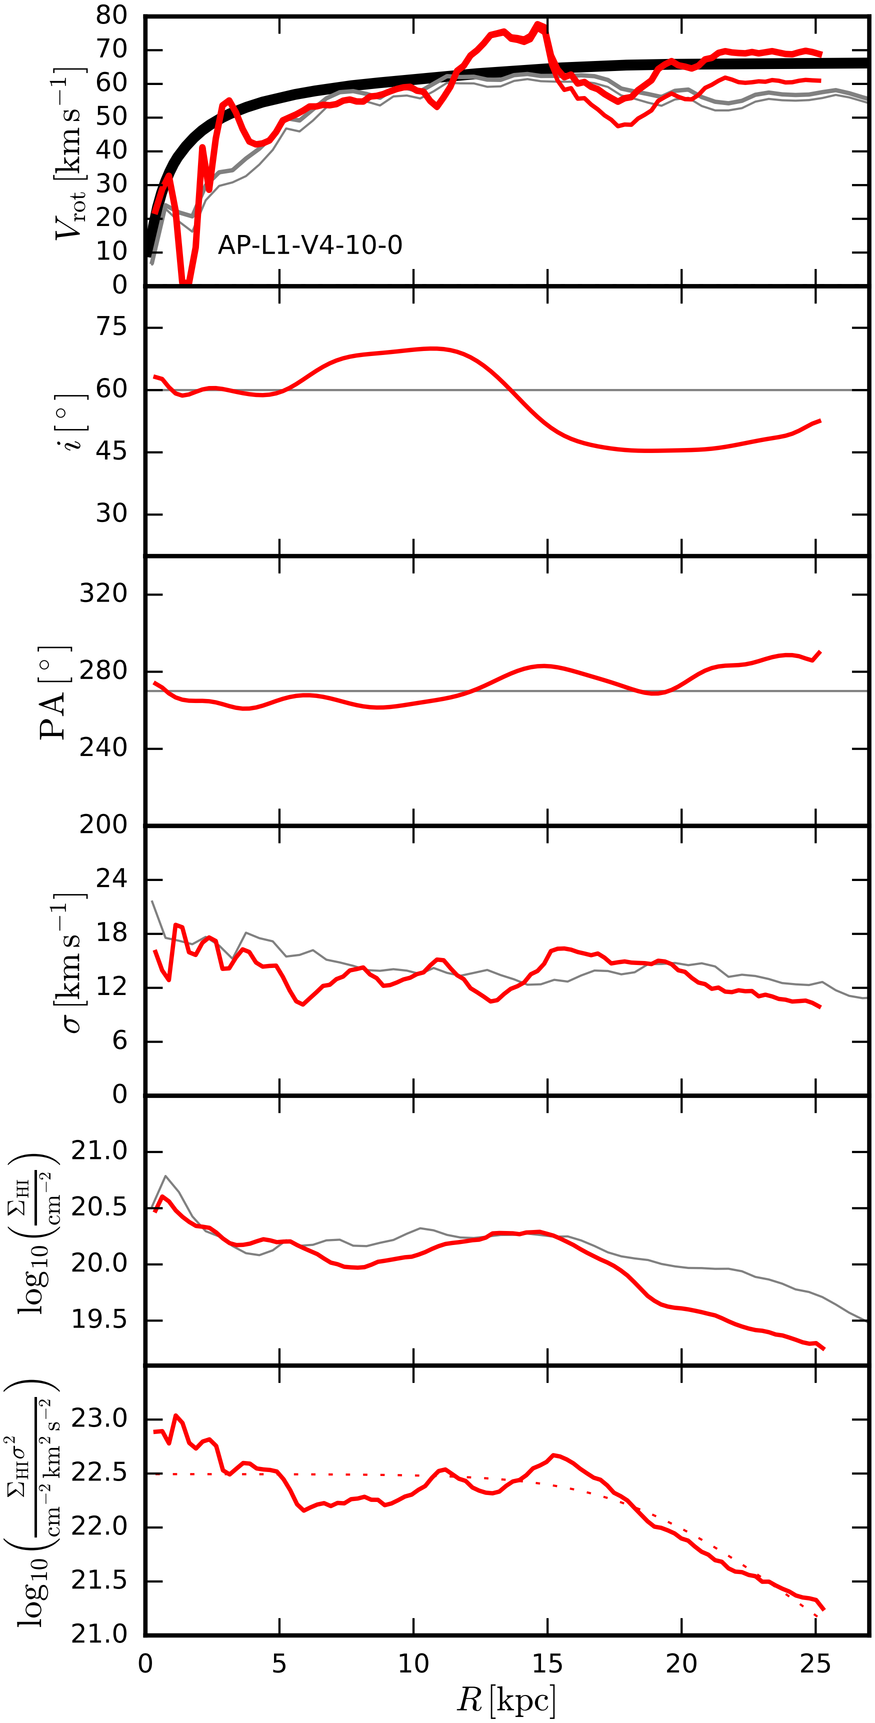


**Figure 7** – *continued*

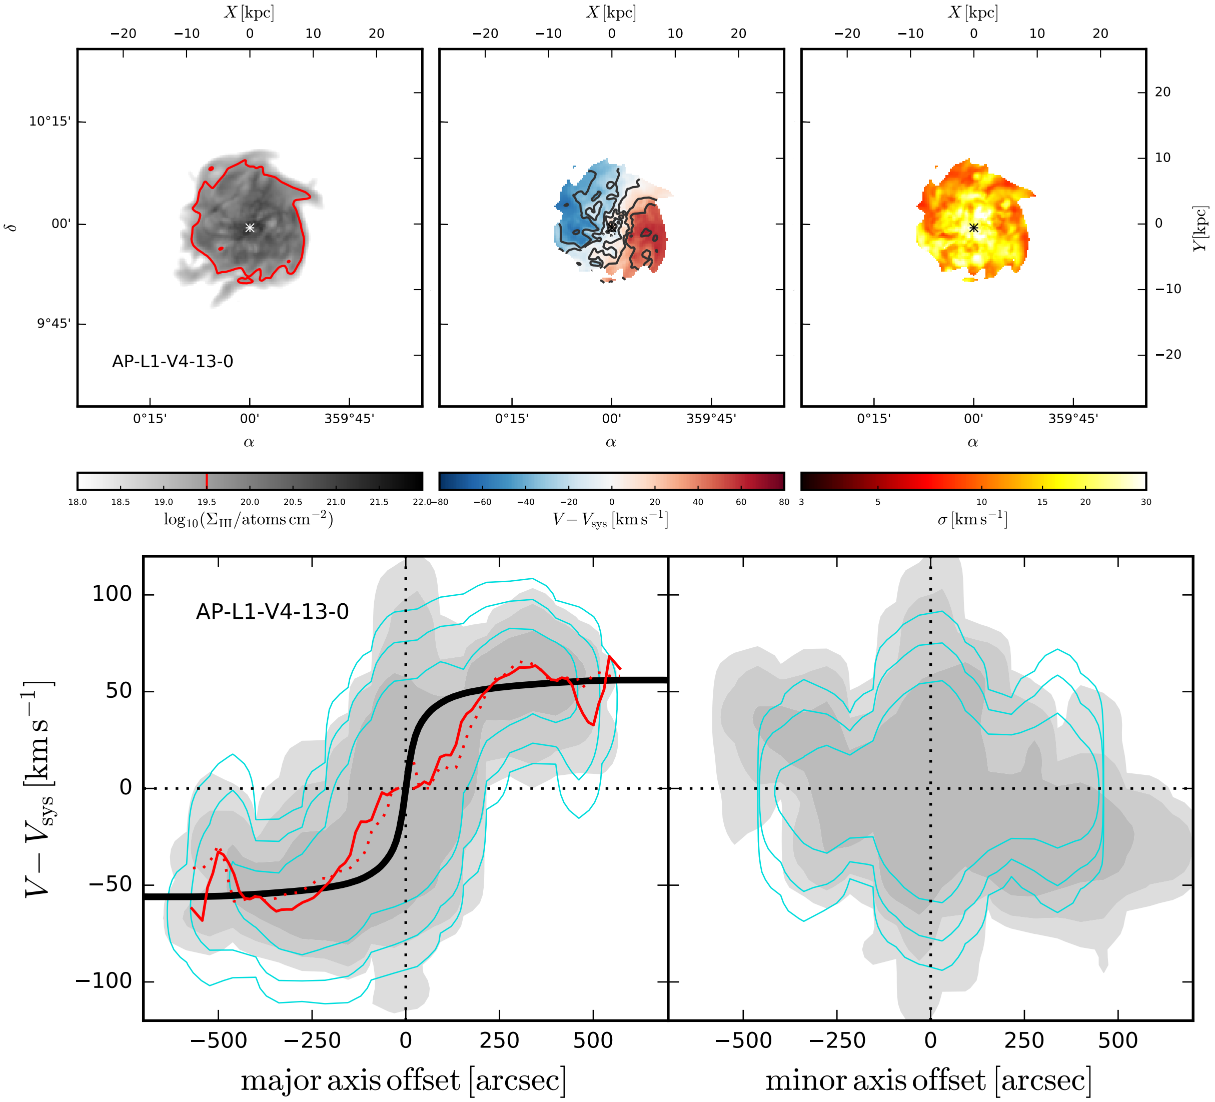


**Figure 8.** Moment maps, position-velocity diagrams and rotation curve fit summary (next page) for AP-L1-V4-13-0. See text for detailed description.

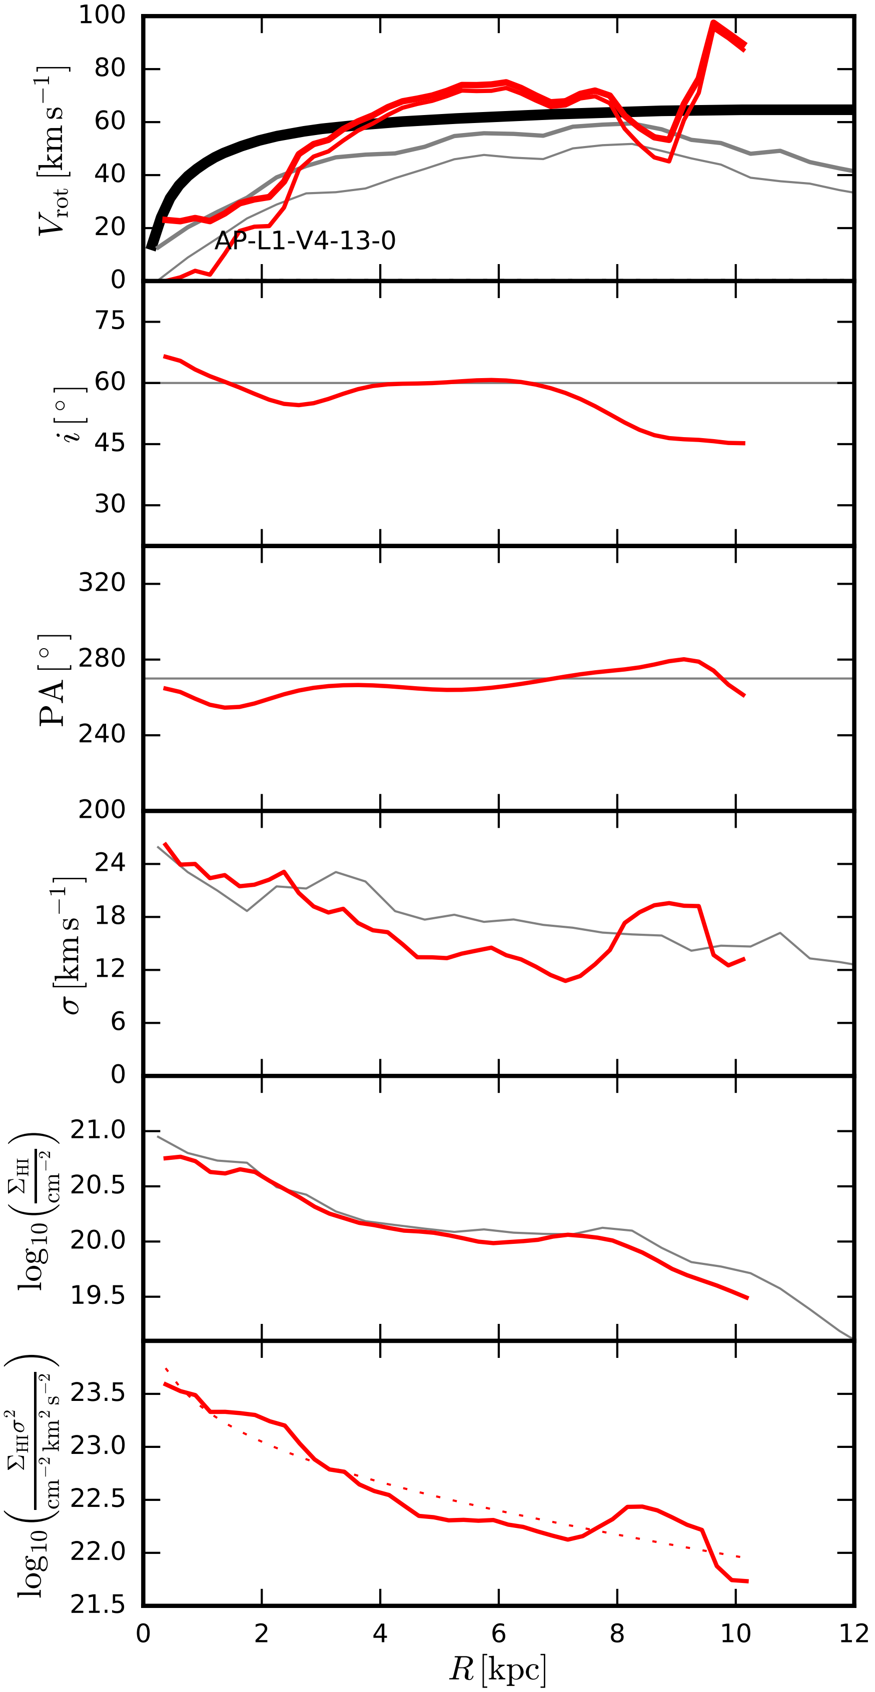


**Figure 8** – *continued*

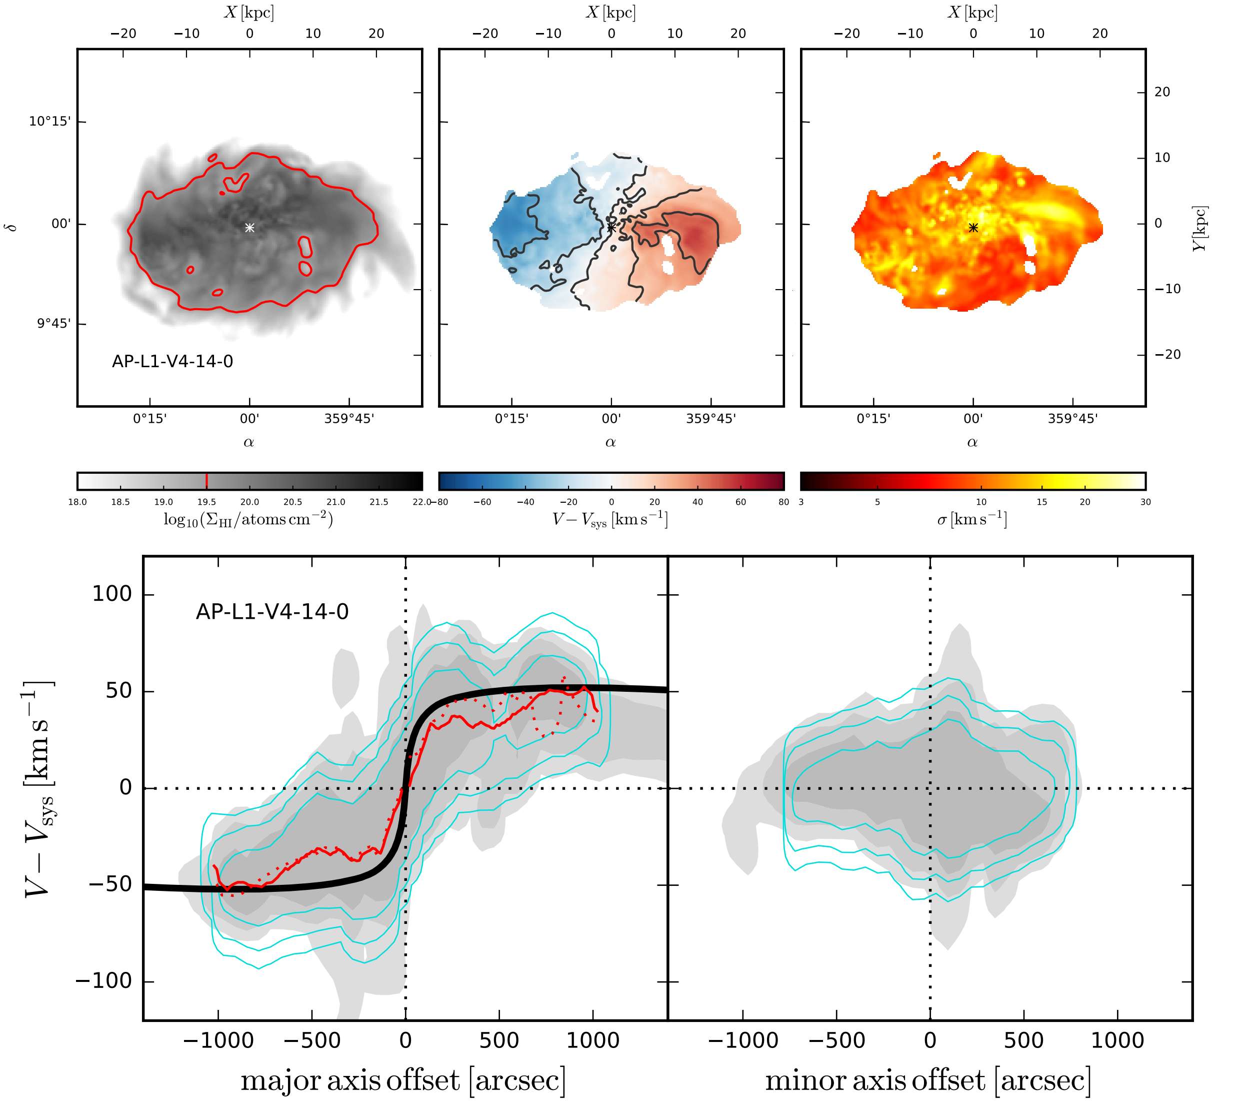


**Figure 9.** Moment maps, position-velocity diagrams and rotation curve fit summary (next page) for AP-L1-V4-14-0. See text for detailed description.

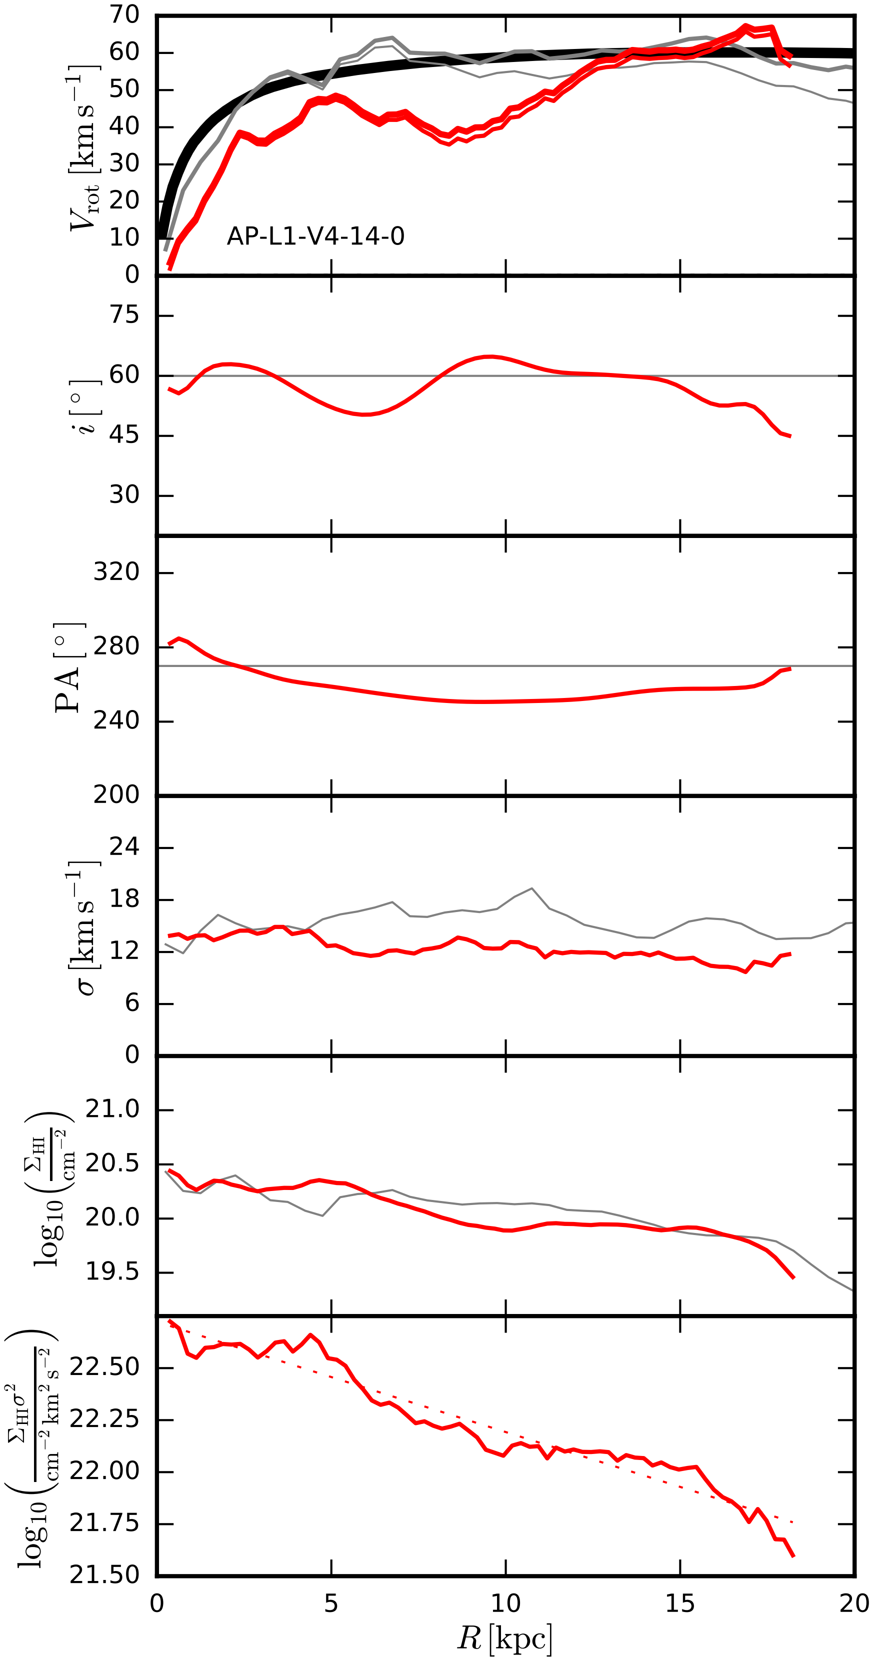


**Figure 9** – *continued*

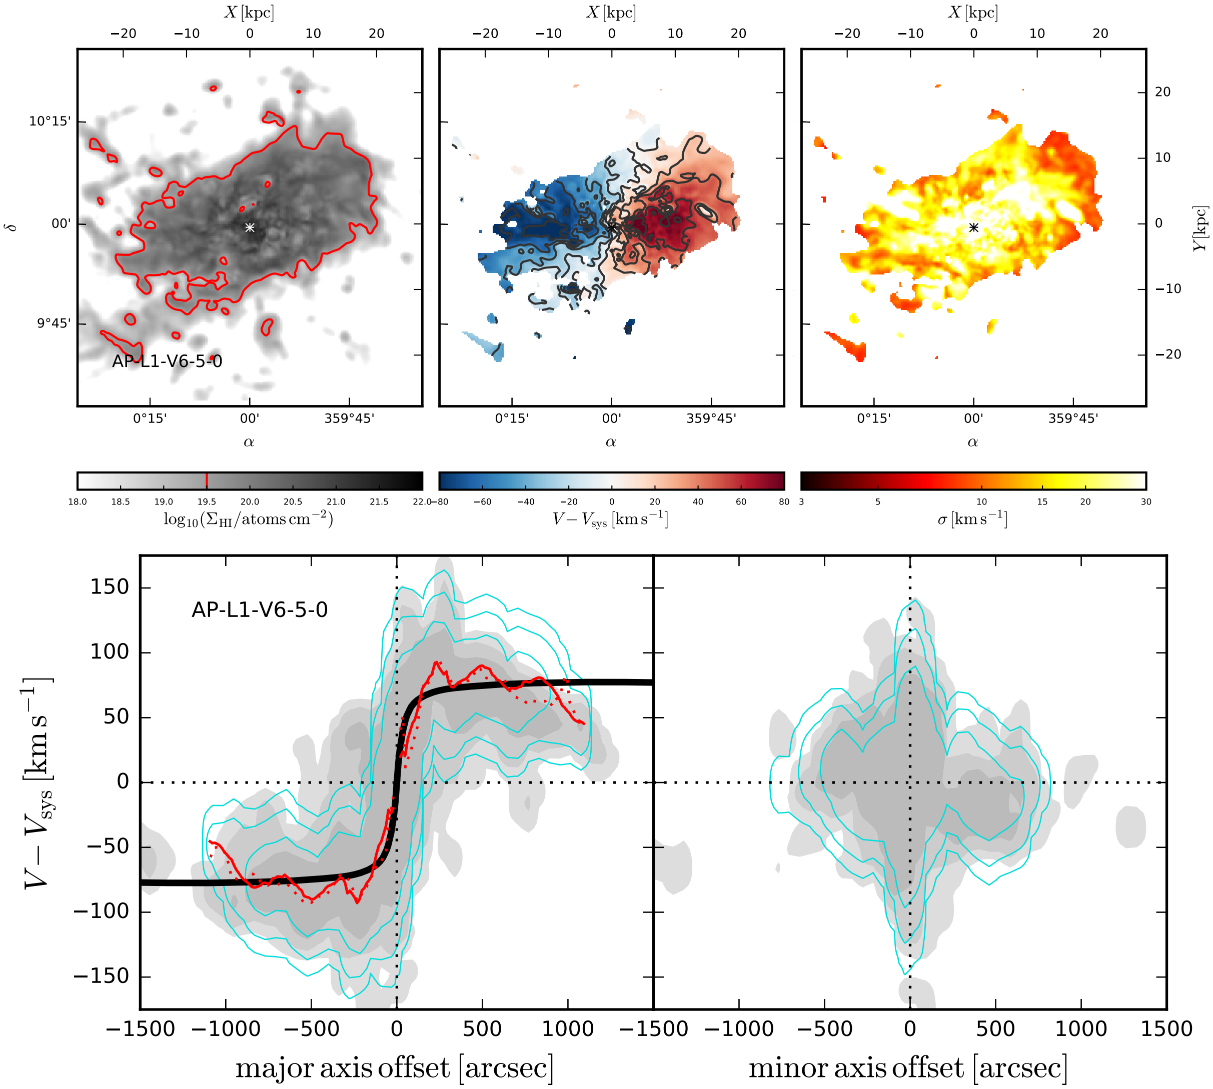


**Figure 10.** Moment maps, position-velocity diagrams and rotation curve fit summary (next page) for AP-L1-V6-5-0. See text for detailed description.

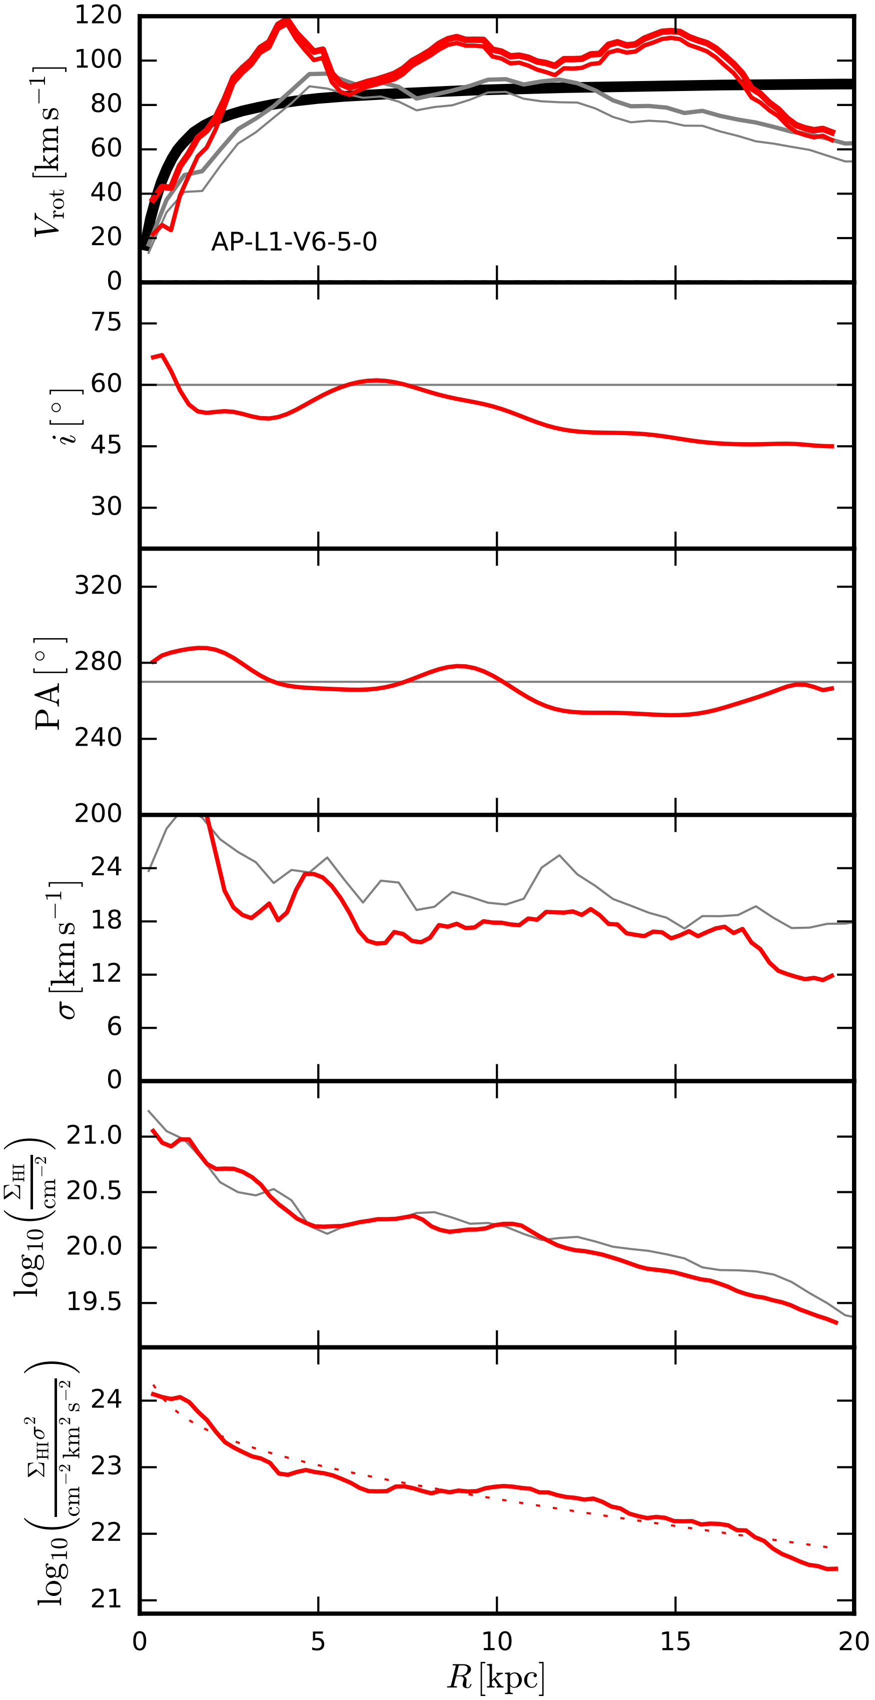


**Figure 10** – *continued*

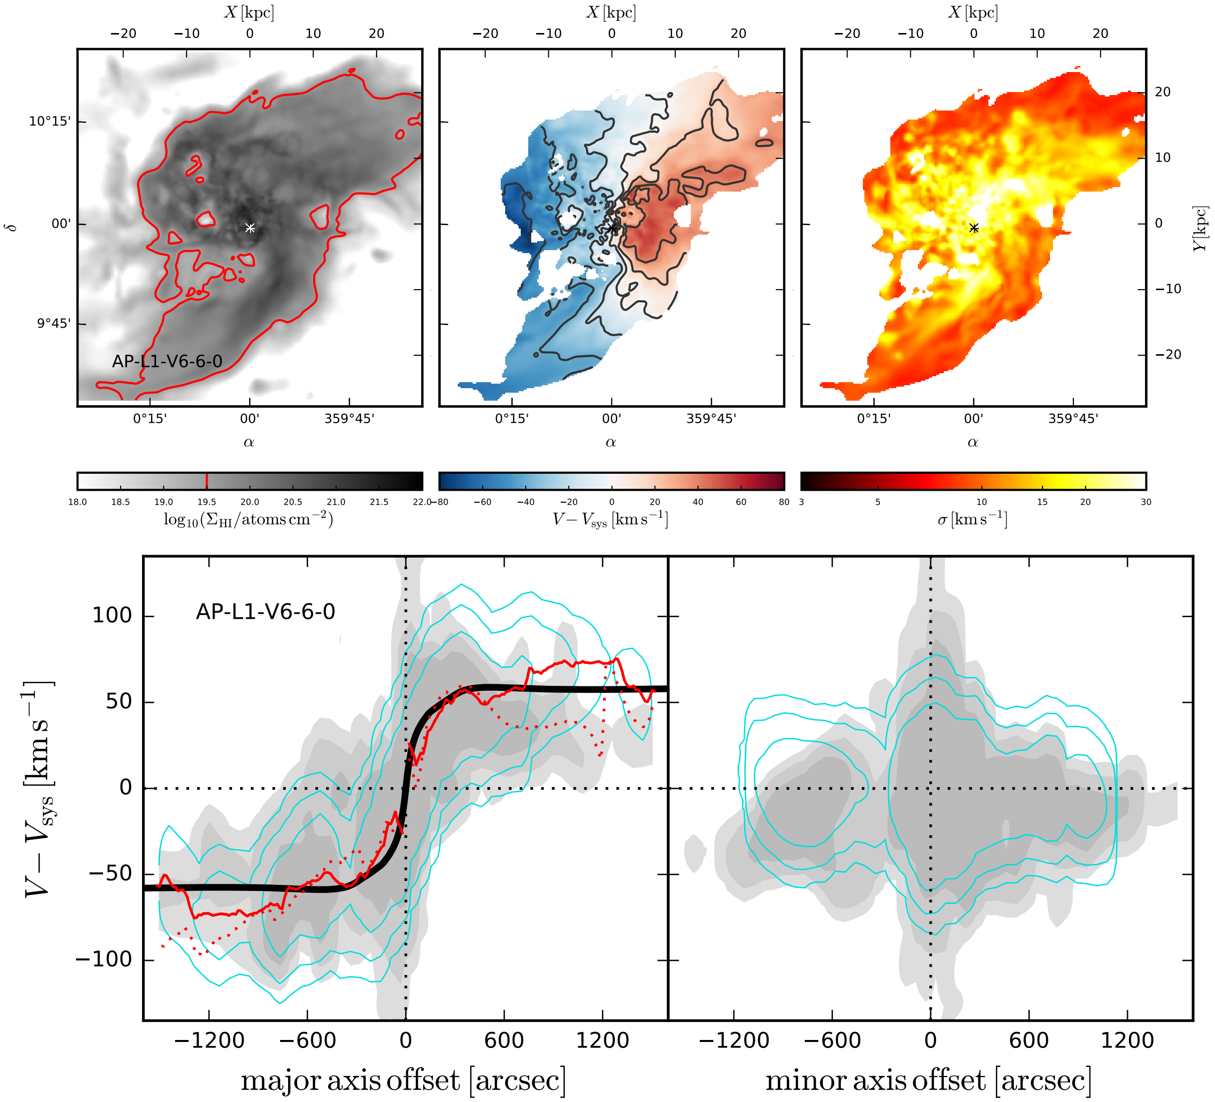


**Figure 11.** Moment maps, position-velocity diagrams and rotation curve fit summary (next page) for AP-L1-V6-6-0. See text for detailed description.

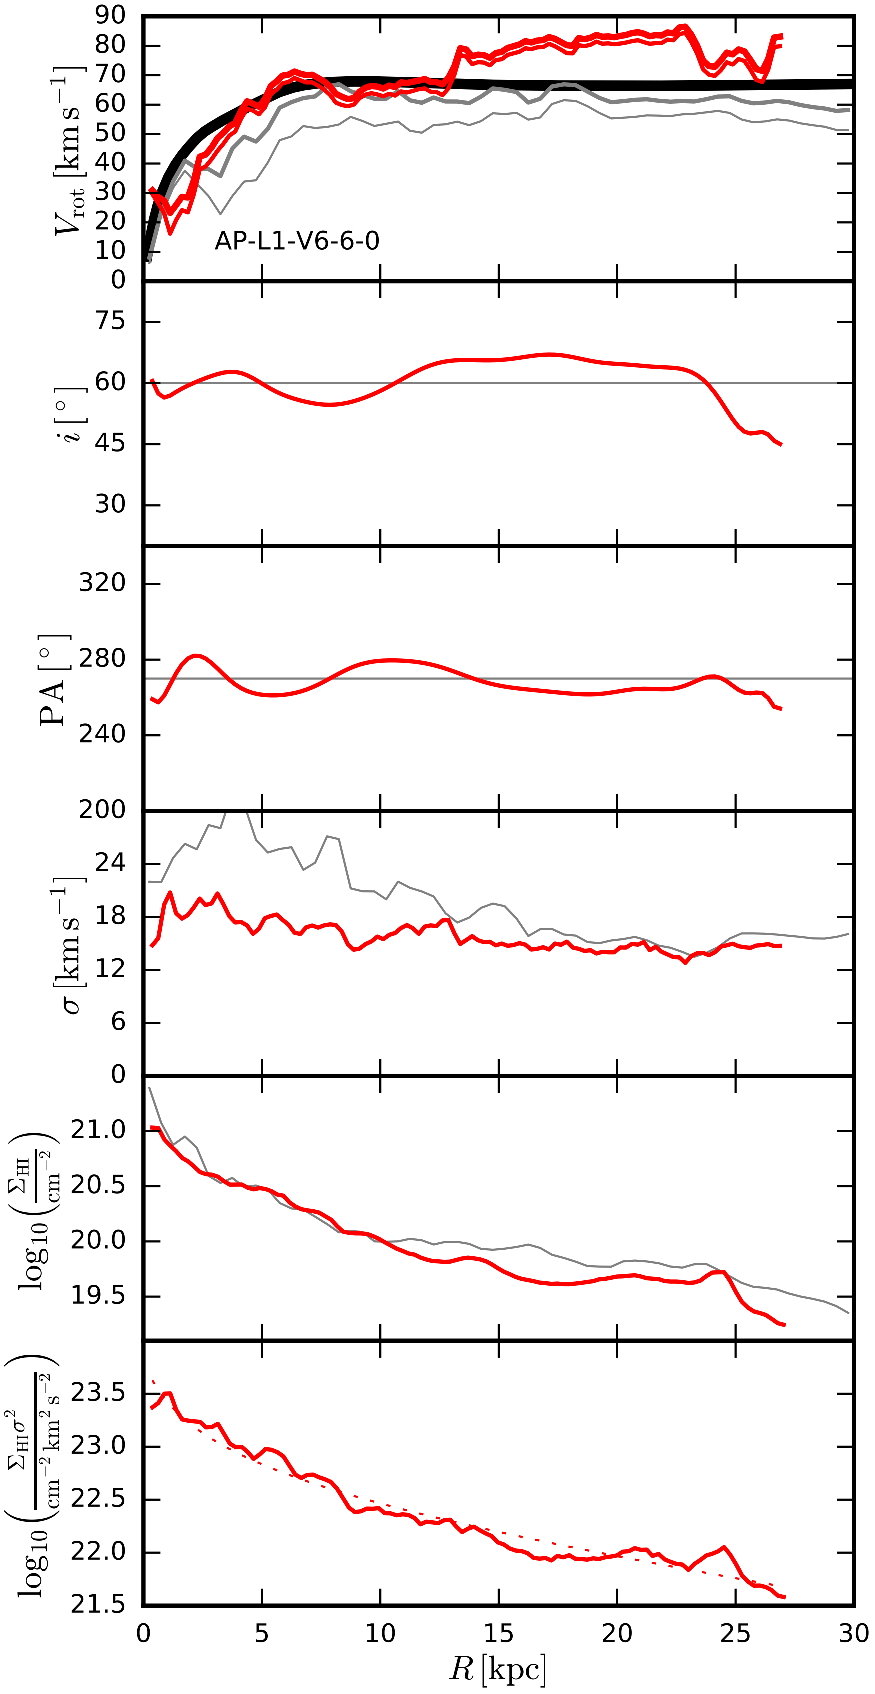


**Figure 11** – *continued*

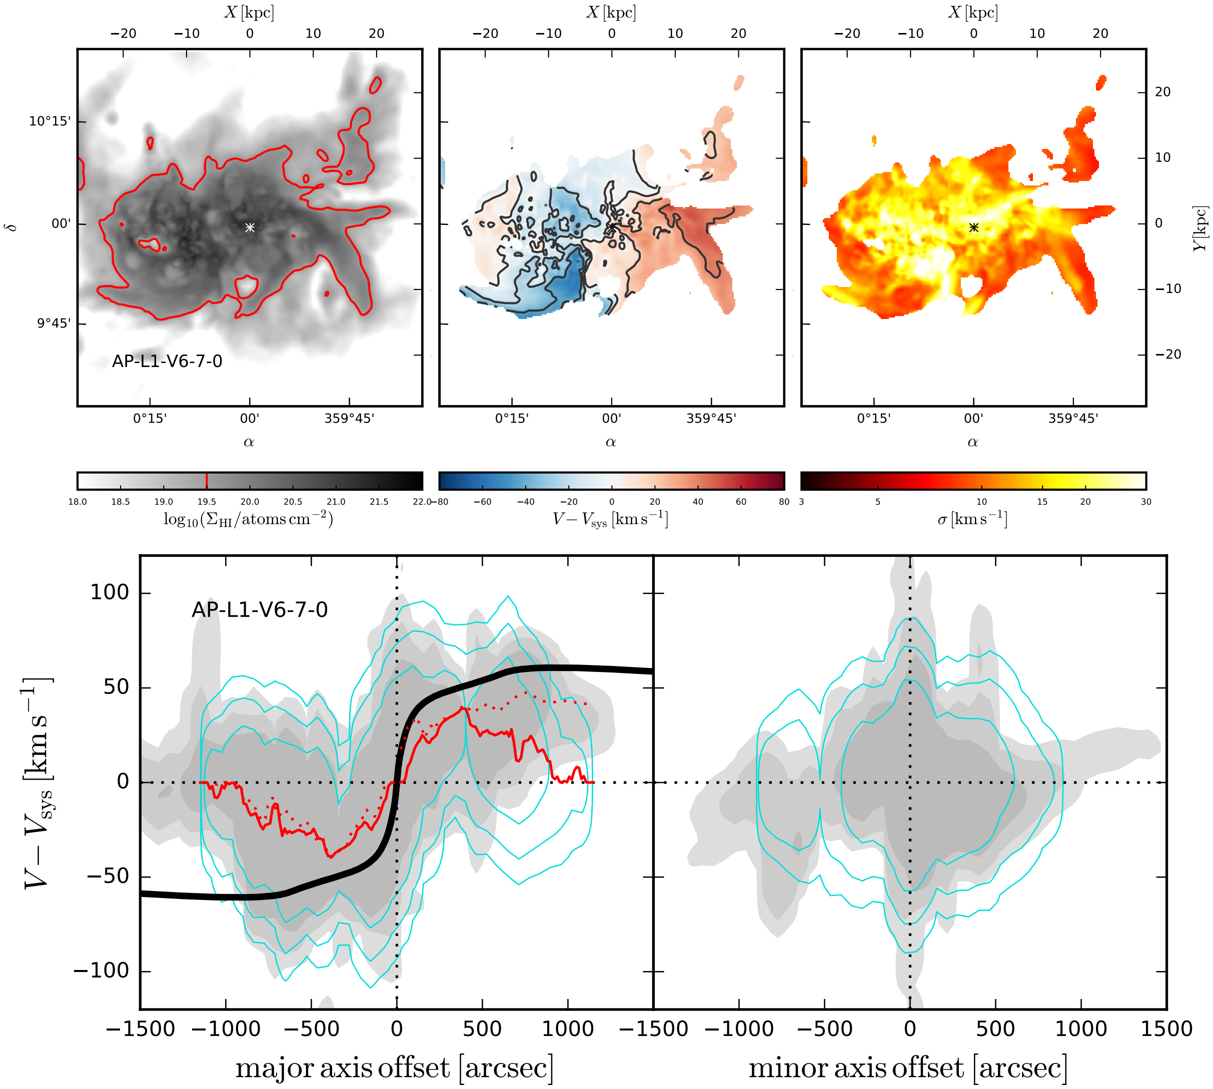


**Figure 12.** Moment maps, position-velocity diagrams and rotation curve fit summary (next page) for AP-L1-V6-7-0. See text for detailed description.

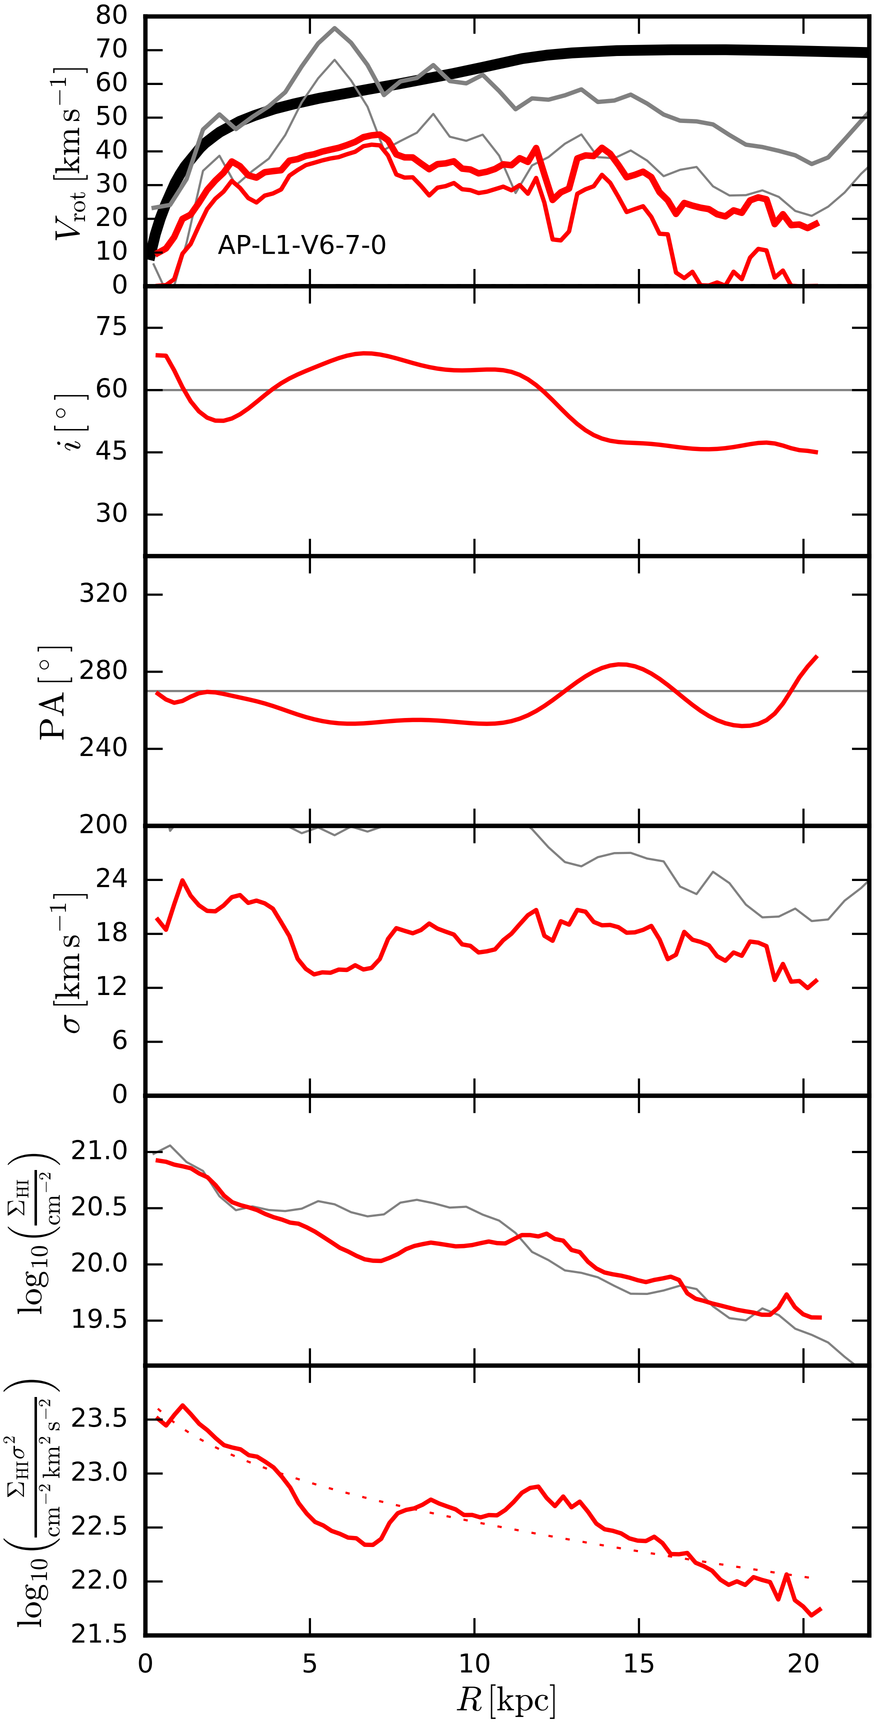


**Figure 12** – *continued*

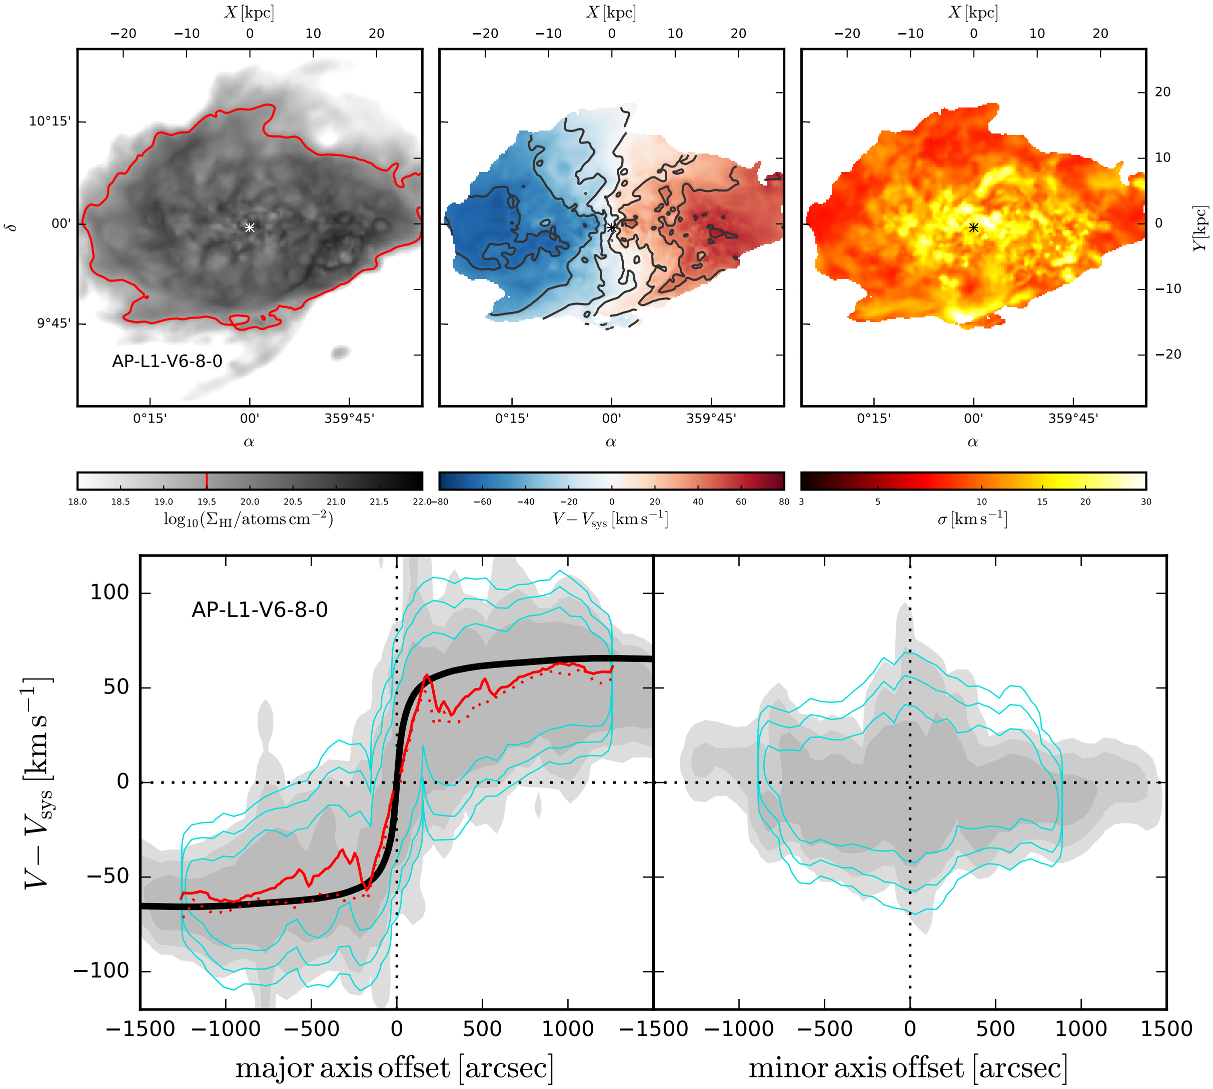


**Figure 13.** Moment maps, position-velocity diagrams and rotation curve fit summary (next page) for AP-L1-V6-8-0. See text for detailed description.

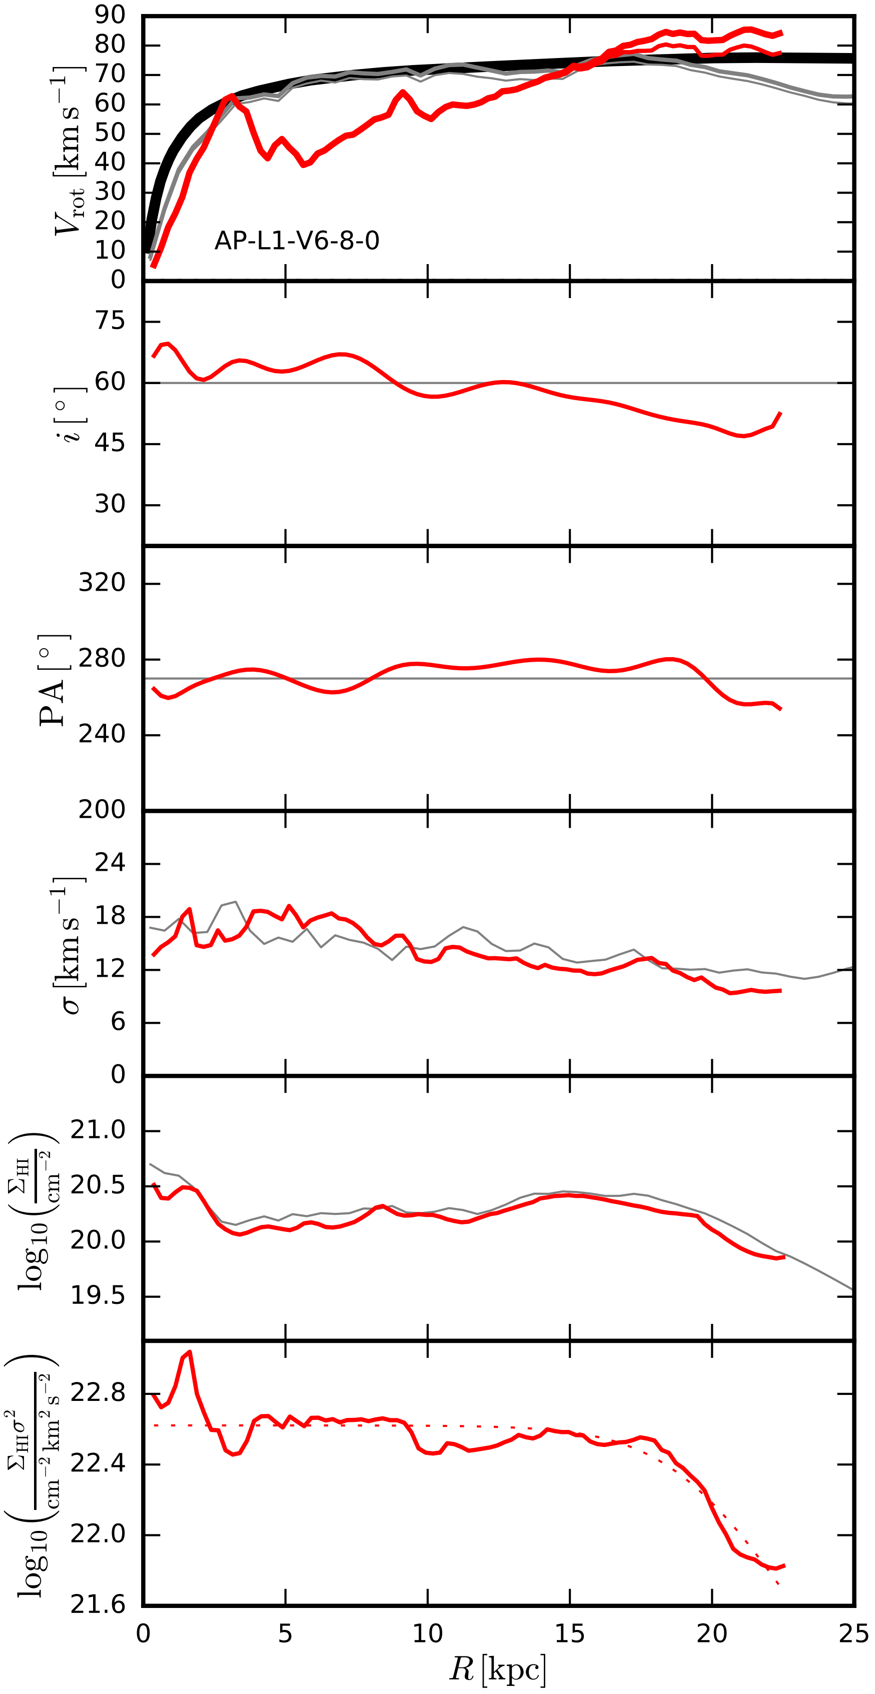


**Figure 13** – *continued*

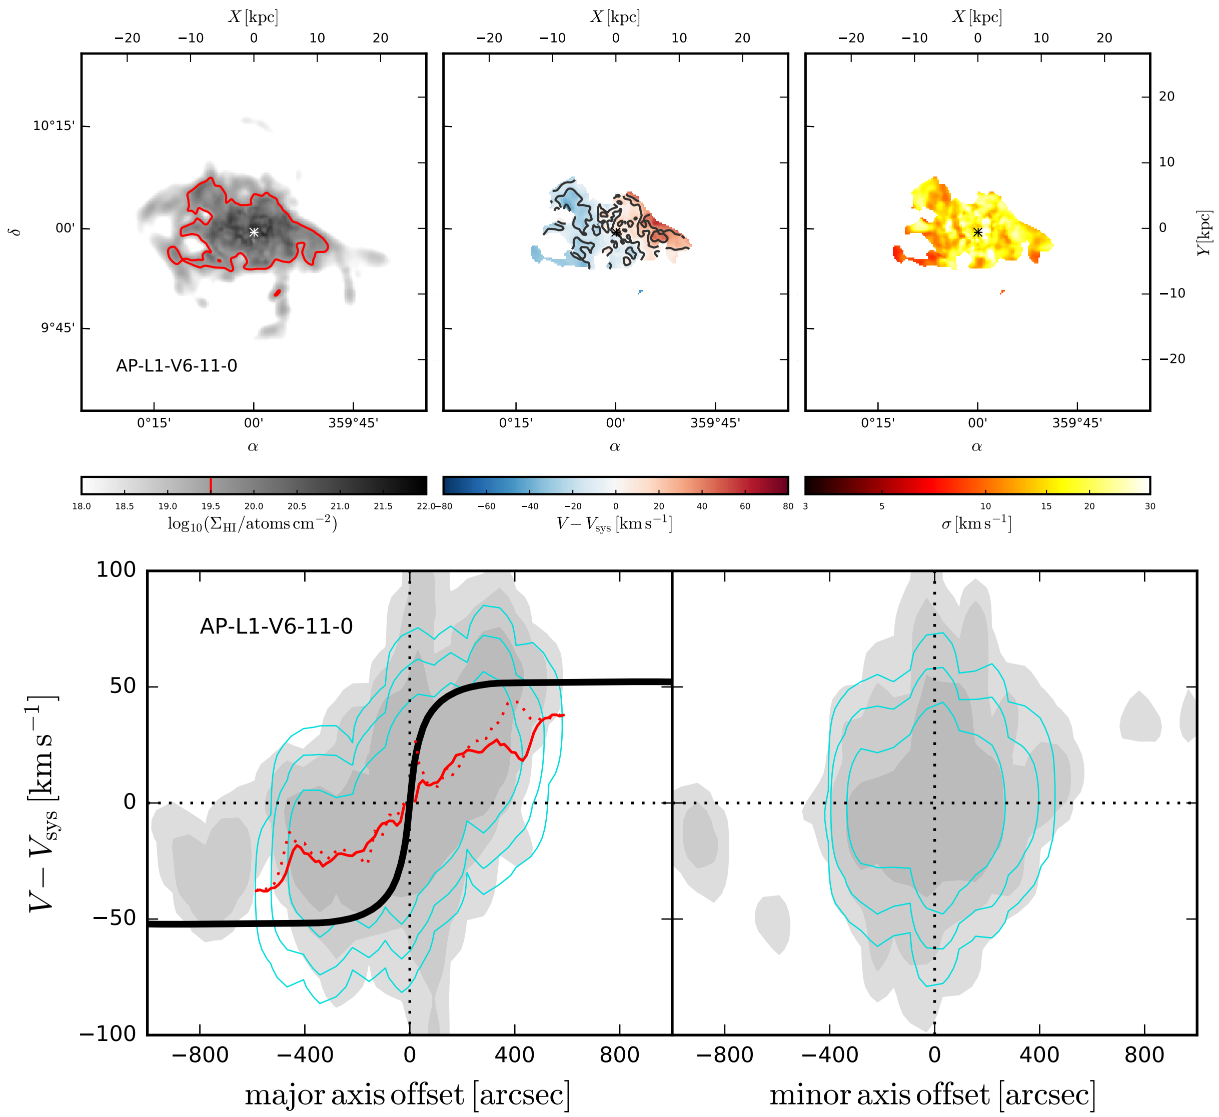


**Figure 14.** Moment maps, position-velocity diagrams and rotation curve fit summary (next page) for AP-L1-V6-11-0. See text for detailed description.

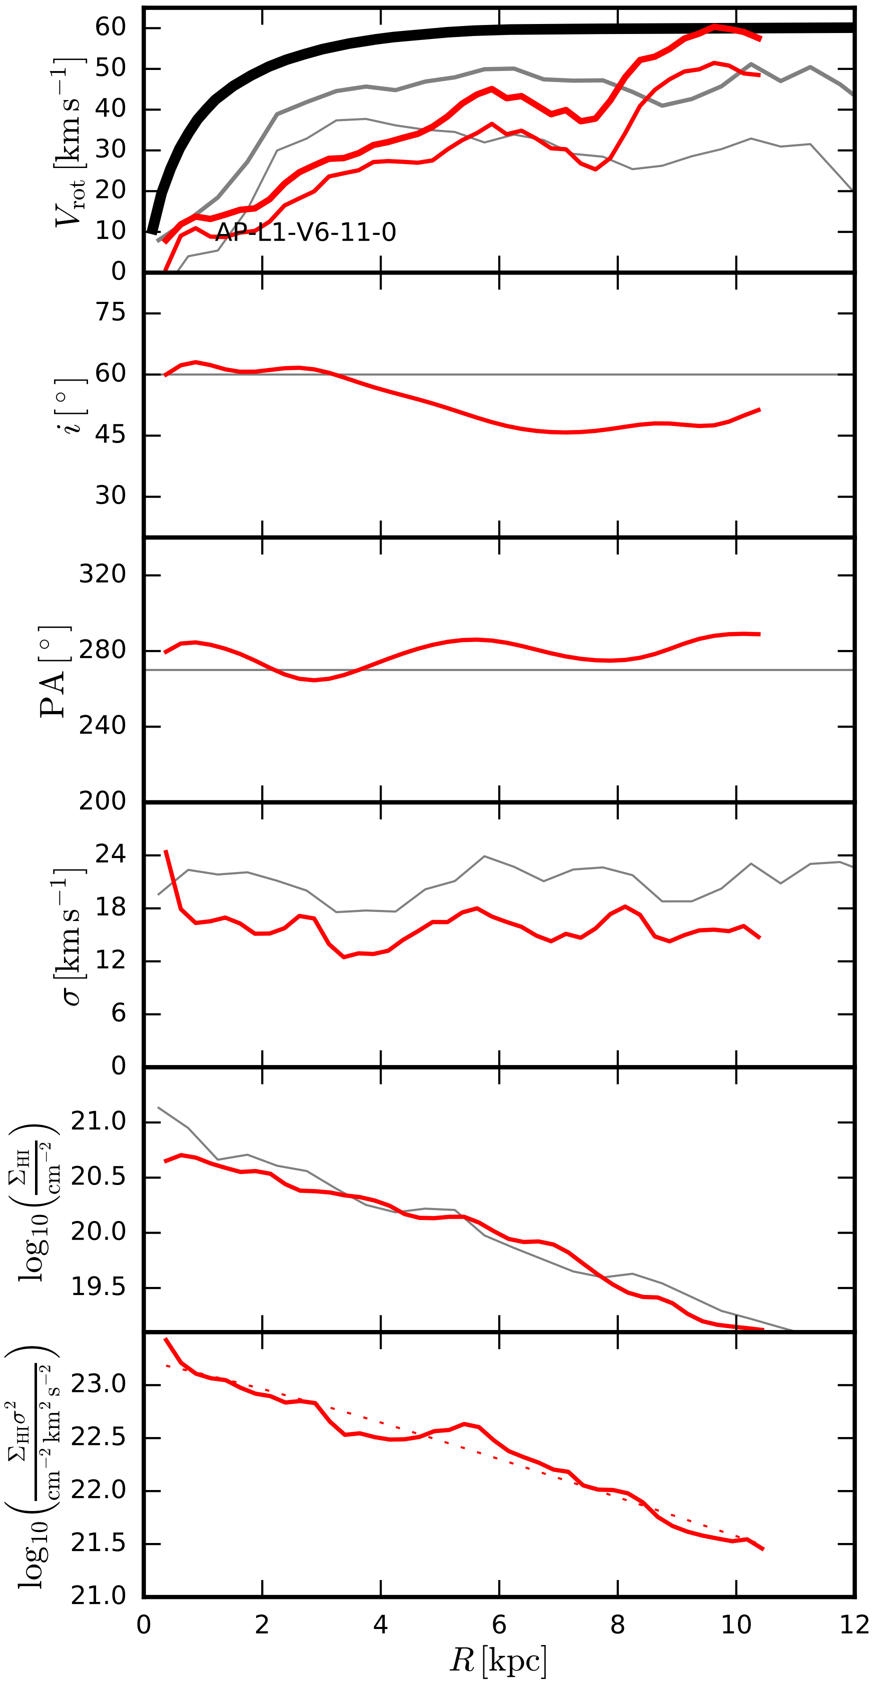


**Figure 14** – *continued*

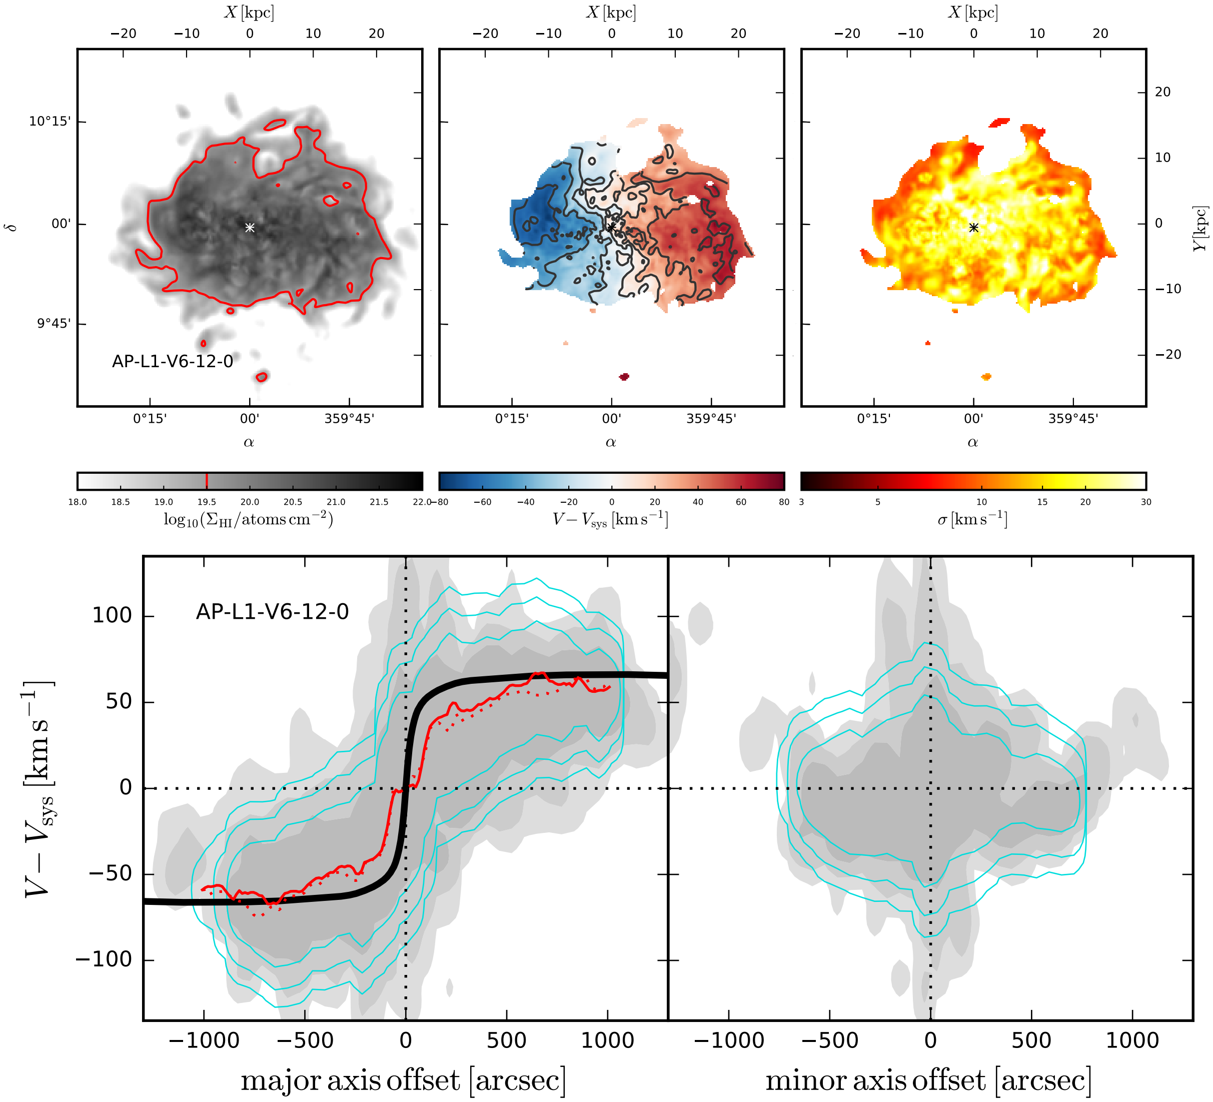


**Figure 15.** Moment maps, position-velocity diagrams and rotation curve fit summary (next page) for AP-L1-V6-12-0. See text for detailed description.

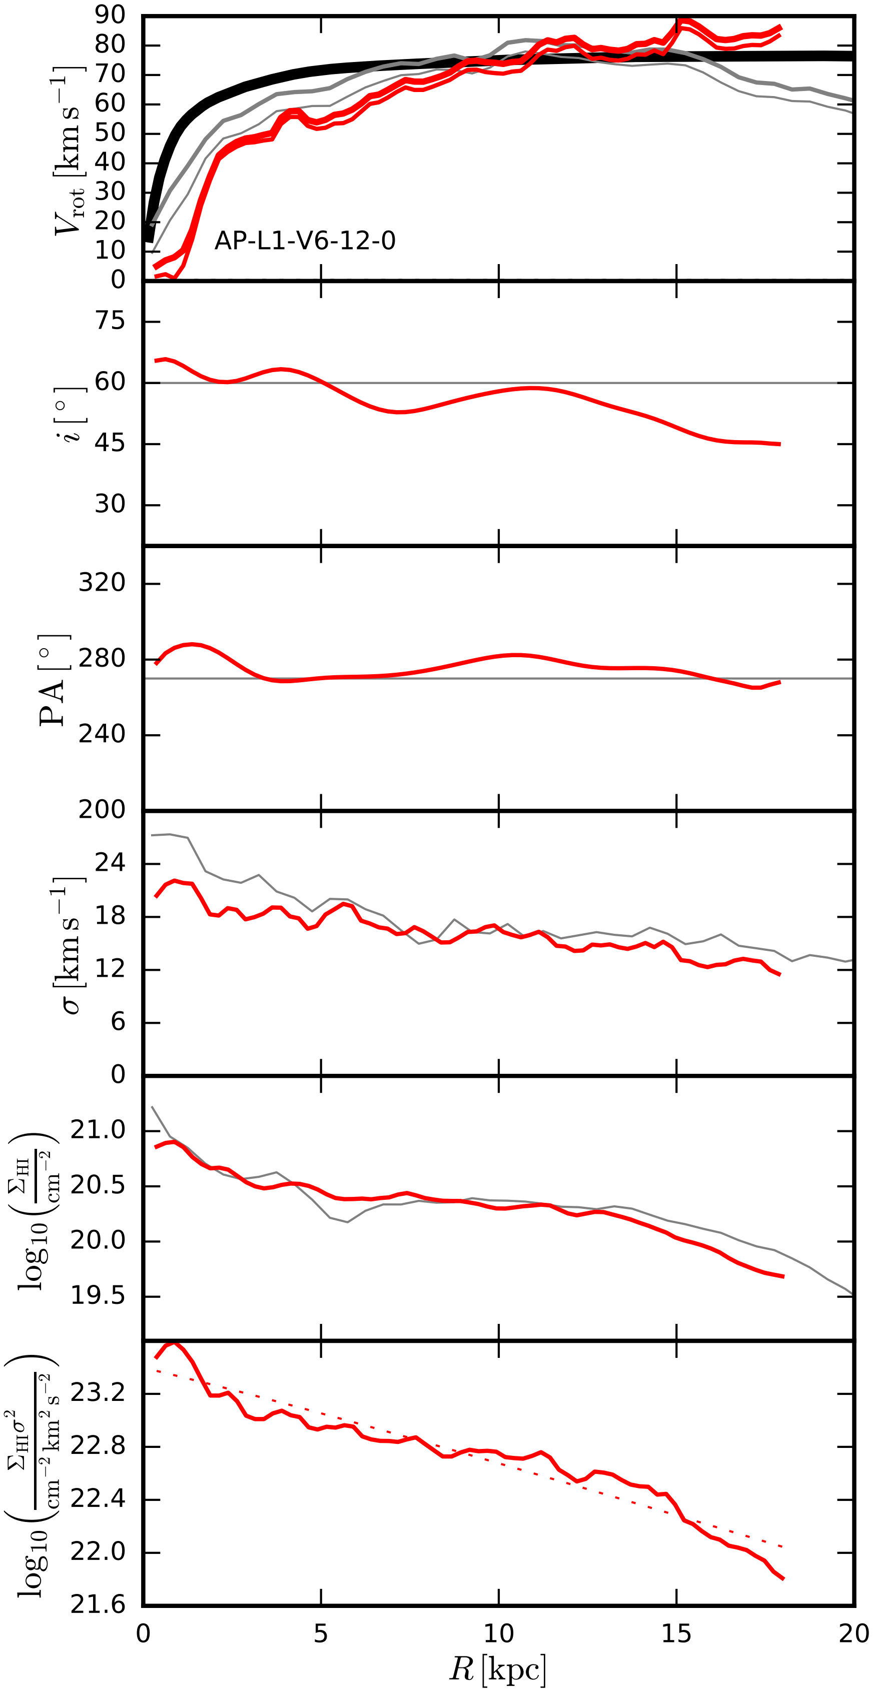


**Figure 15** – *continued*

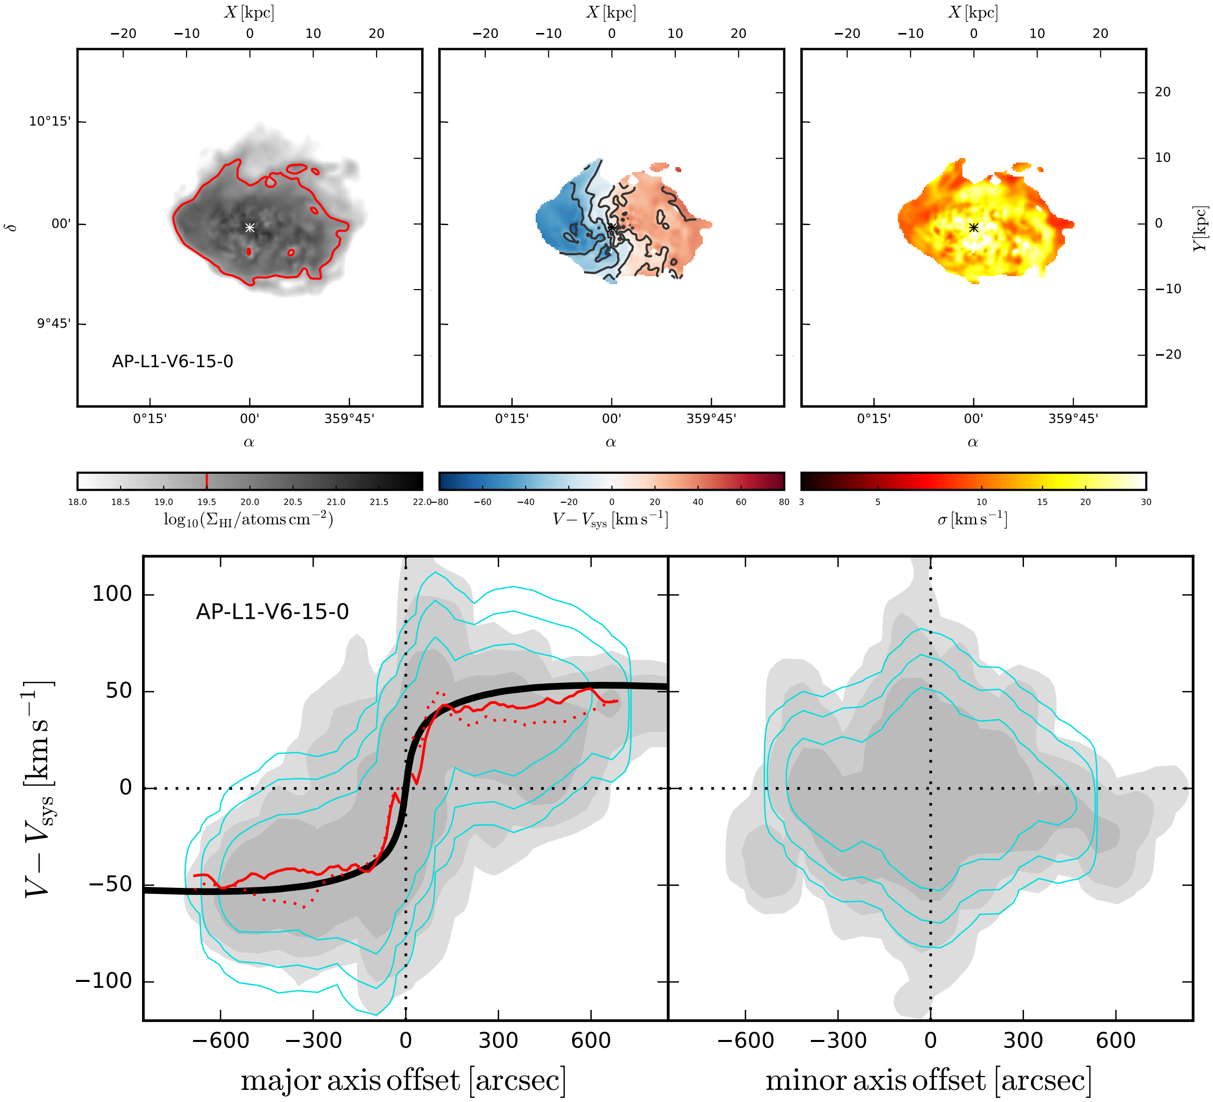


**Figure 16.** Moment maps, position-velocity diagrams and rotation curve fit summary (next page) for AP-L1-V6-15-0. See text for detailed description.

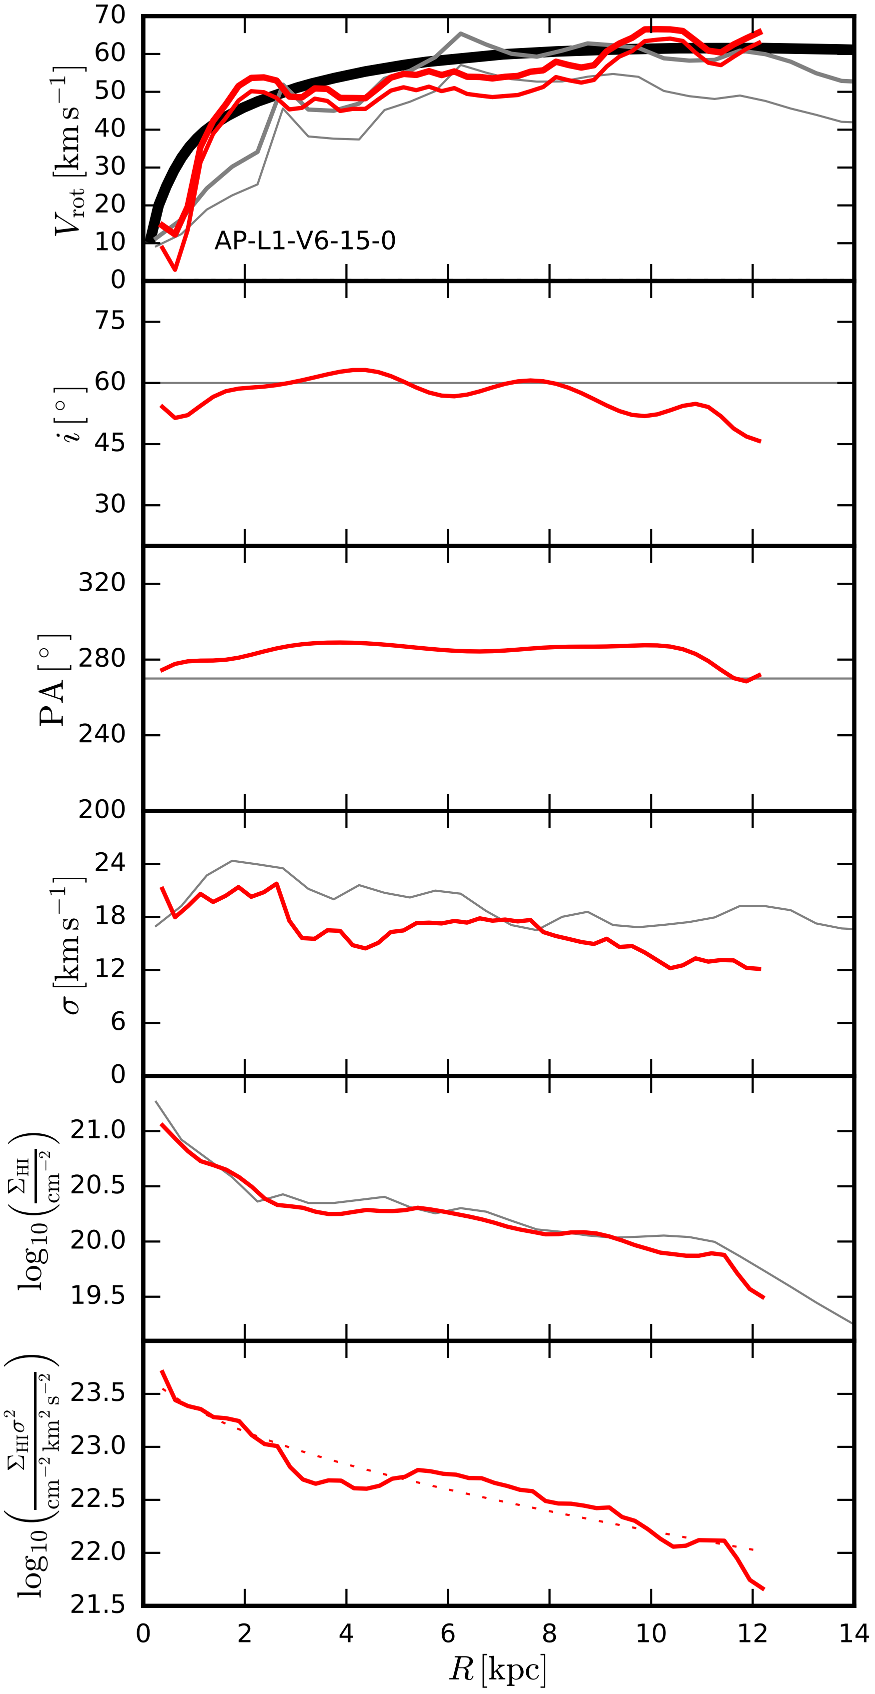


**Figure 16** – *continued*

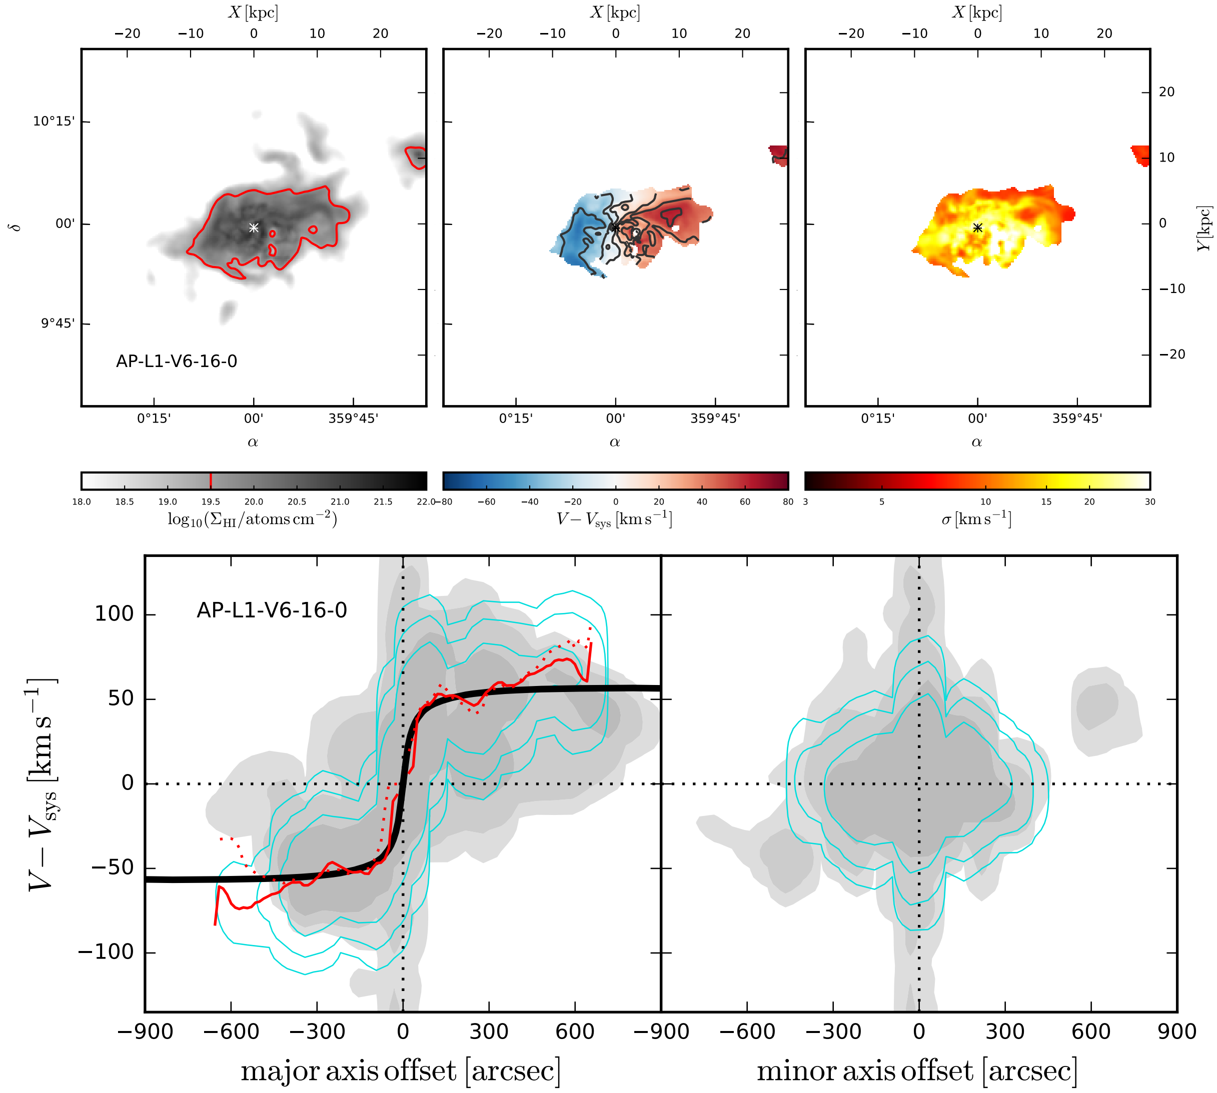


**Figure 17.** Moment maps, position-velocity diagrams and rotation curve fit summary (next page) for AP-L1-V6-16-0. See text for detailed description.

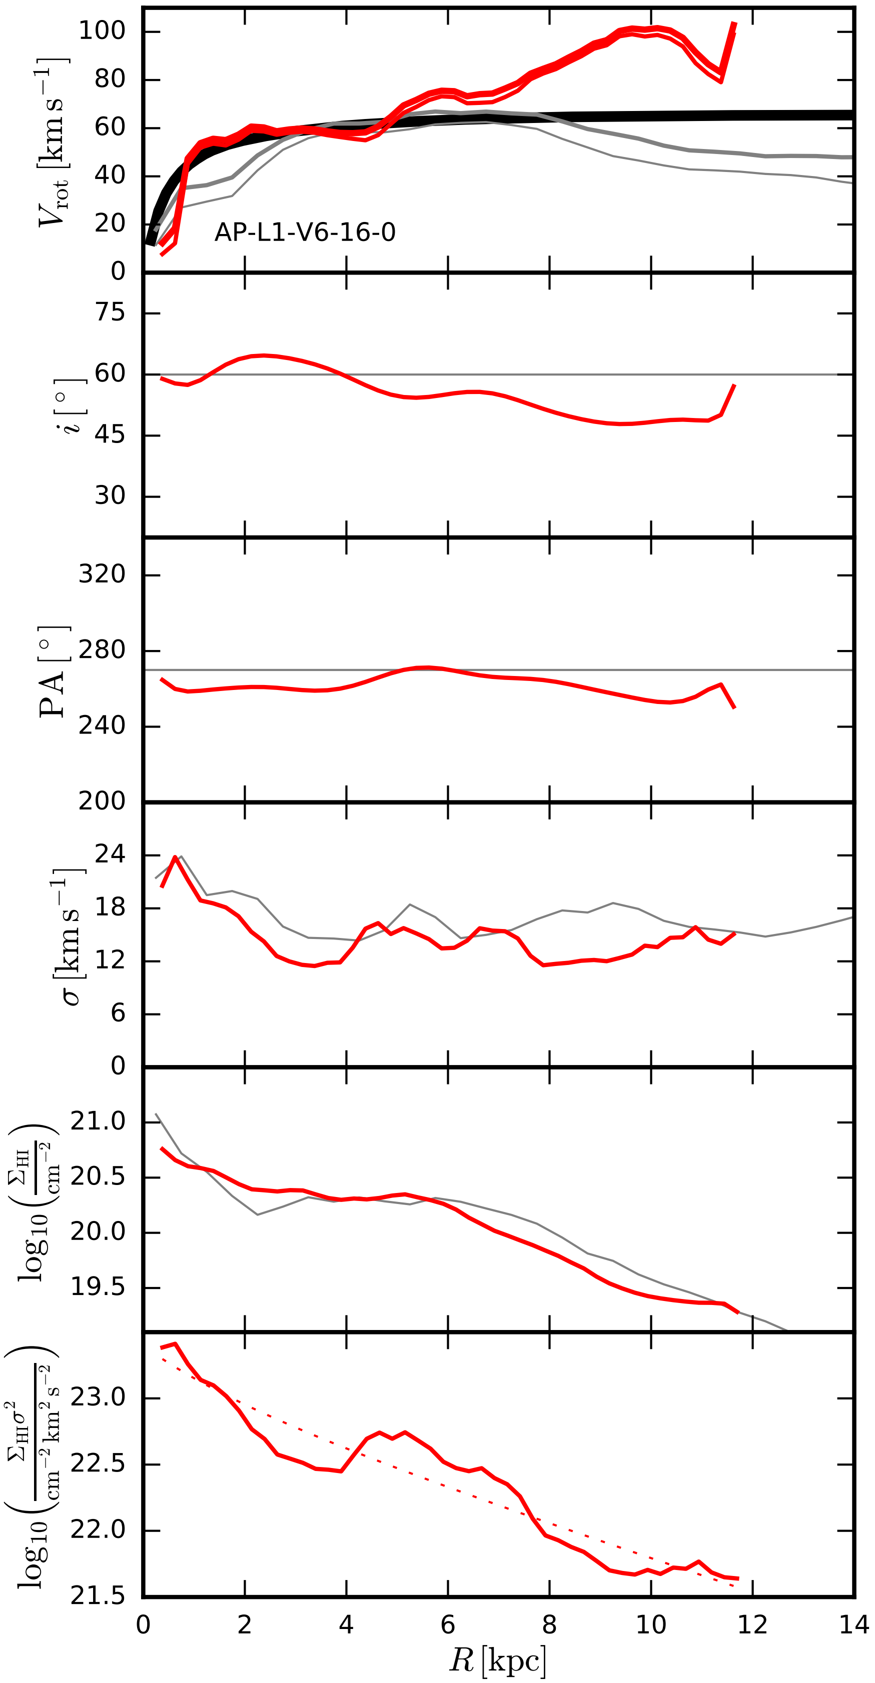


**Figure 17** – *continued*

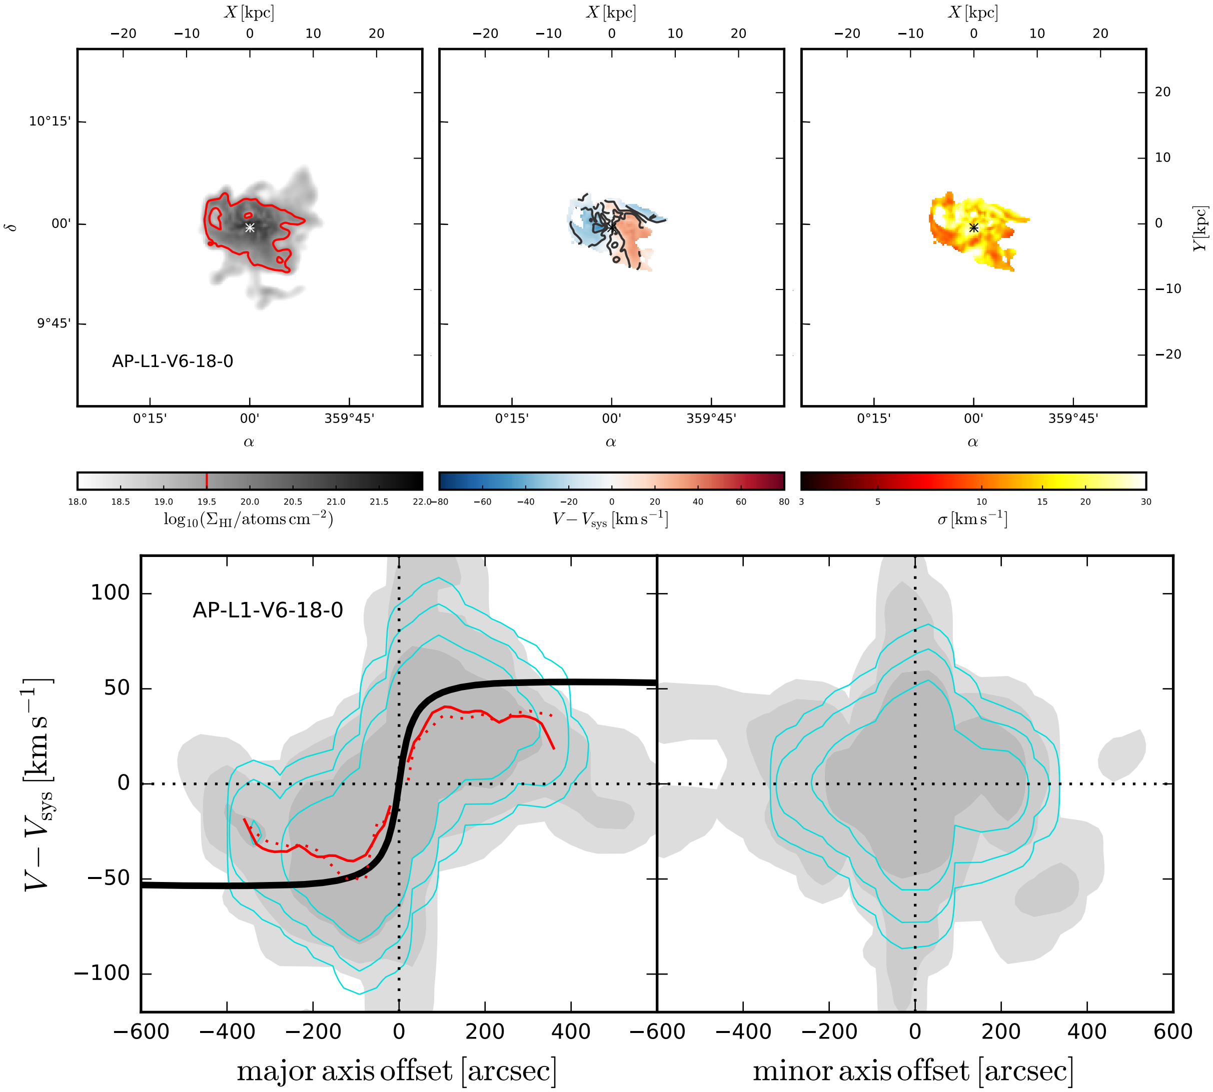


**Figure 18.** Moment maps, position-velocity diagrams and rotation curve fit summary (next page) for AP-L1-V6-18-0. See text for detailed description.

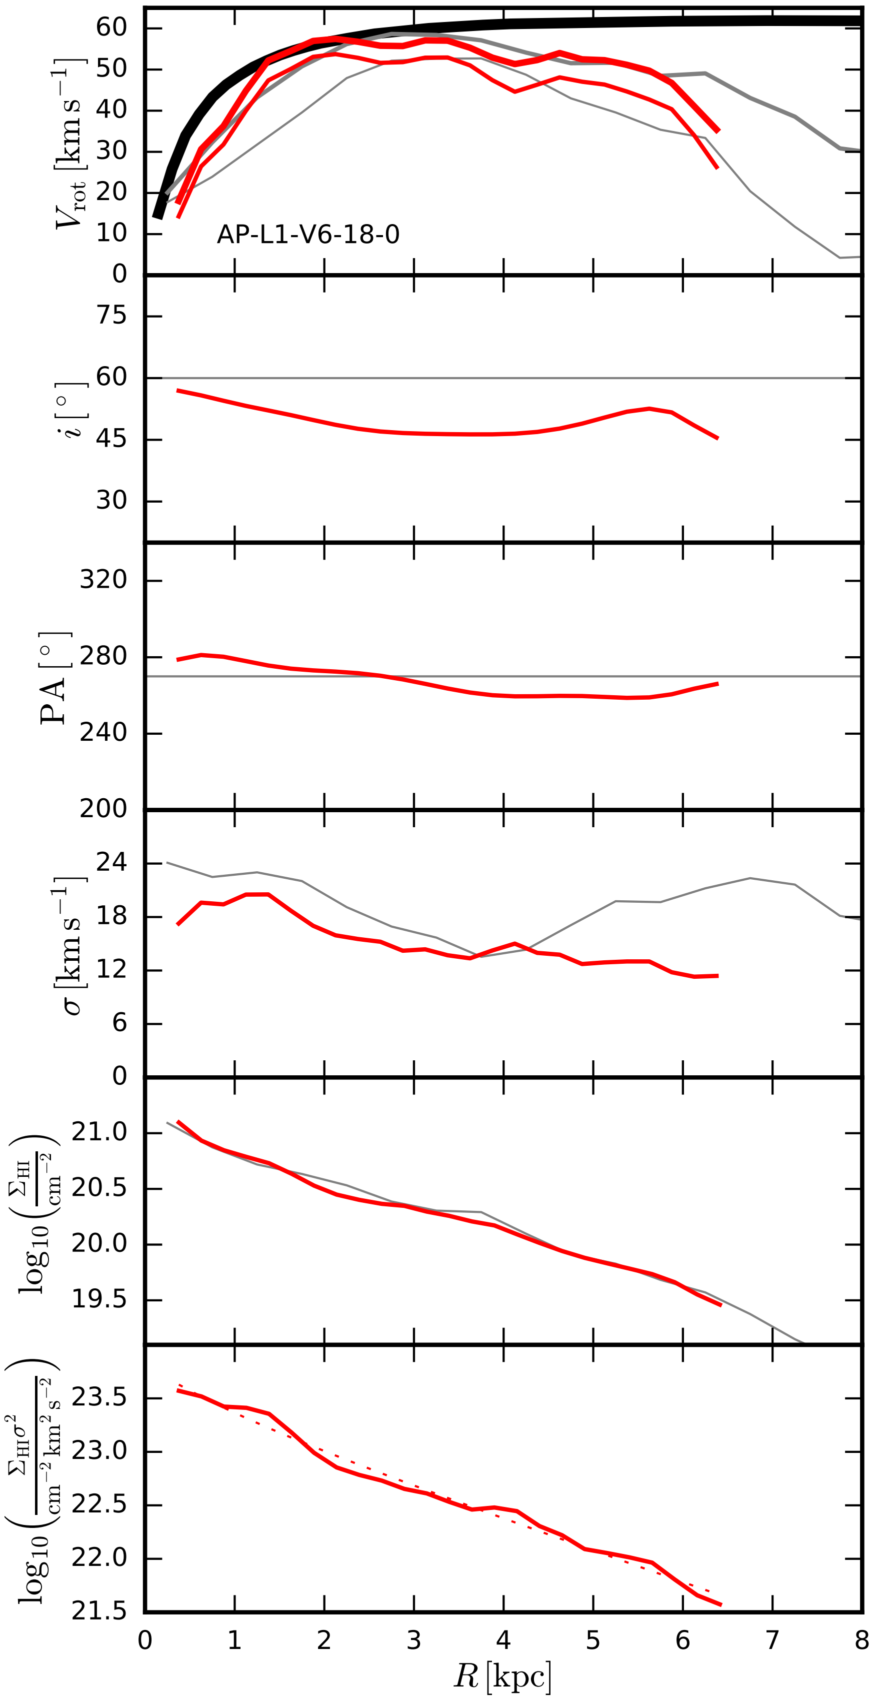


**Figure 18** – *continued*

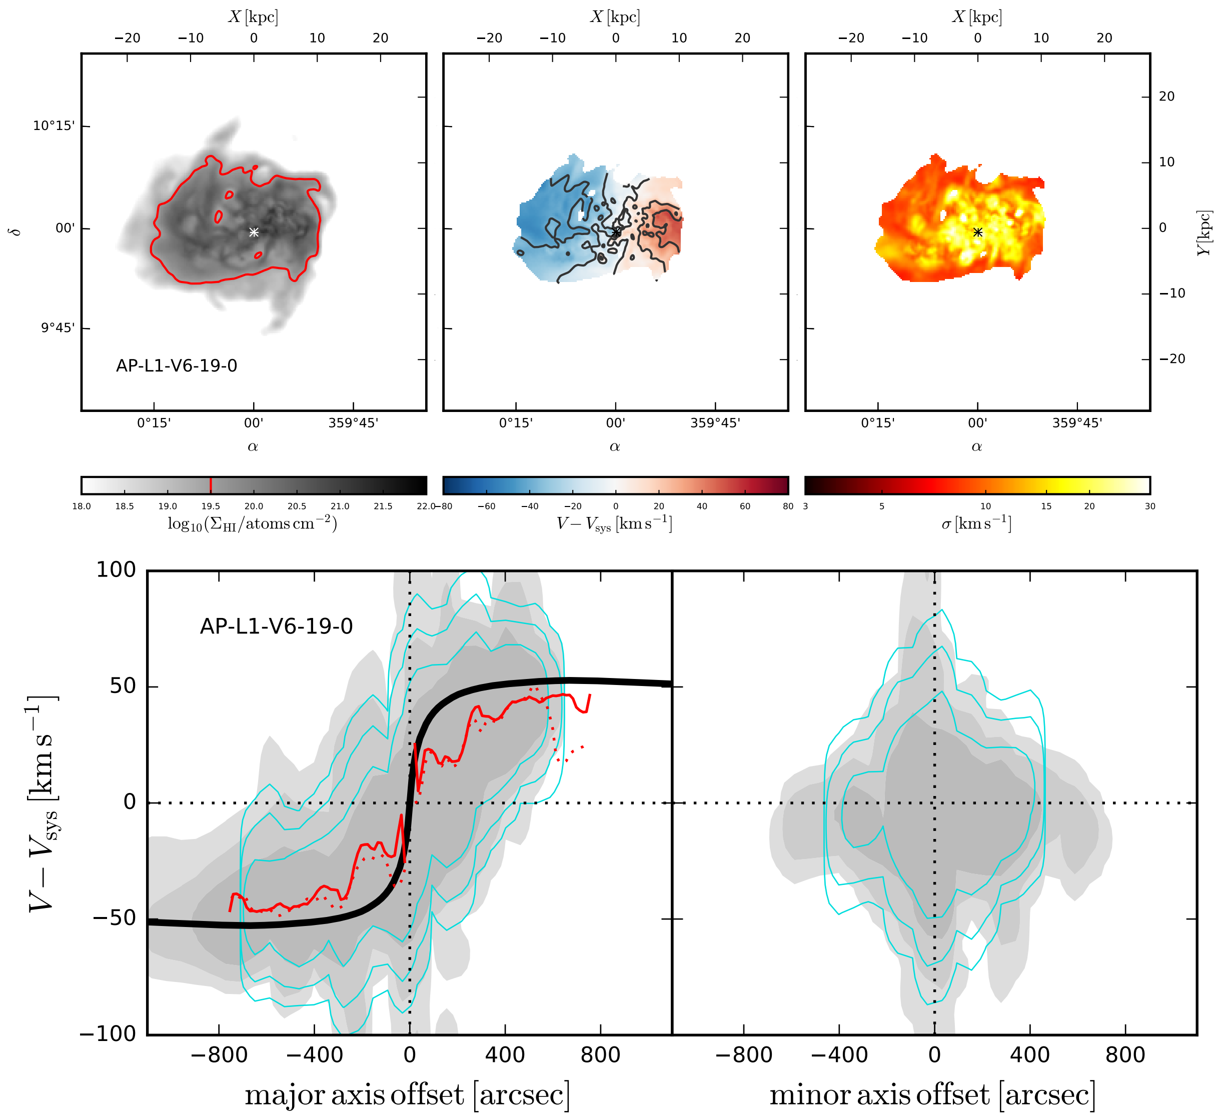


**Figure 19.** Moment maps, position-velocity diagrams and rotation curve fit summary (next page) for AP-L1-V6-19-0. See text for detailed description.

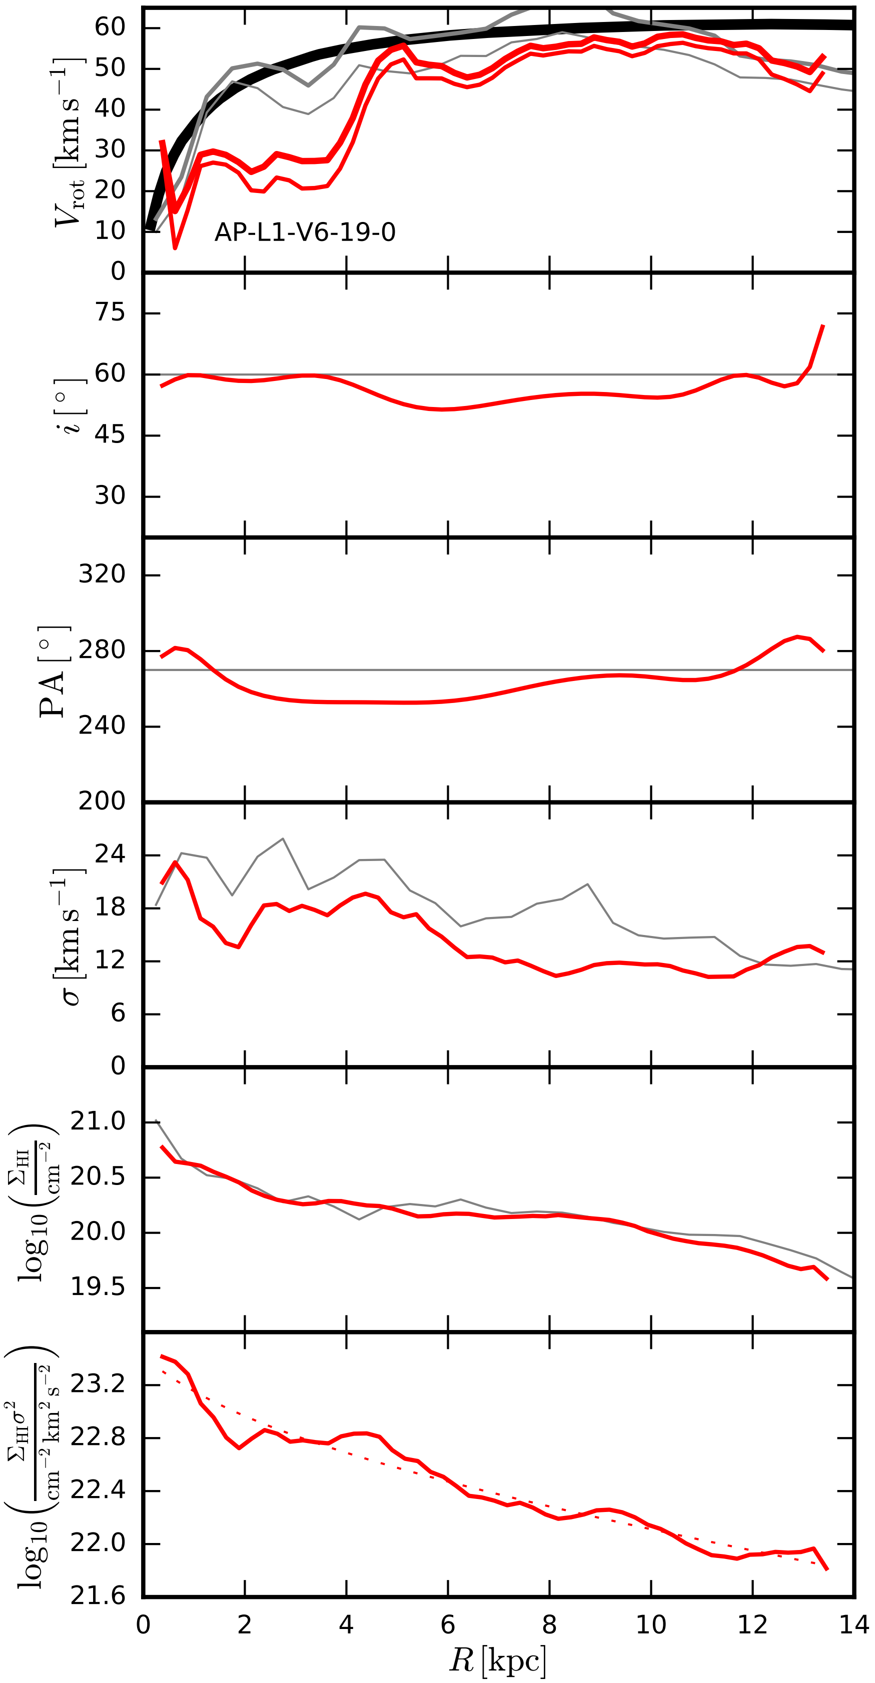


**Figure 19** – *continued*

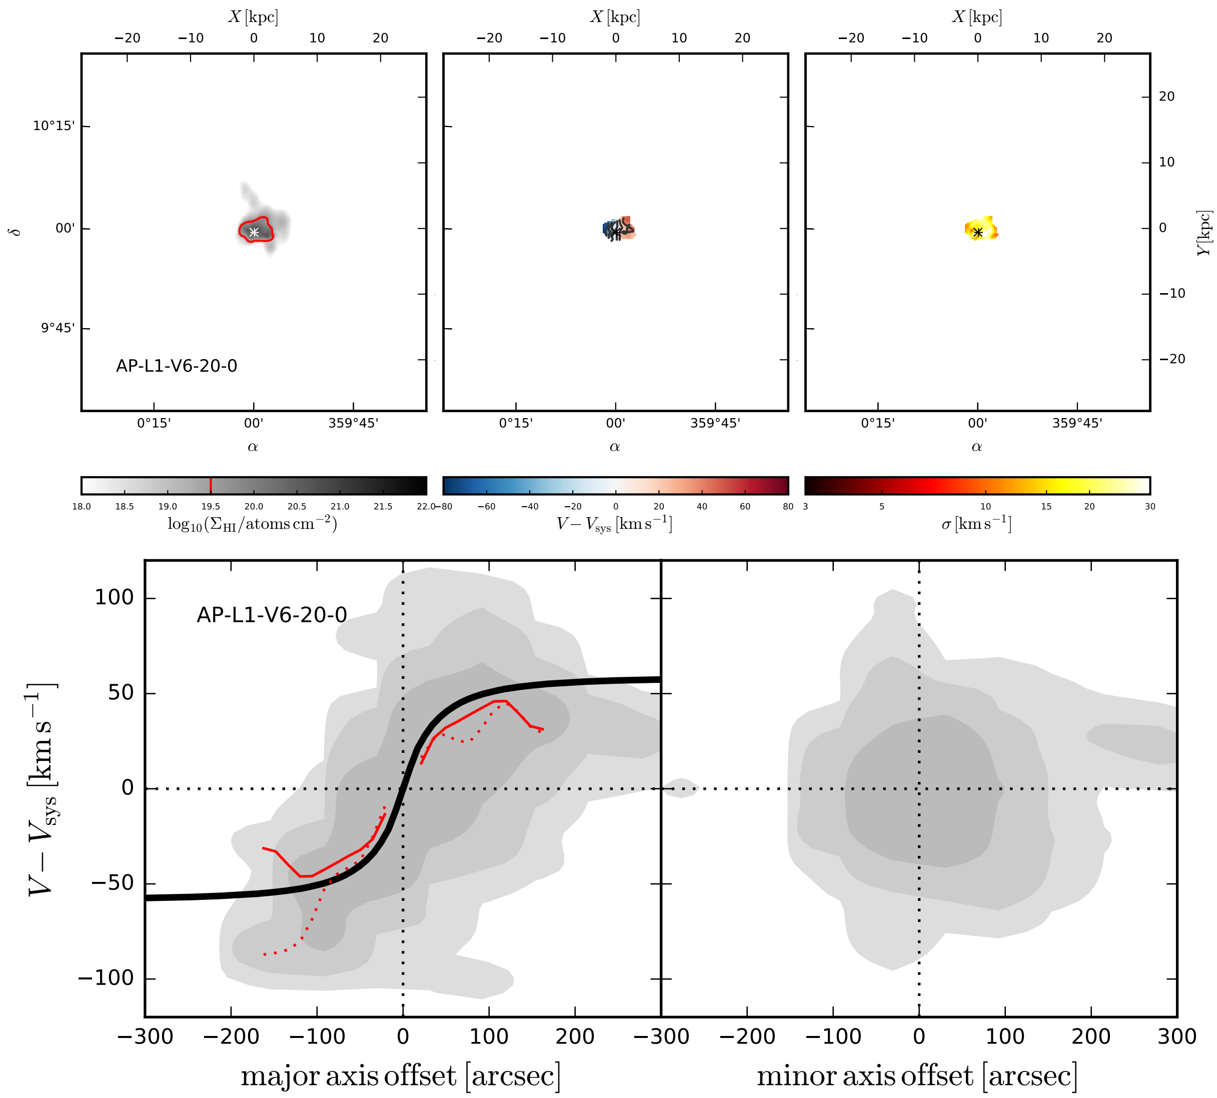


**Figure 20.** Moment maps, position-velocity diagrams and rotation curve fit summary (next page) for AP-L1-V6-20-0. See text for detailed description.

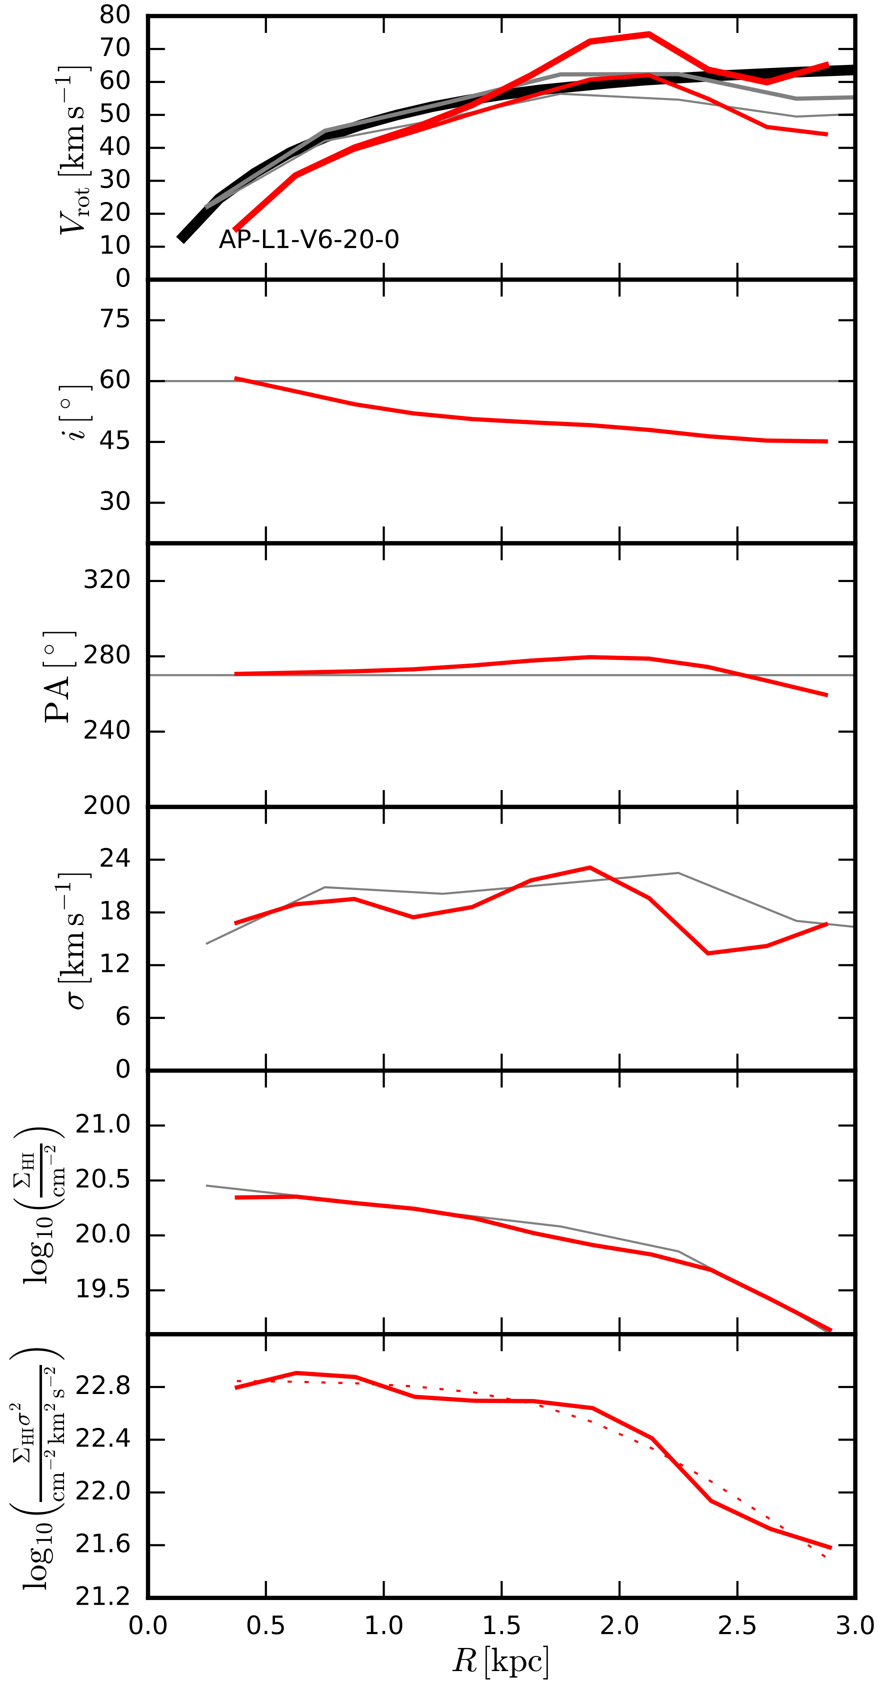


**Figure 20** – *continued*

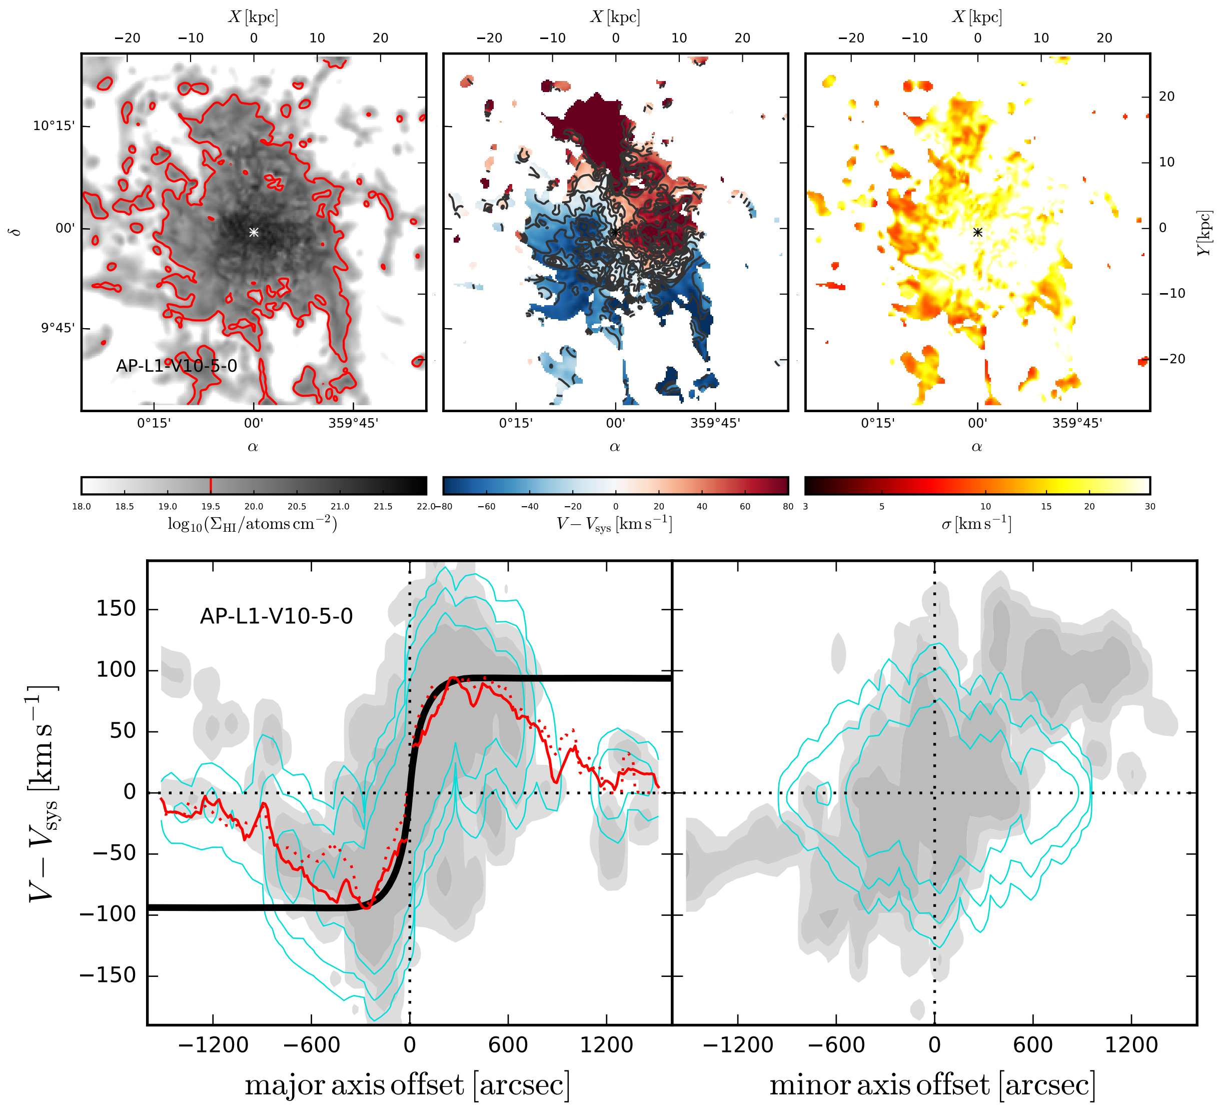


**Figure 21.** Moment maps, position-velocity diagrams and rotation curve fit summary (next page) for AP-L1-V10-5-0. See text for detailed description.

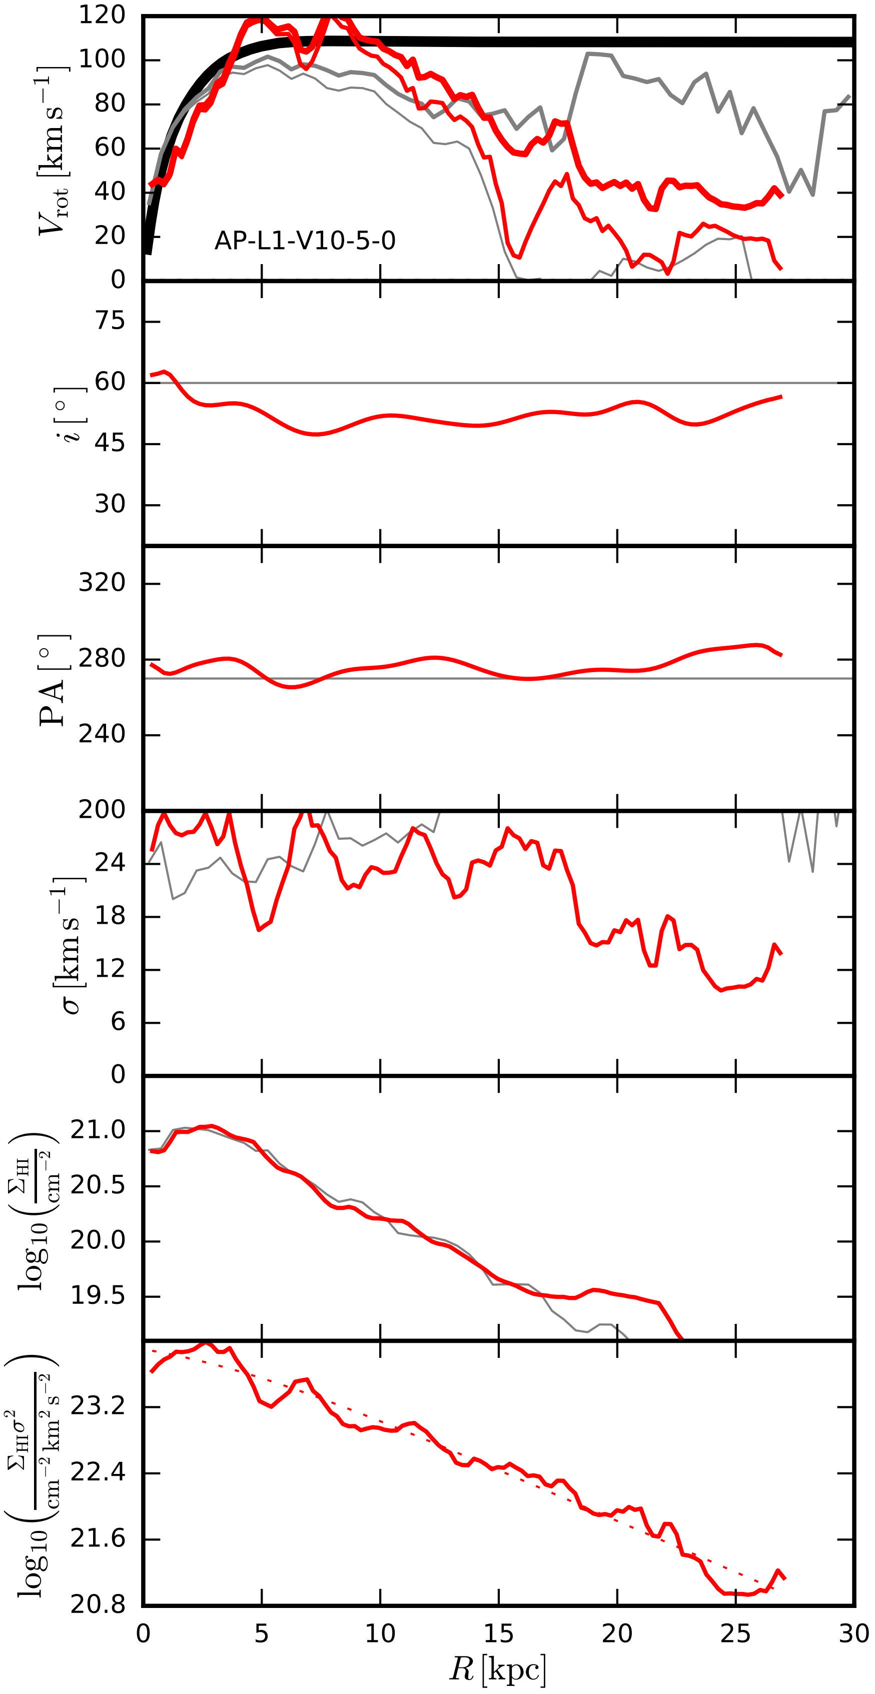


**Figure 21** – *continued*

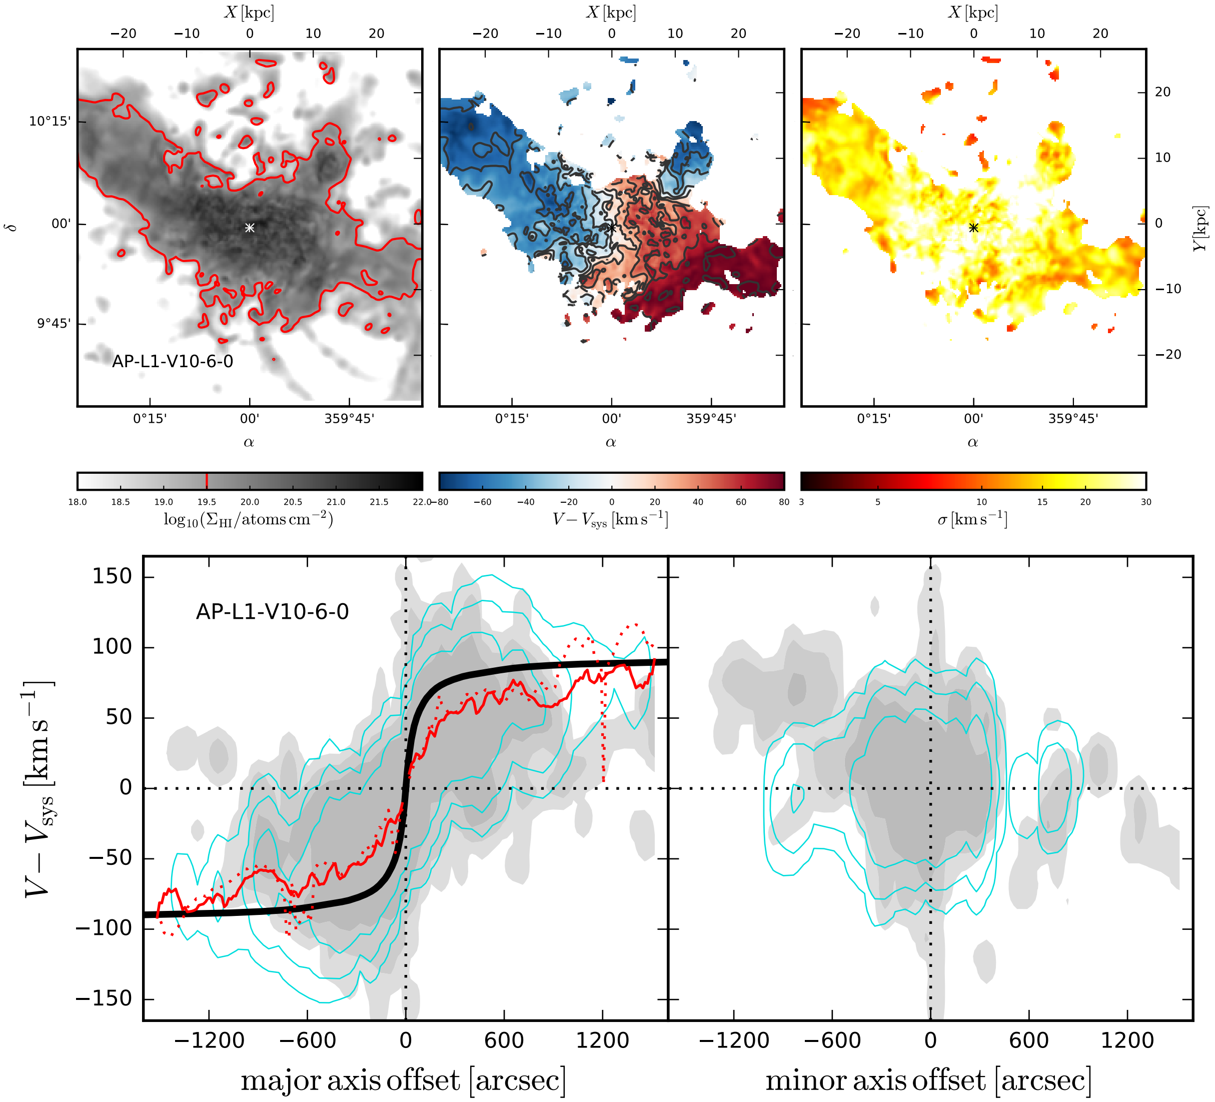


**Figure 22.** Moment maps, position-velocity diagrams and rotation curve fit summary (next page) for AP-L1-V10-5-0. See text for detailed description.

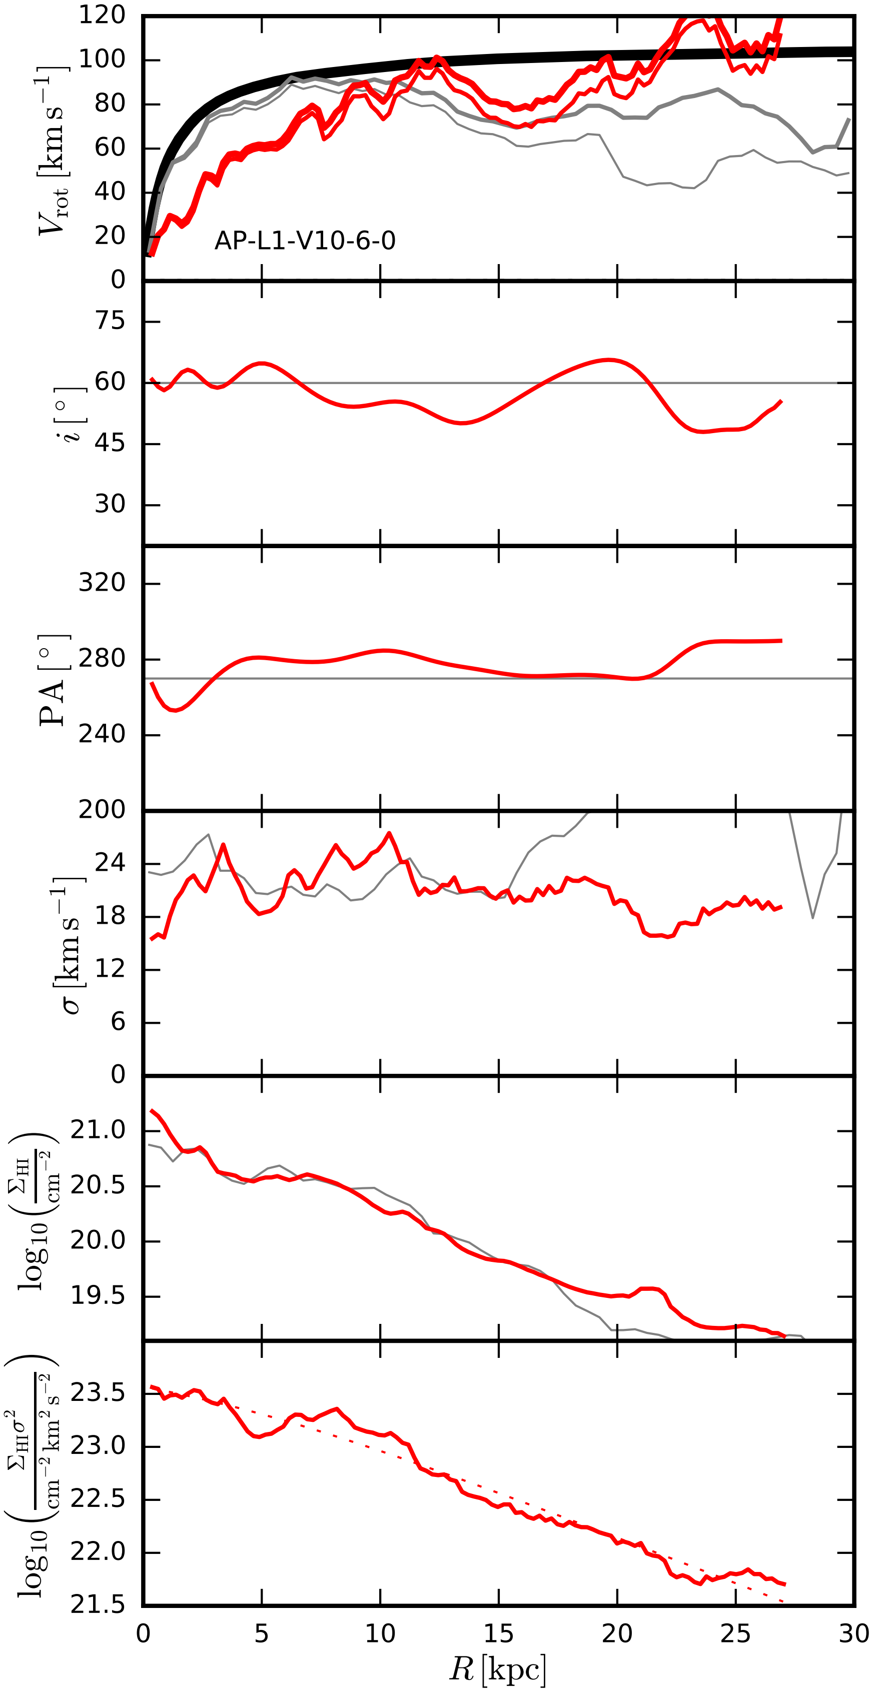


**Figure 22** – *continued*

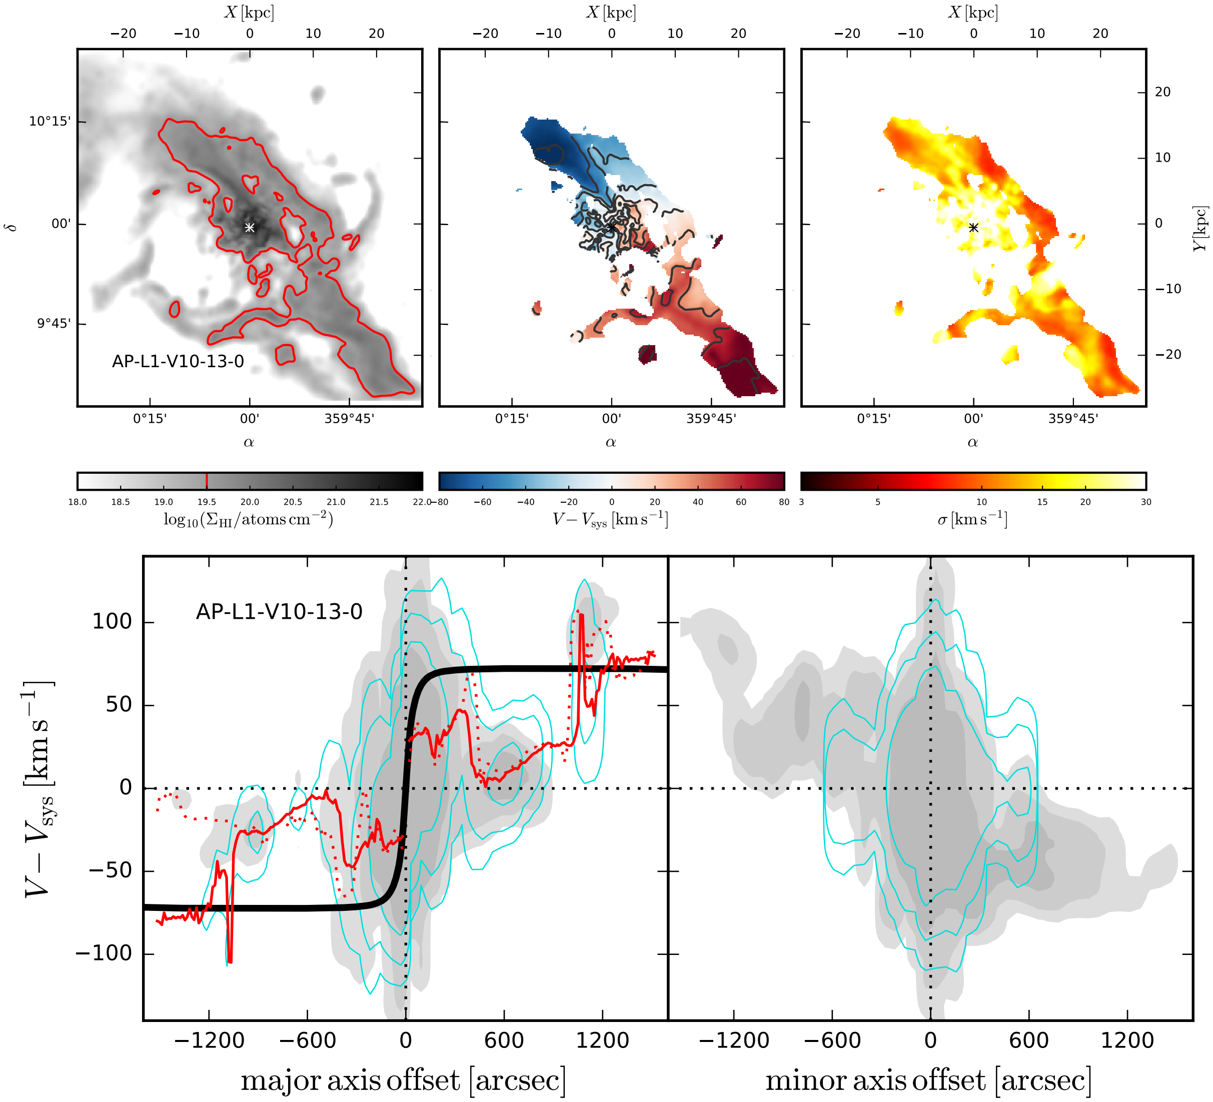


**Figure 23.** Moment maps, position-velocity diagrams and rotation curve fit summary (next page) for AP-L1-V10-13-0. See text for detailed description.

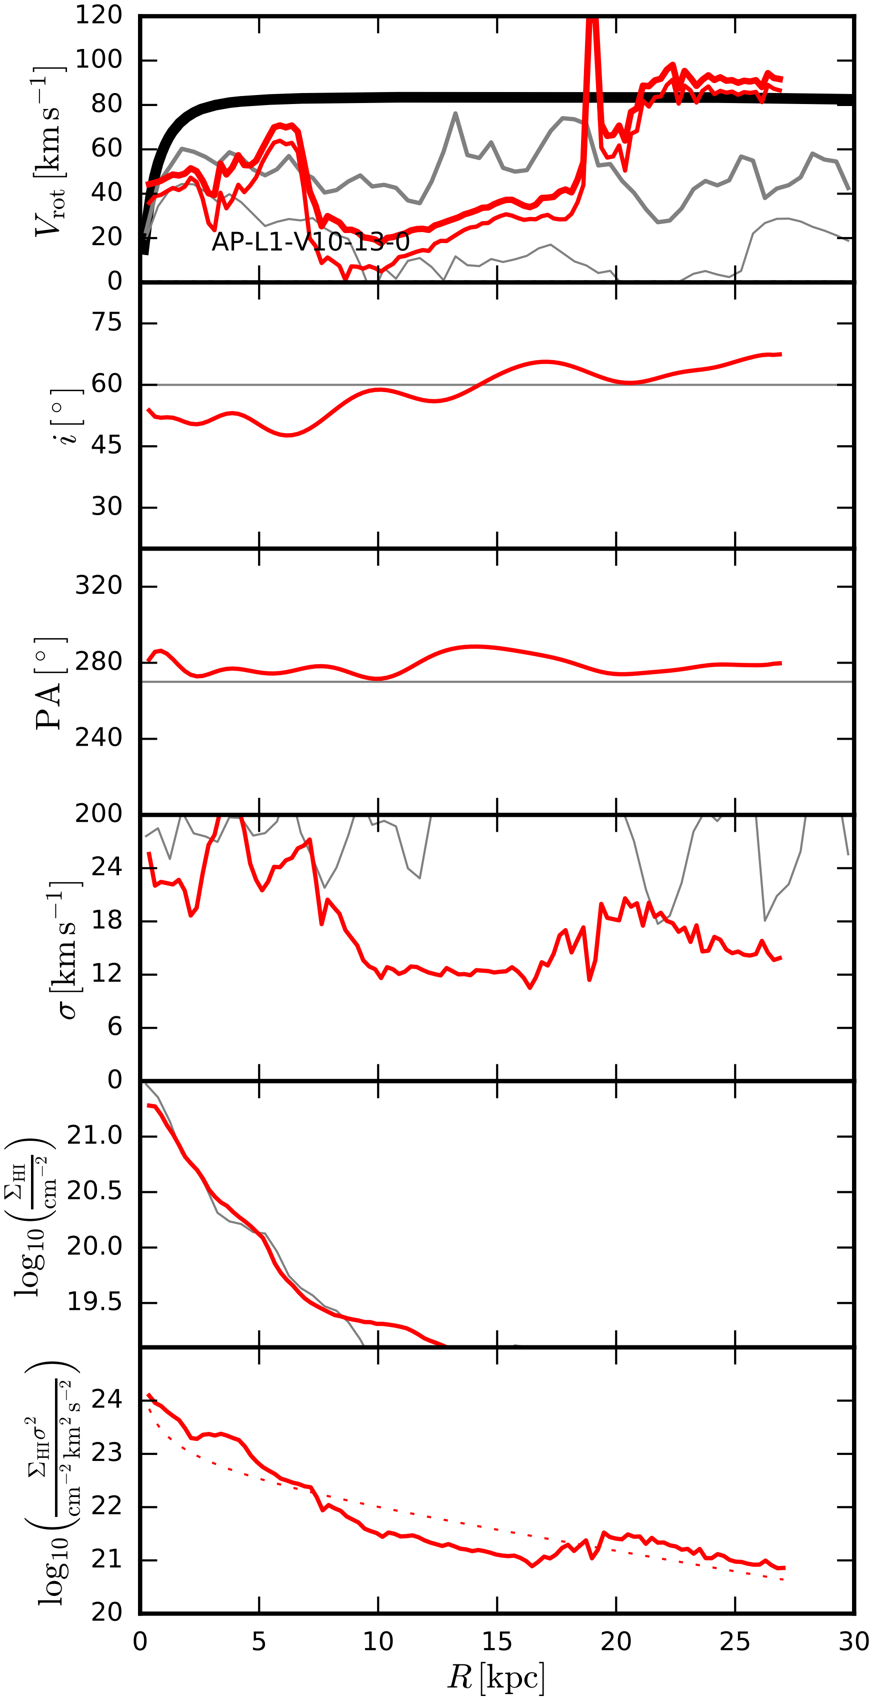


**Figure 23** – *continued*

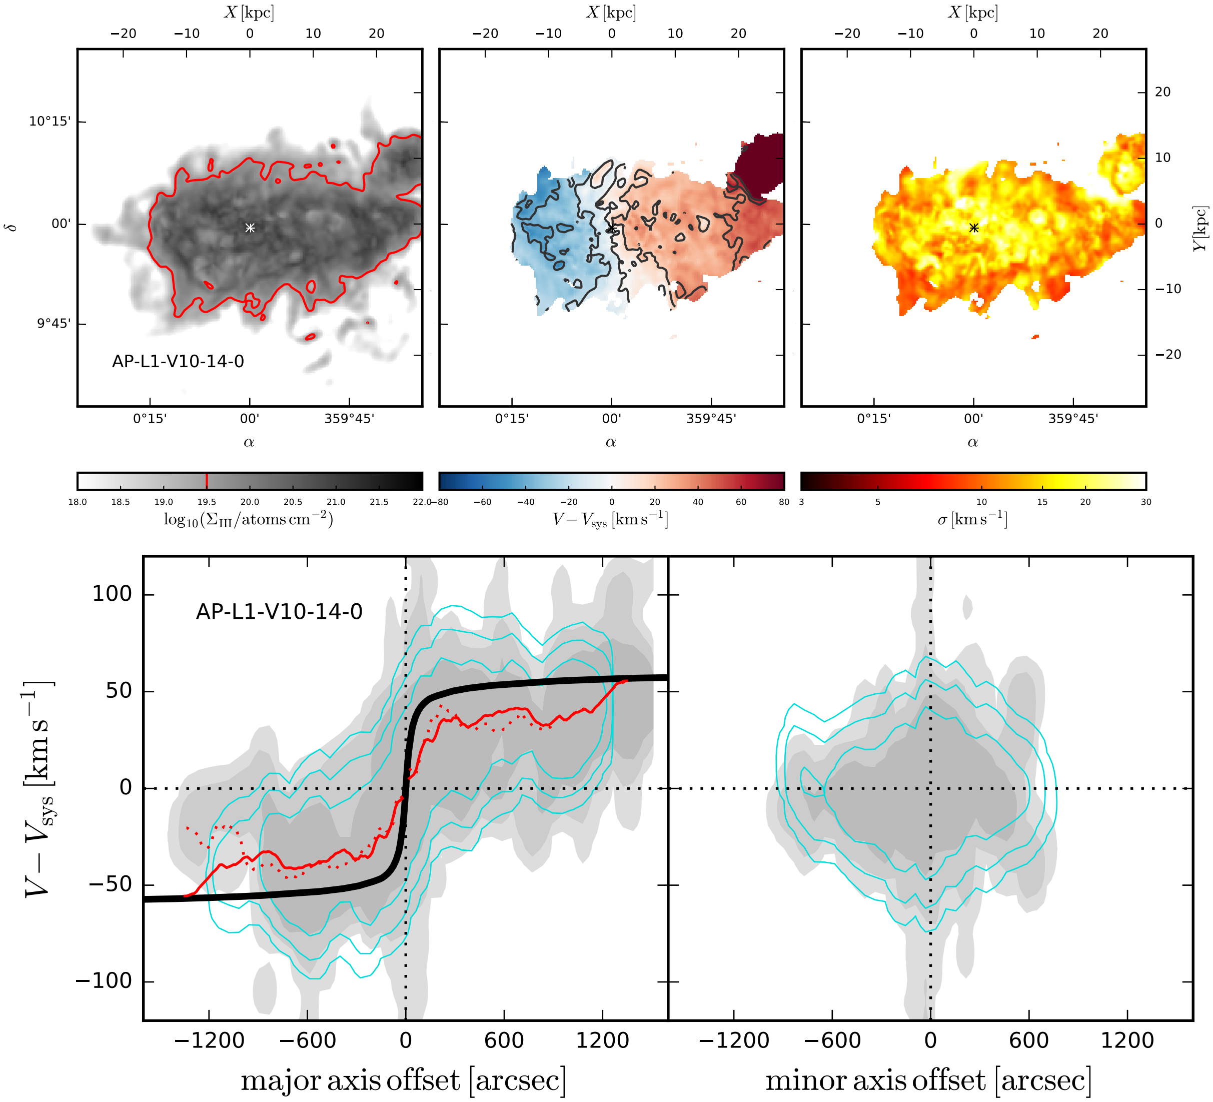


**Figure 24.** Moment maps, position-velocity diagrams and rotation curve fit summary (next page) for AP-L1-V10-14-0. See text for detailed description.

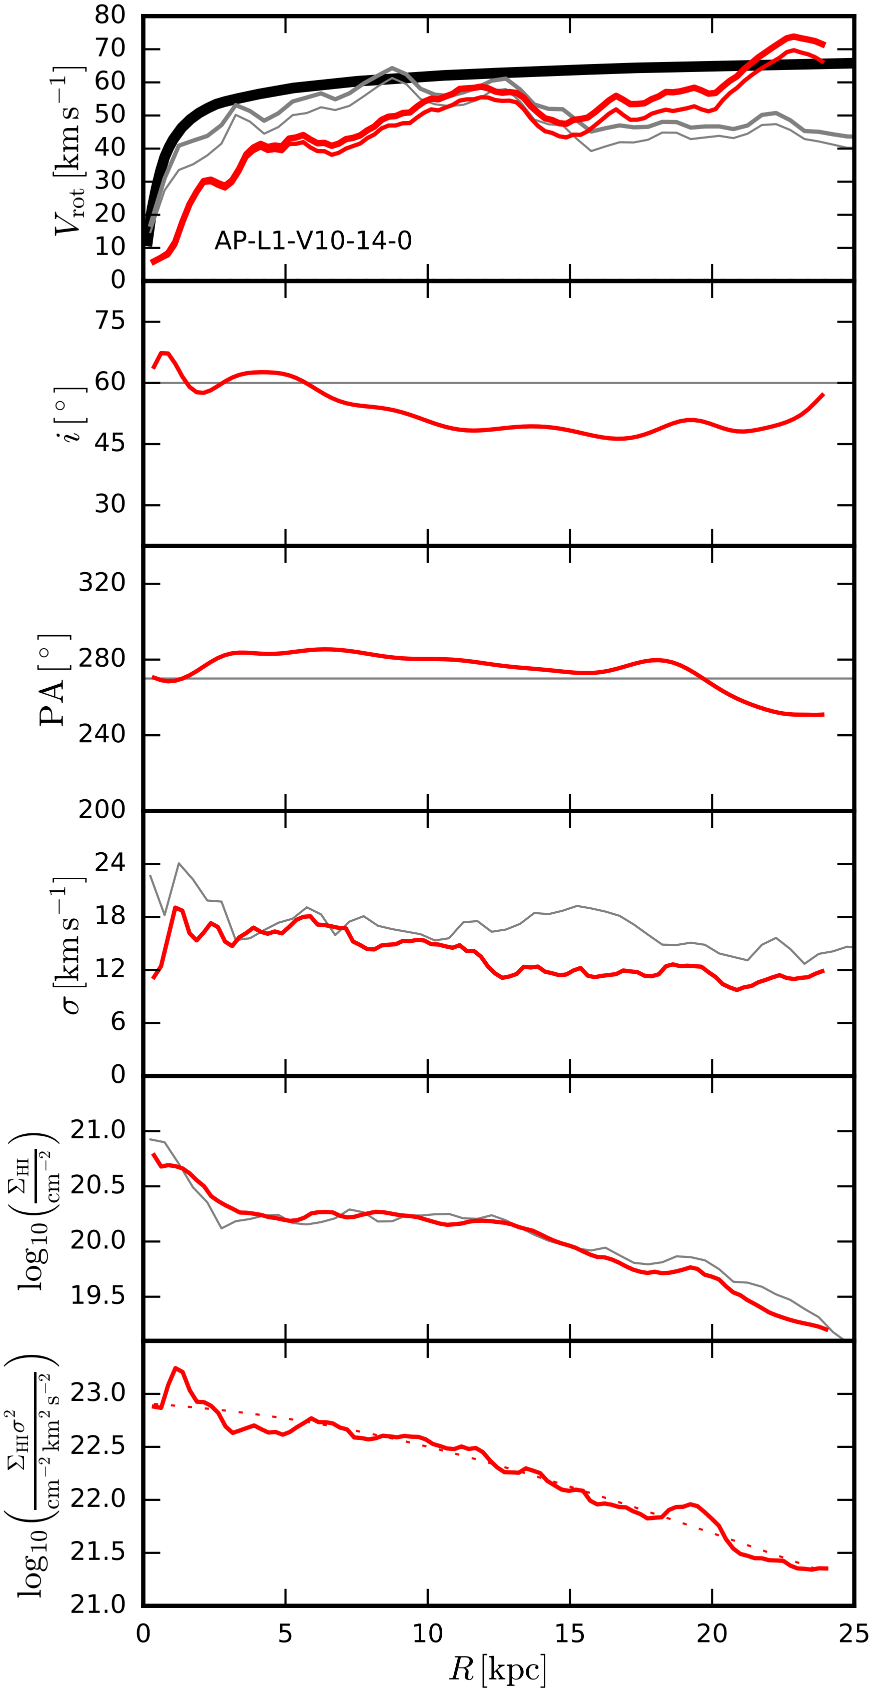


**Figure 24** – *continued*

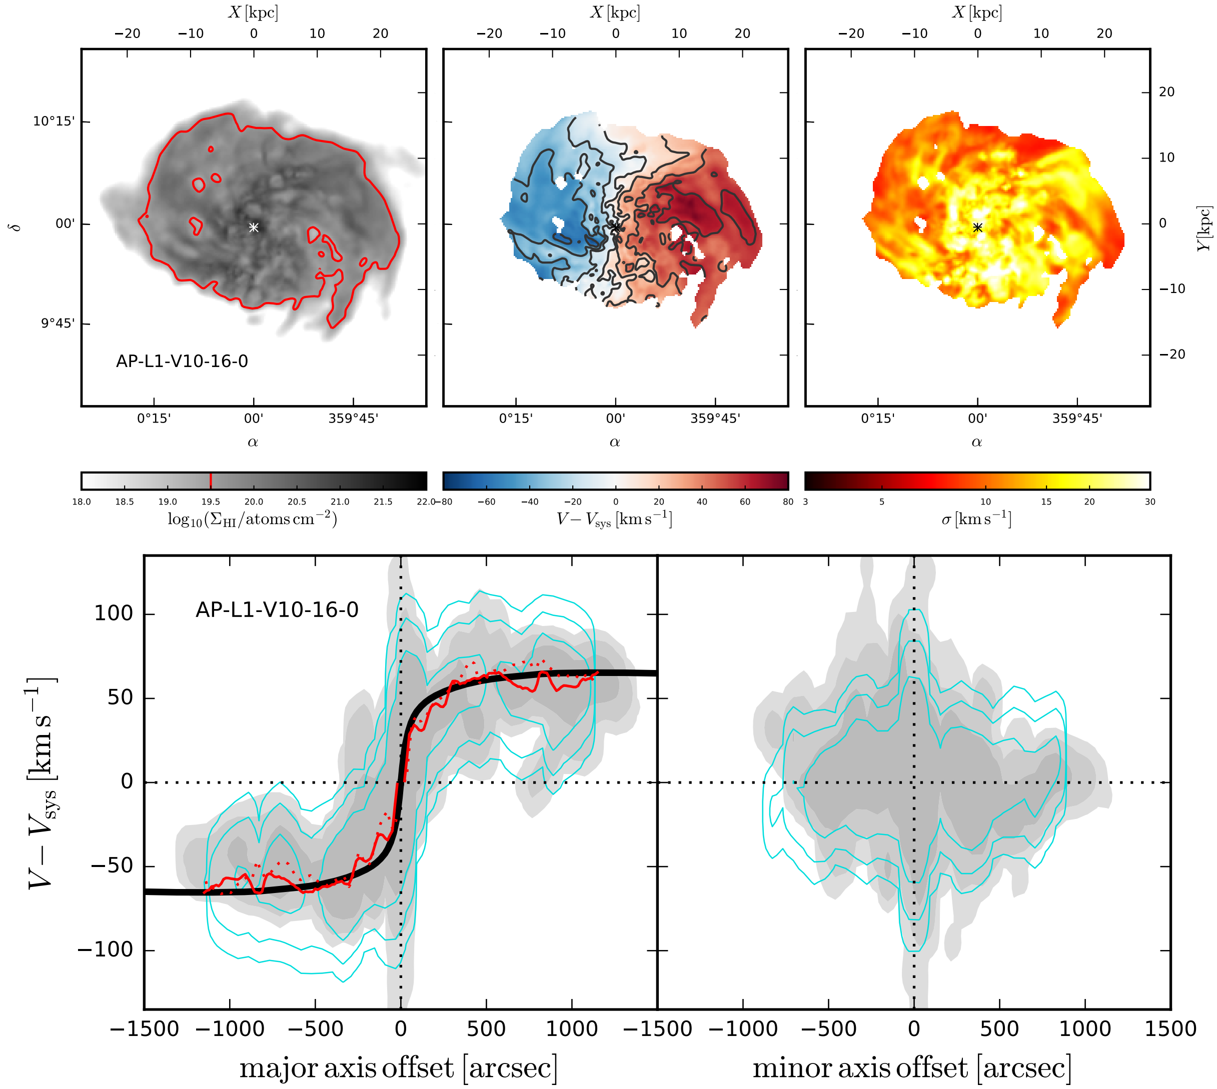


**Figure 25.** Moment maps, position-velocity diagrams and rotation curve fit summary (next page) for AP-L1-V10-16-0. See text for detailed description.

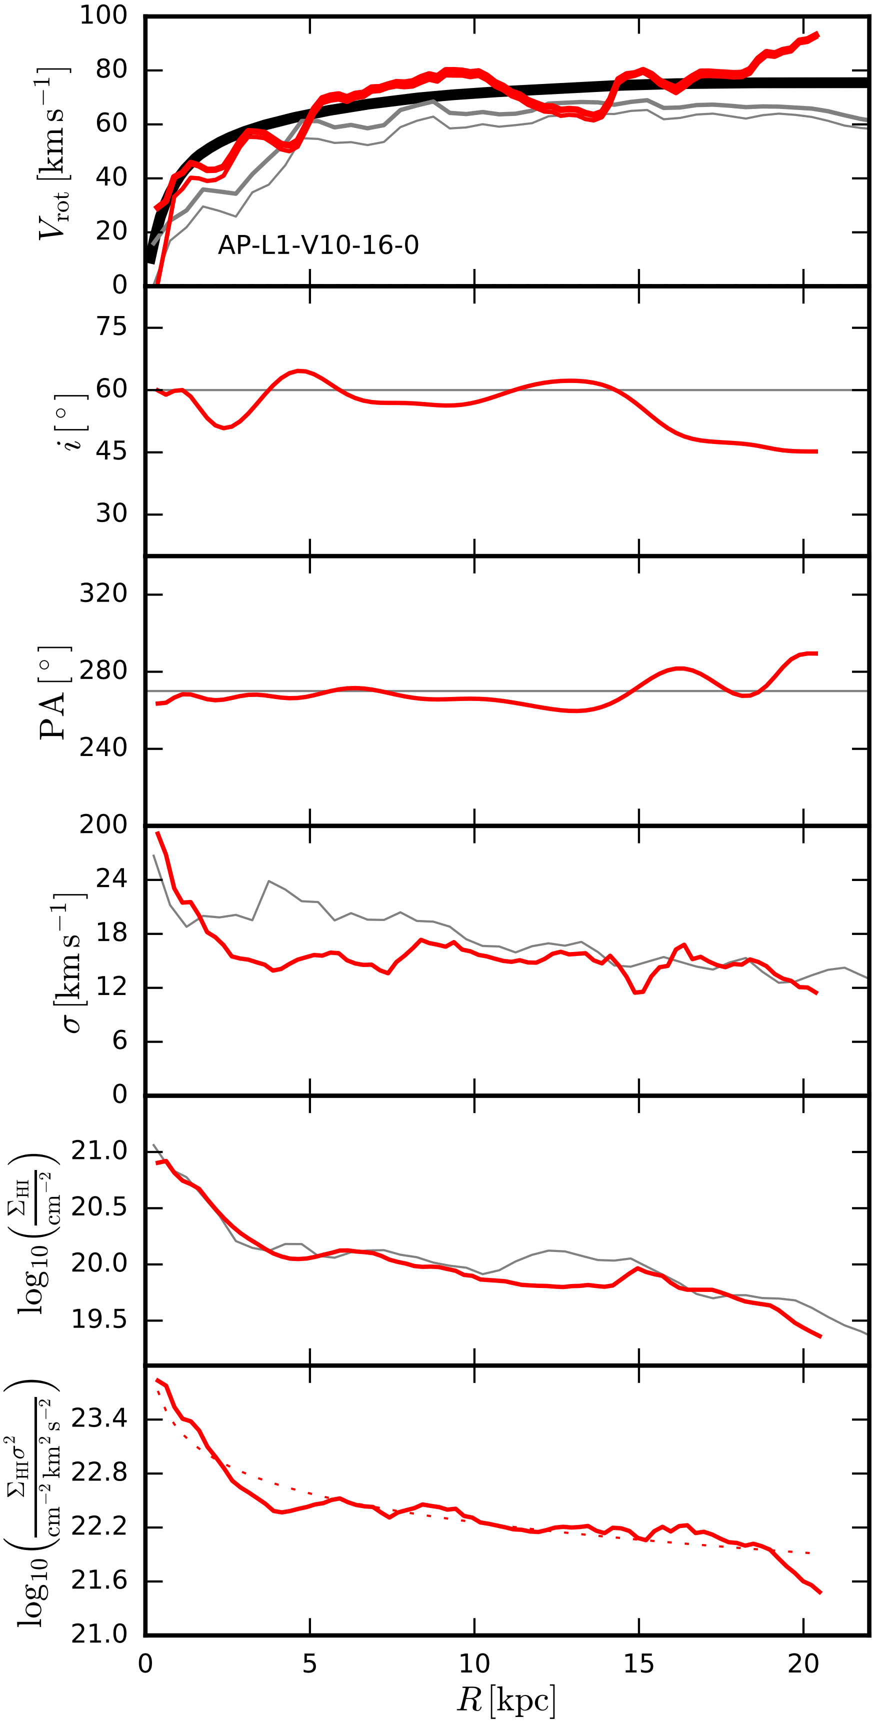


**Figure 25** – *continued*

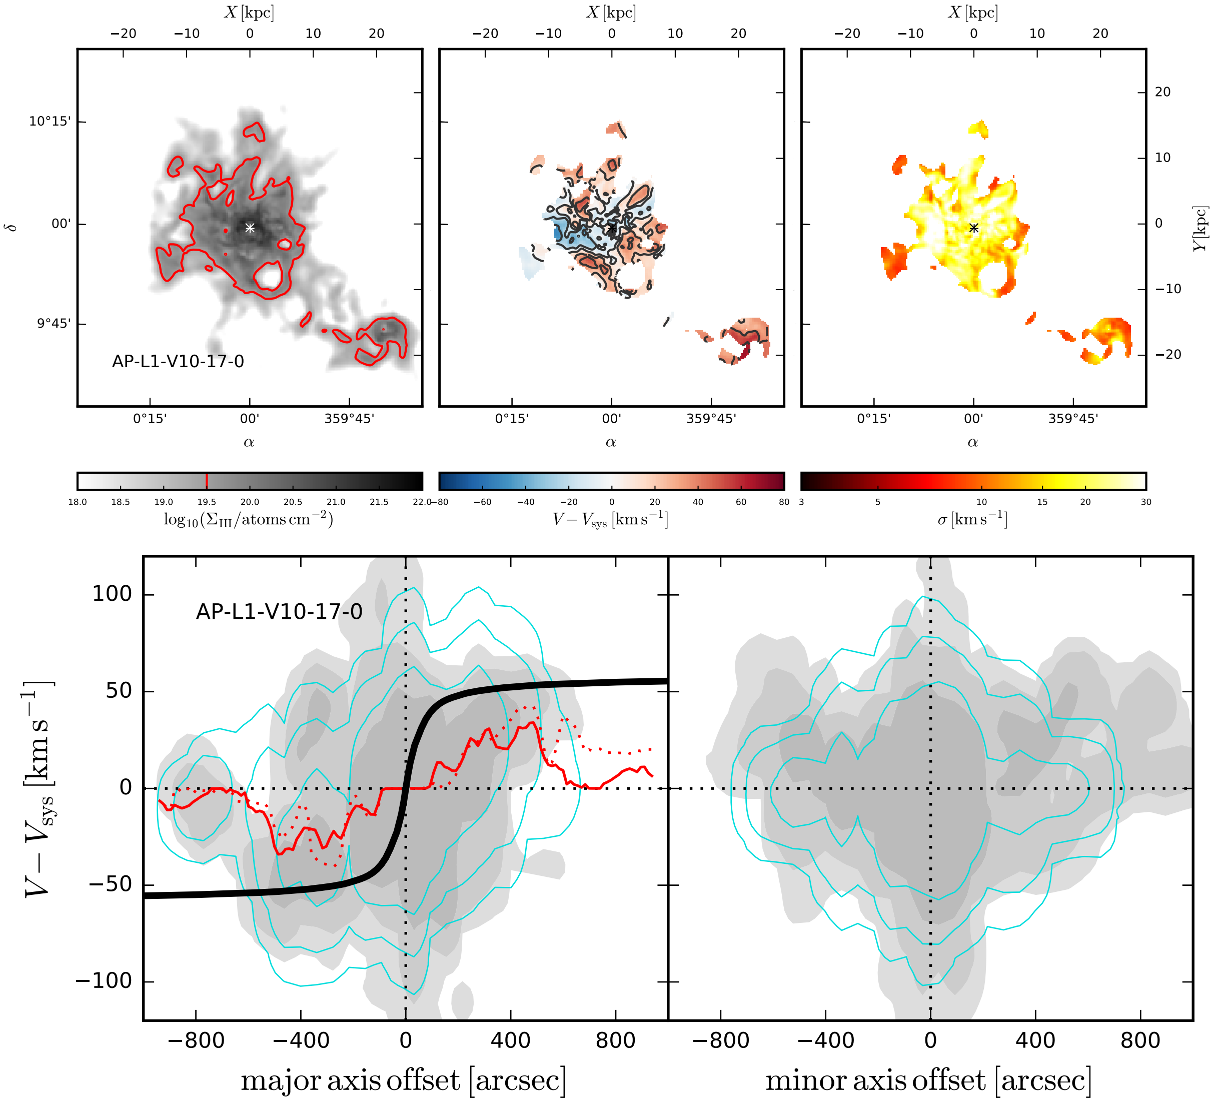


**Figure 26.** Moment maps, position-velocity diagrams and rotation curve fit summary (next page) for AP-L1-V10-17-0. See text for detailed description.

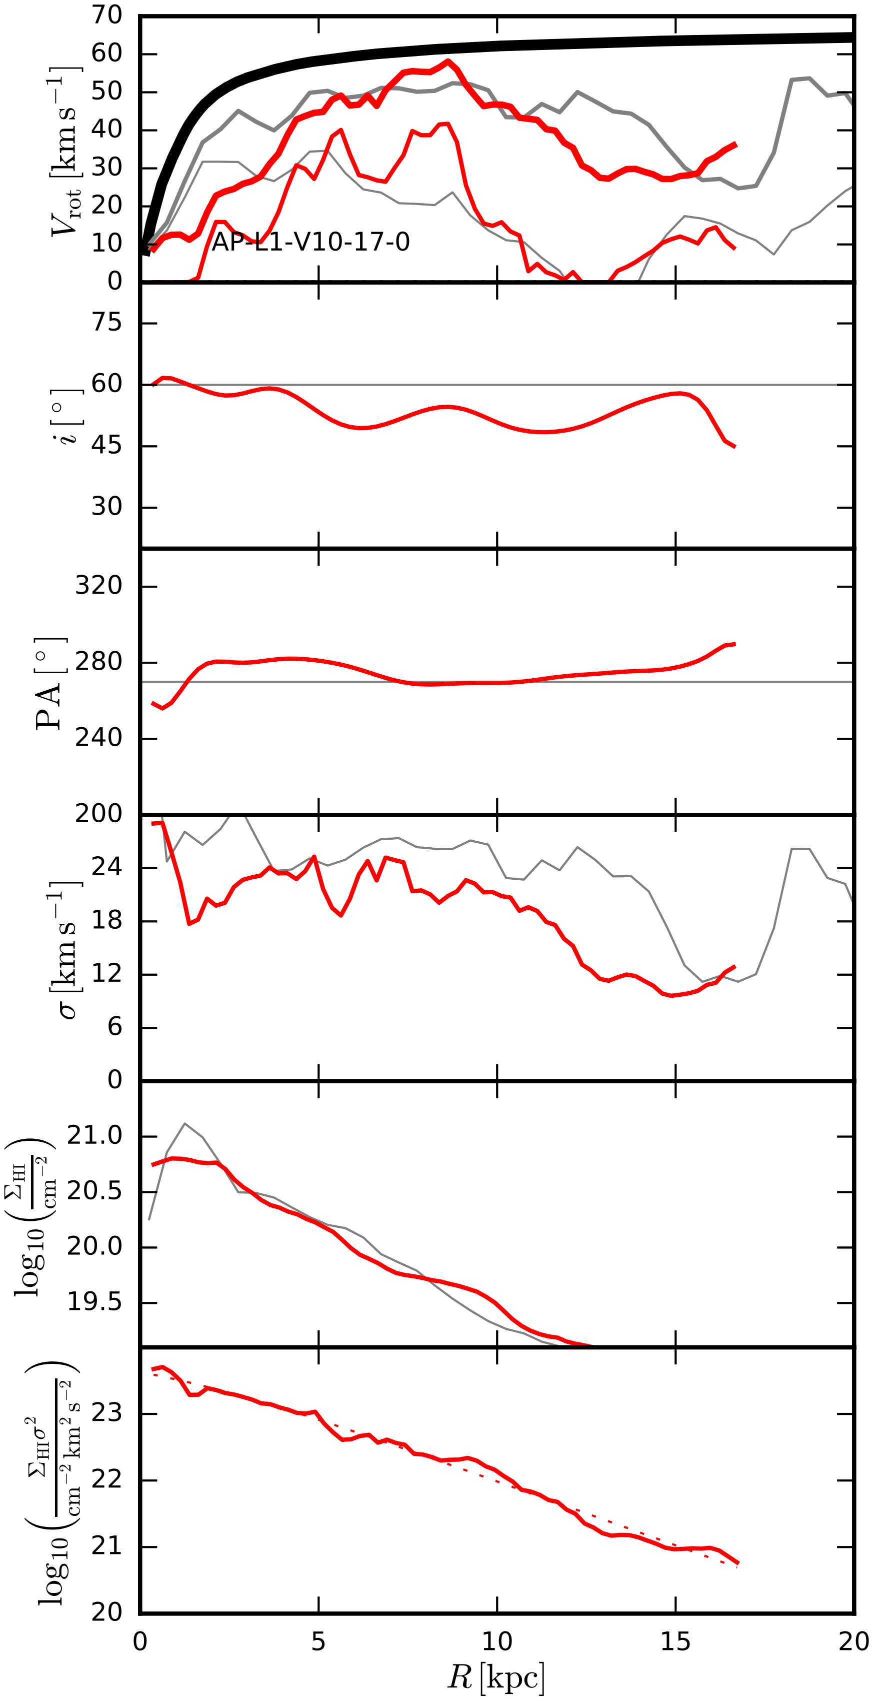


**Figure 26** – *continued*

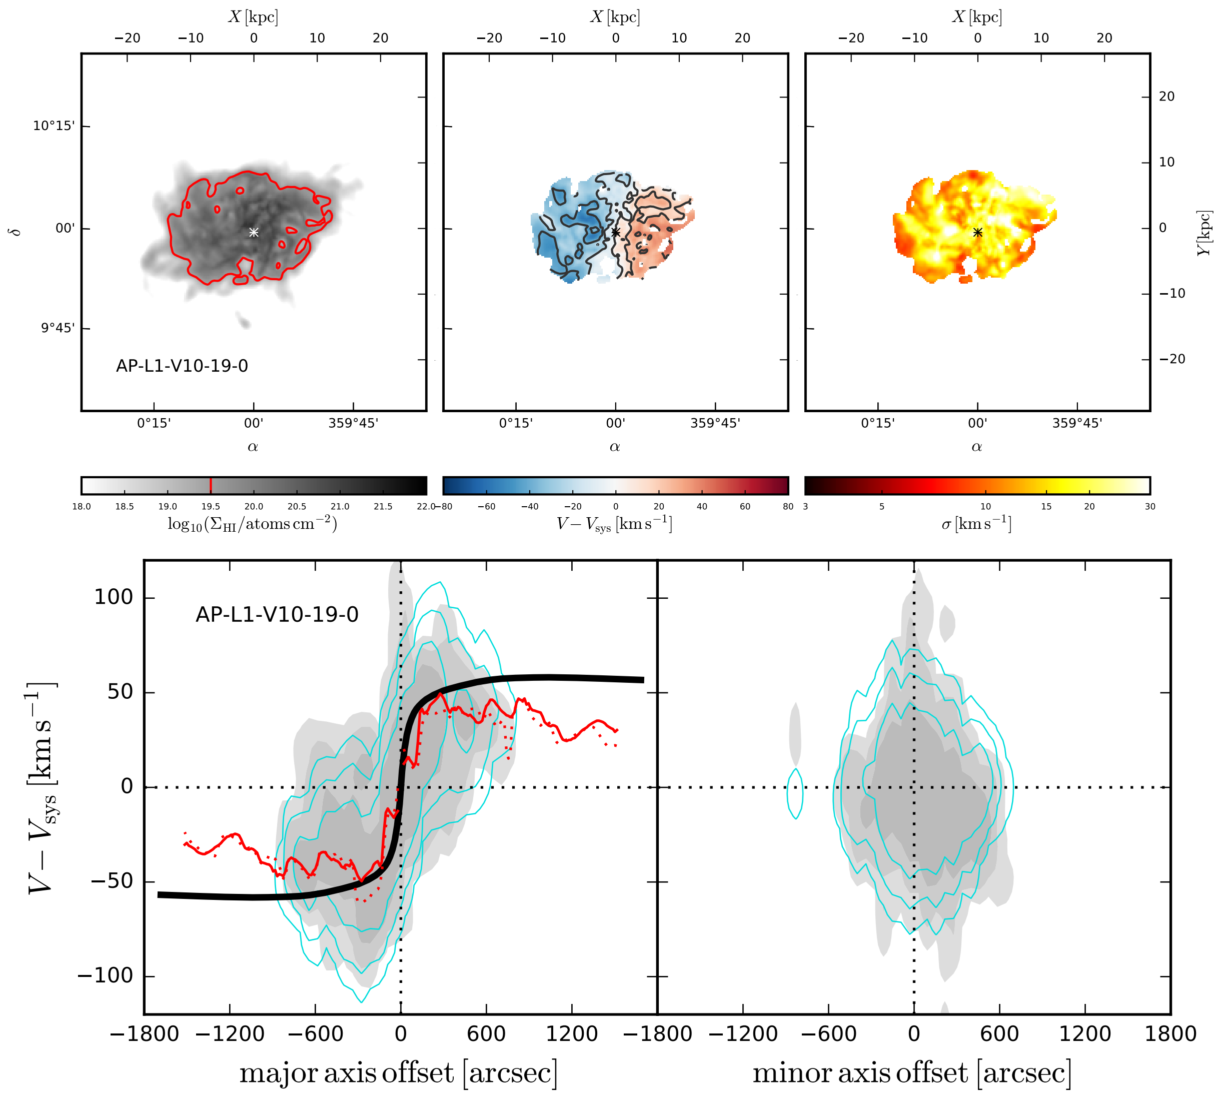


**Figure 27.** Moment maps, position-velocity diagrams and rotation curve fit summary (next page) for AP-L1-V10-19-0. See text for detailed description.

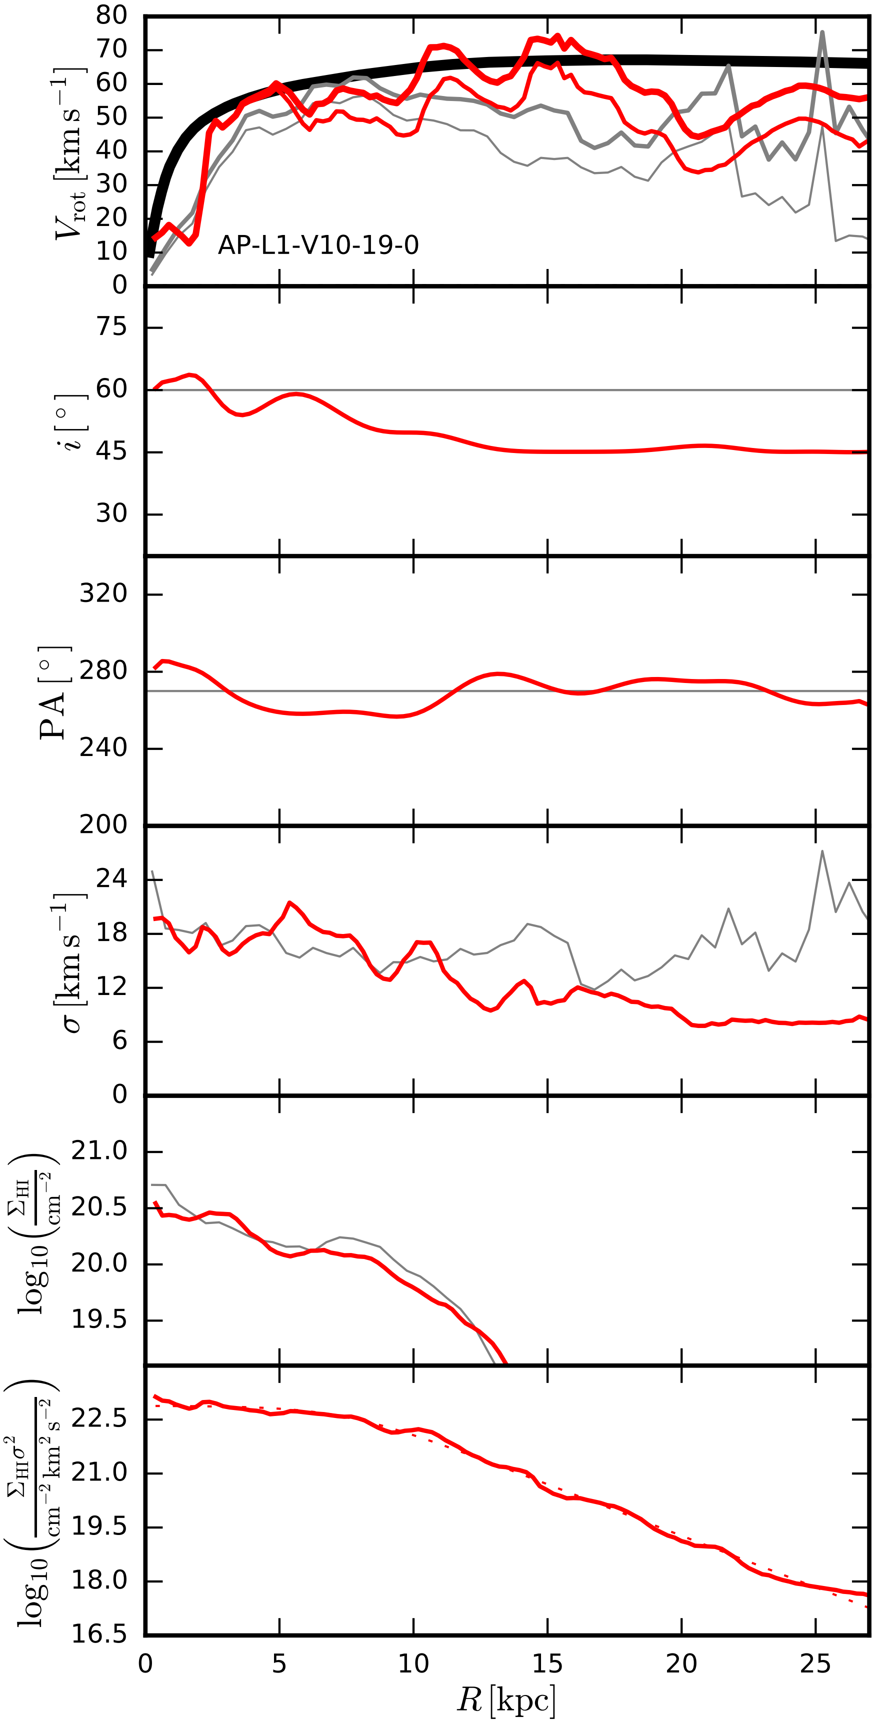


**Figure 27** – *continued*

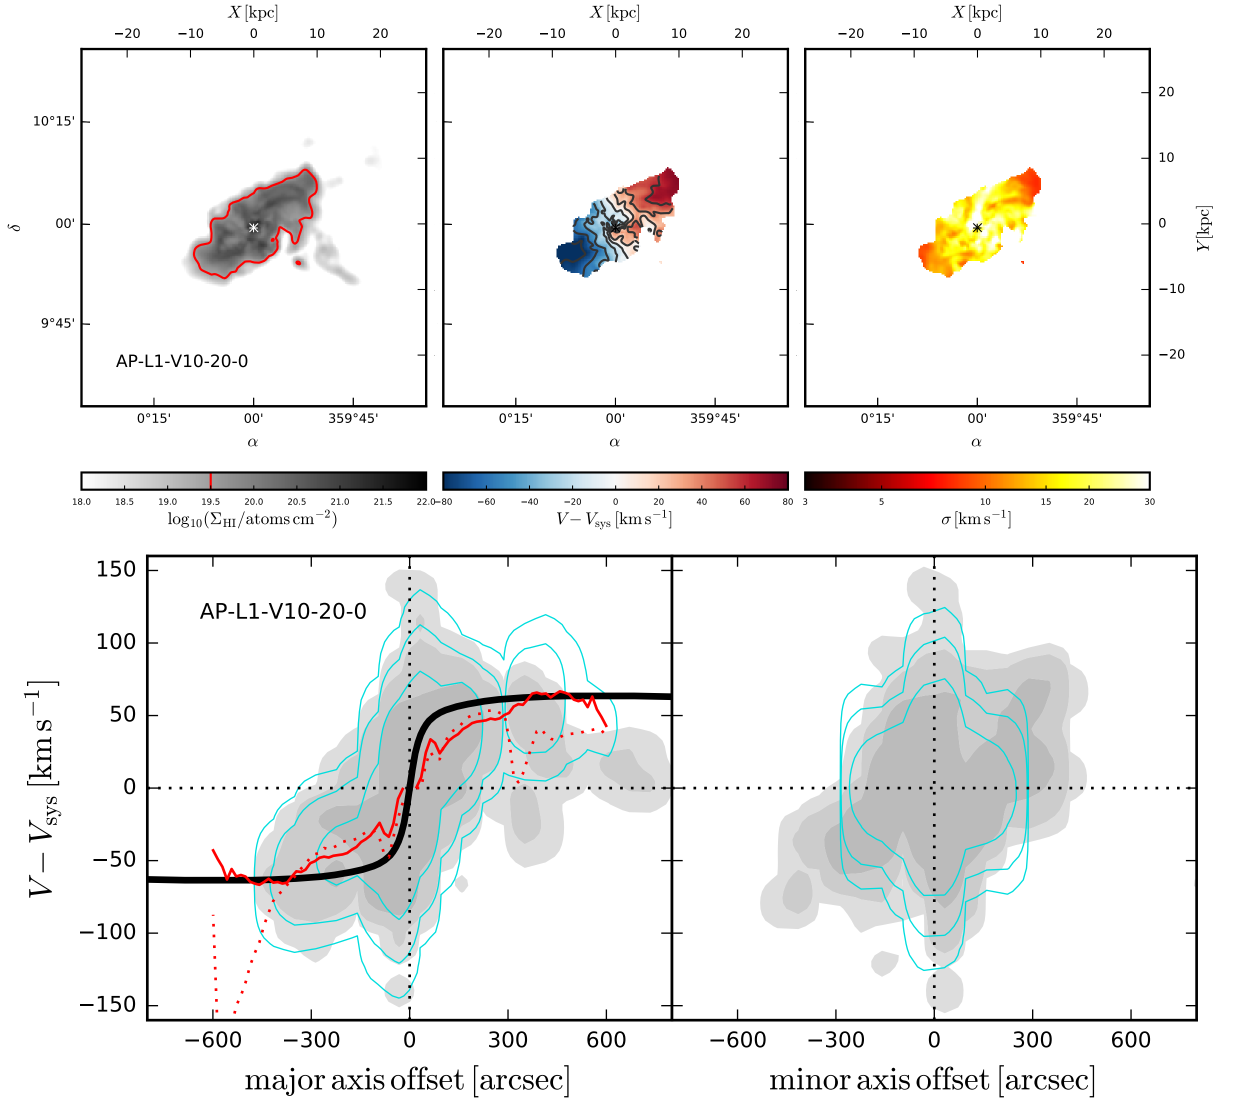


**Figure 28.** Moment maps, position-velocity diagrams and rotation curve fit summary (next page) for AP-L1-V10-20-0. See text for detailed description.

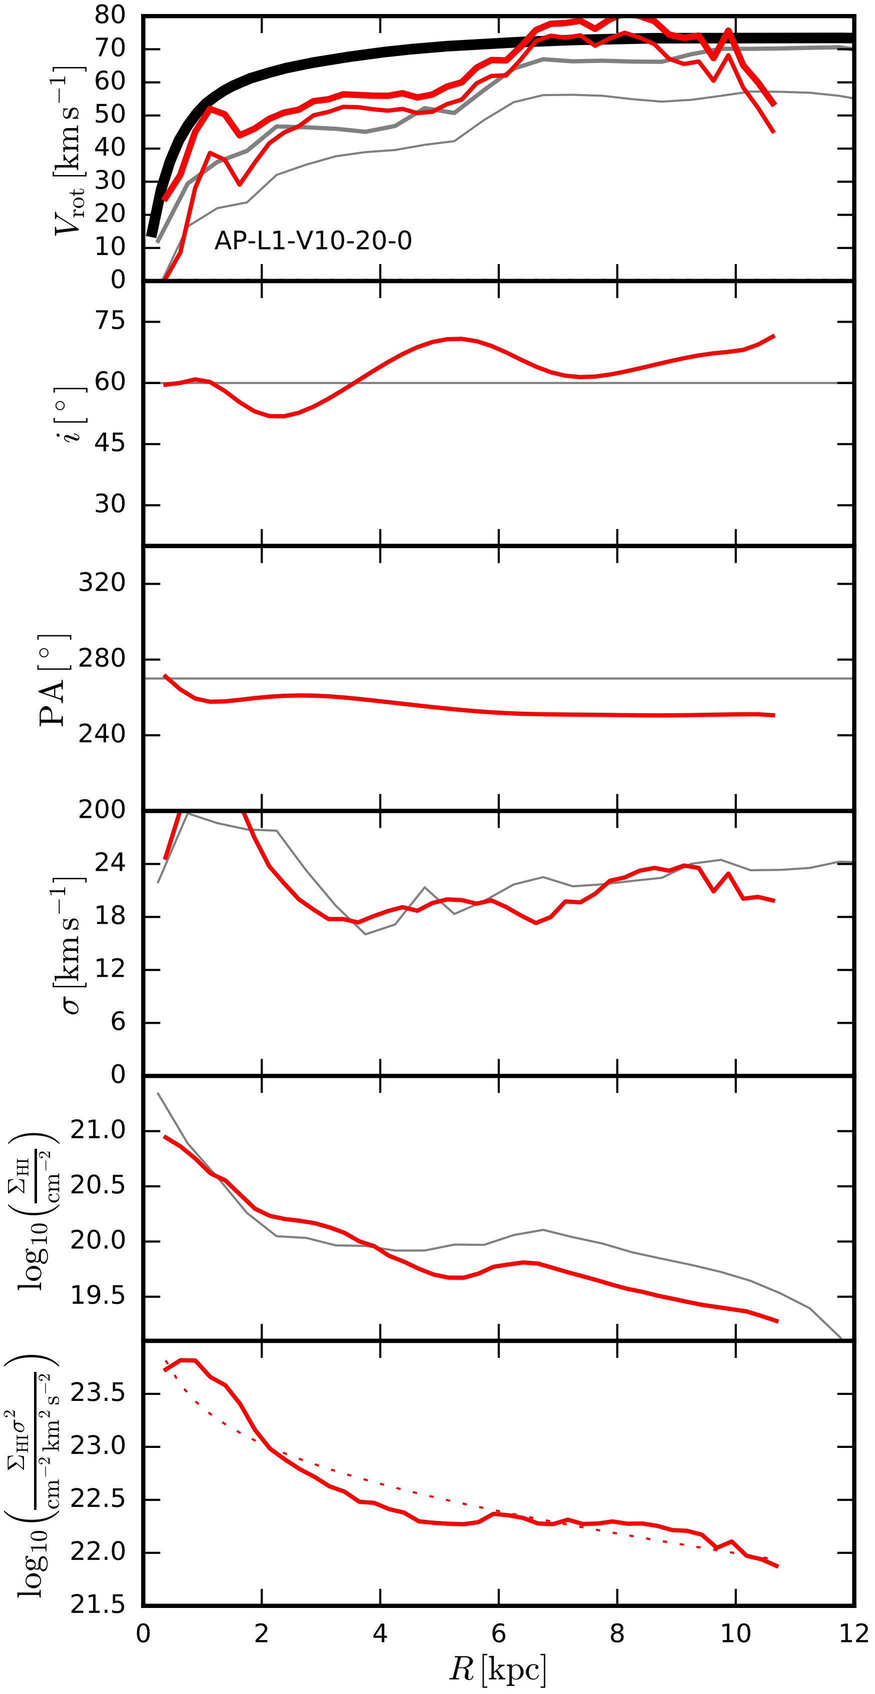


**Figure 28** – *continued*

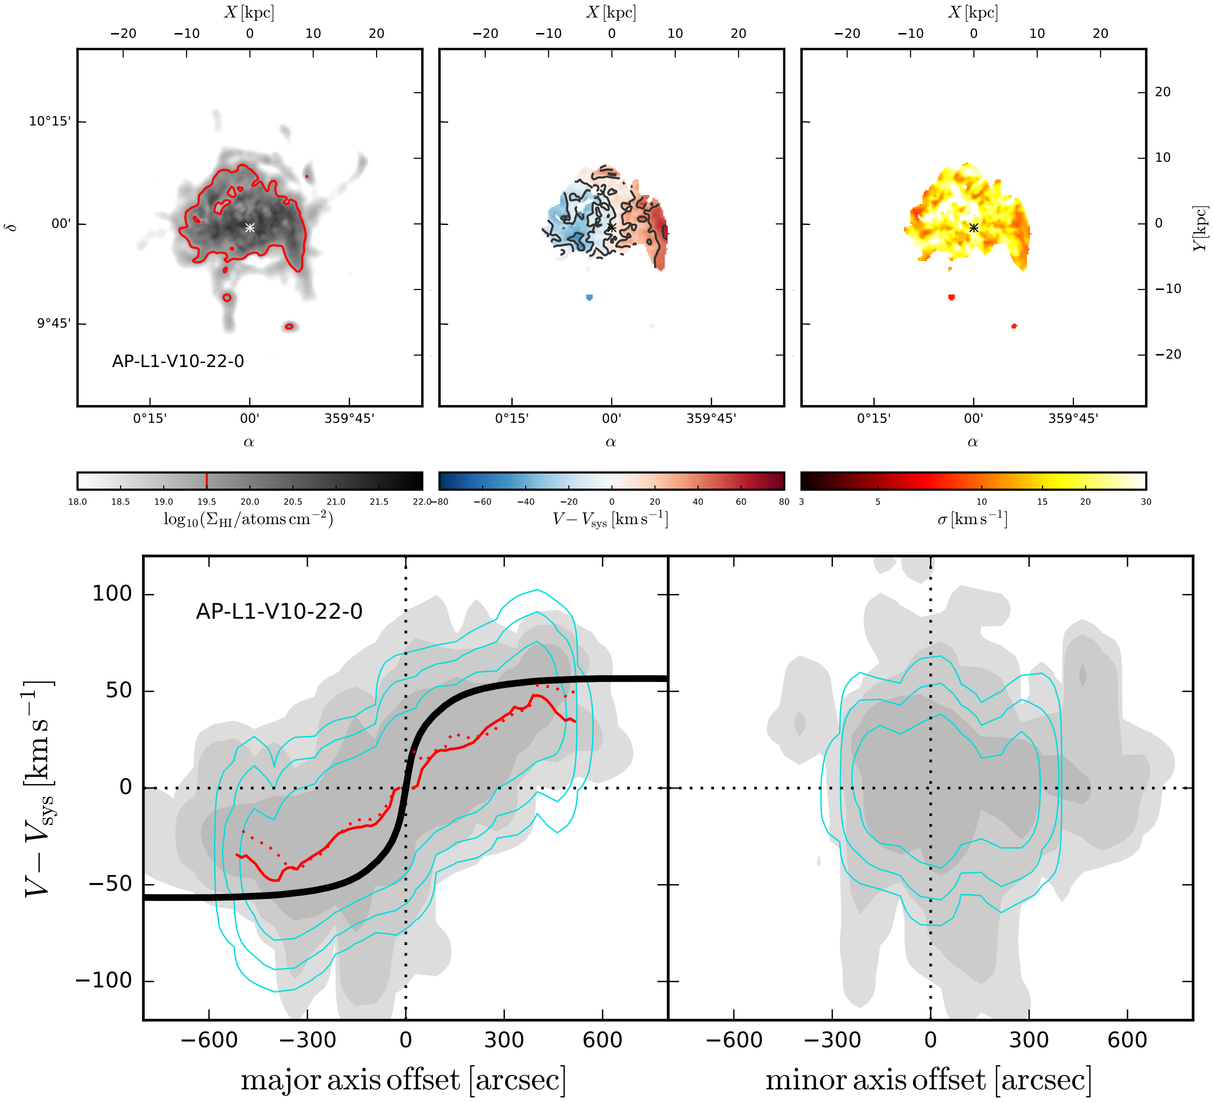


**Figure 29.** Moment maps, position-velocity diagrams and rotation curve fit summary (next page) for AP-L1-V10-22-0. See text for detailed description.

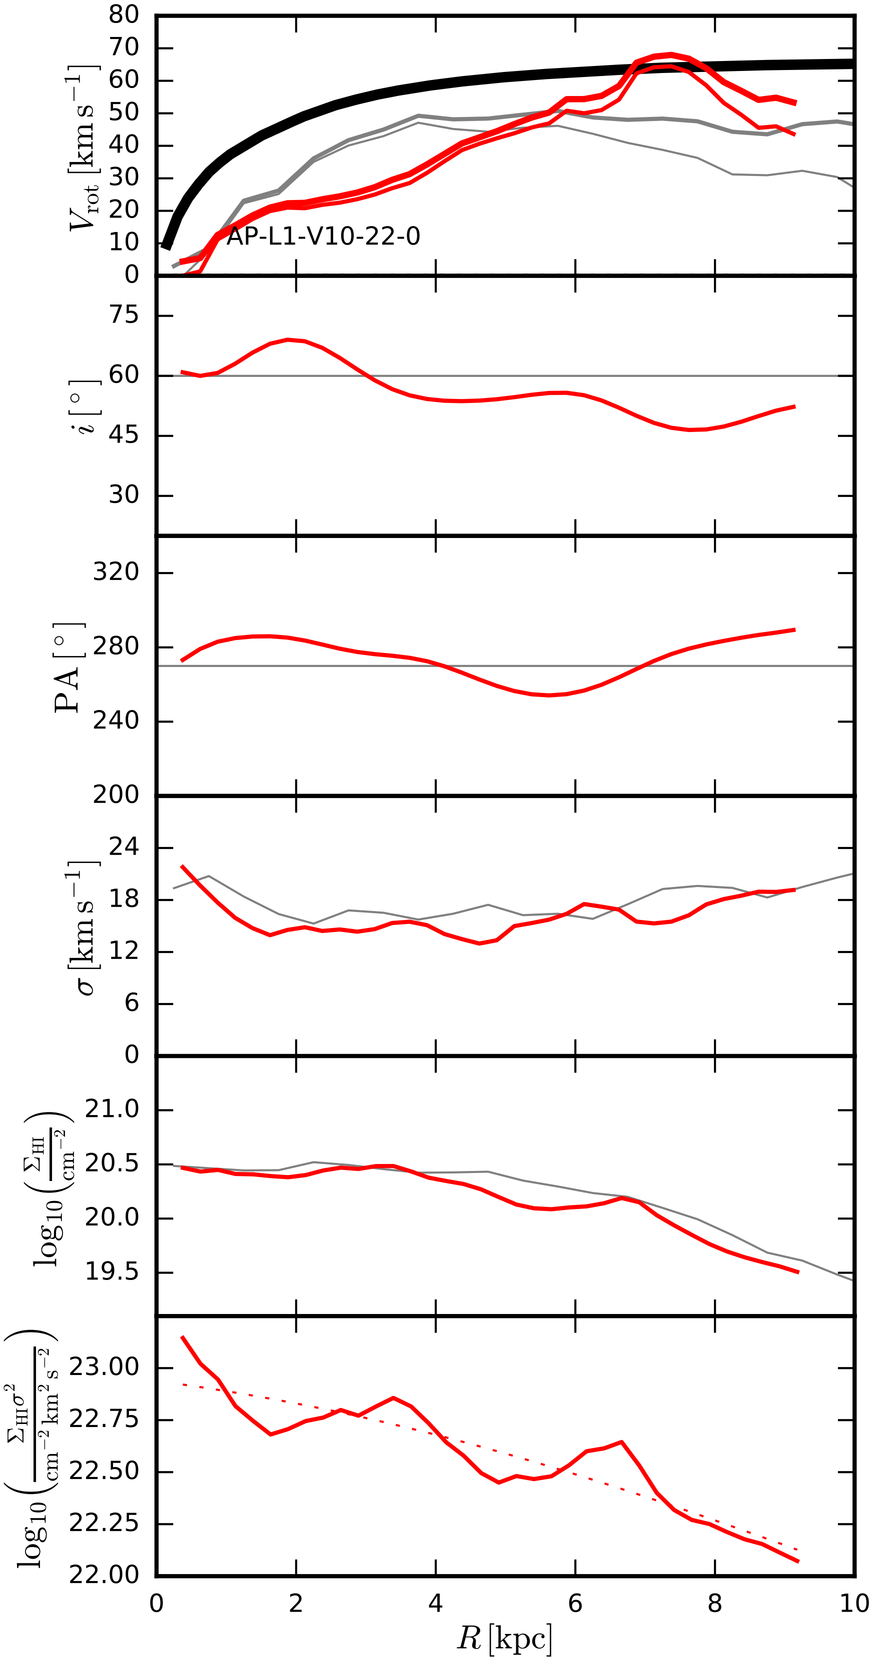


**Figure 29** – *continued*

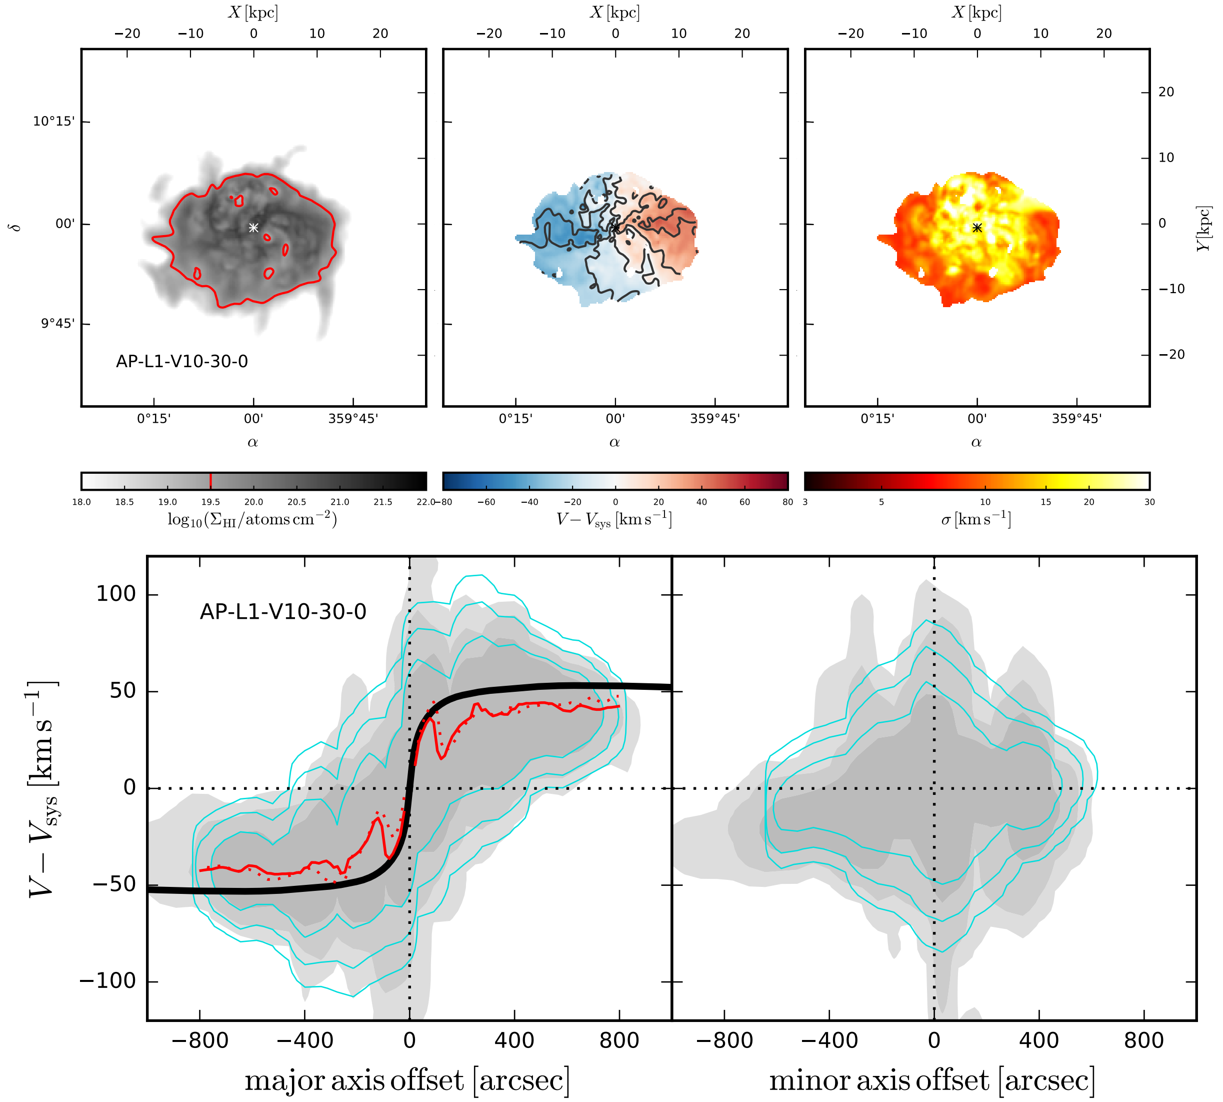


**Figure 30.** Moment maps, position-velocity diagrams and rotation curve fit summary (next page) for AP-L1-V10-30-0. See text for detailed description.

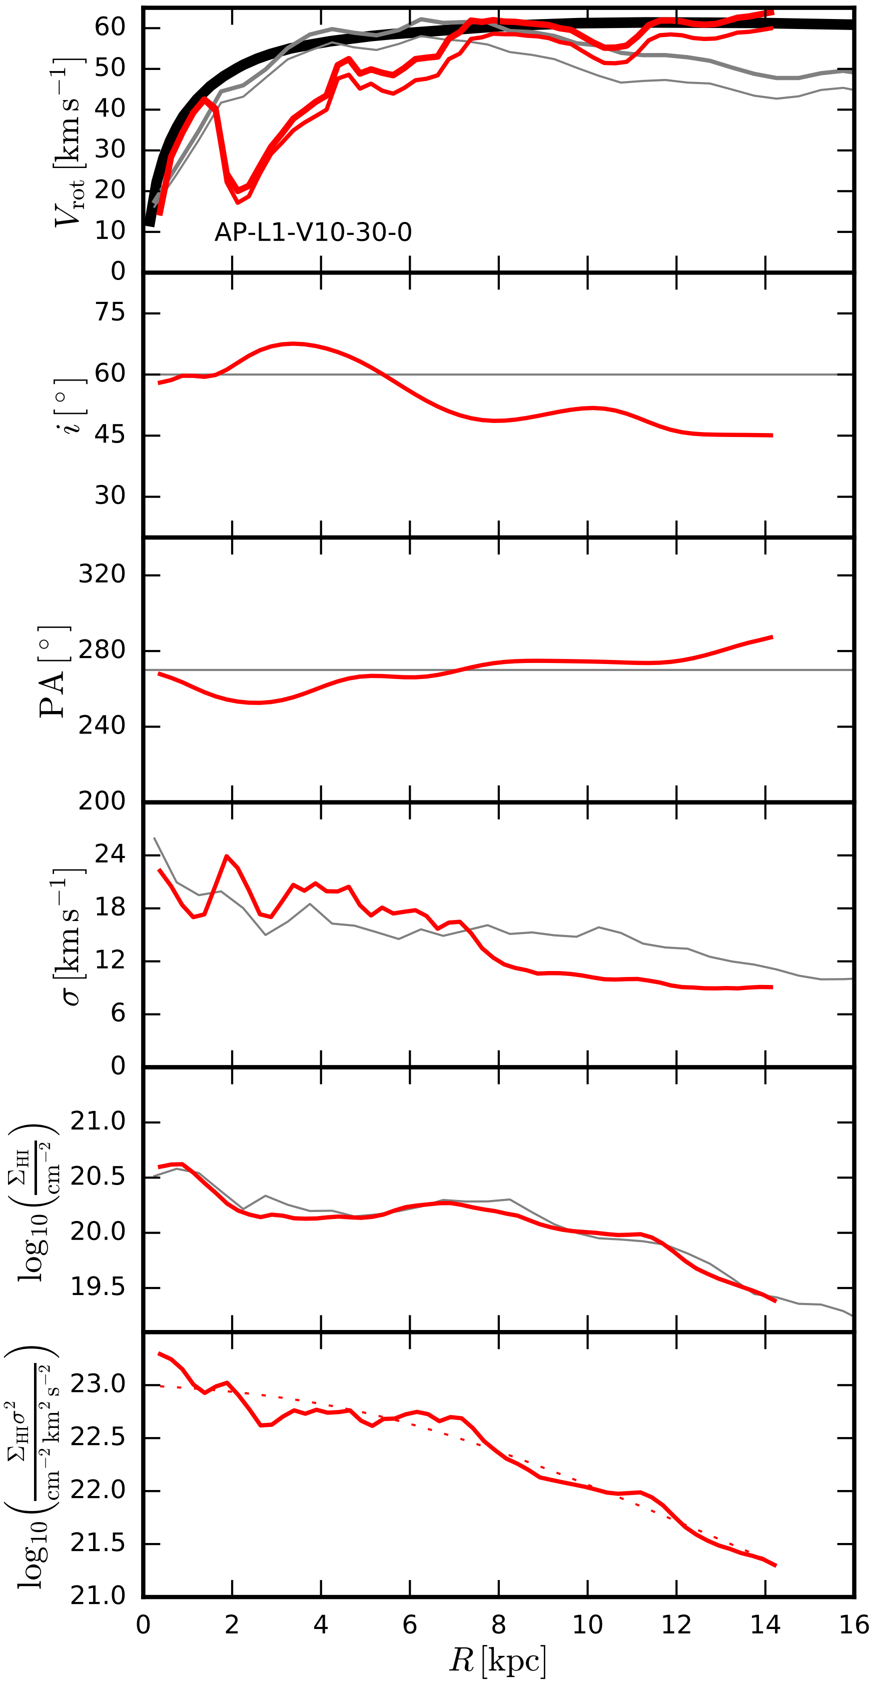


**Figure 30** – *continued*

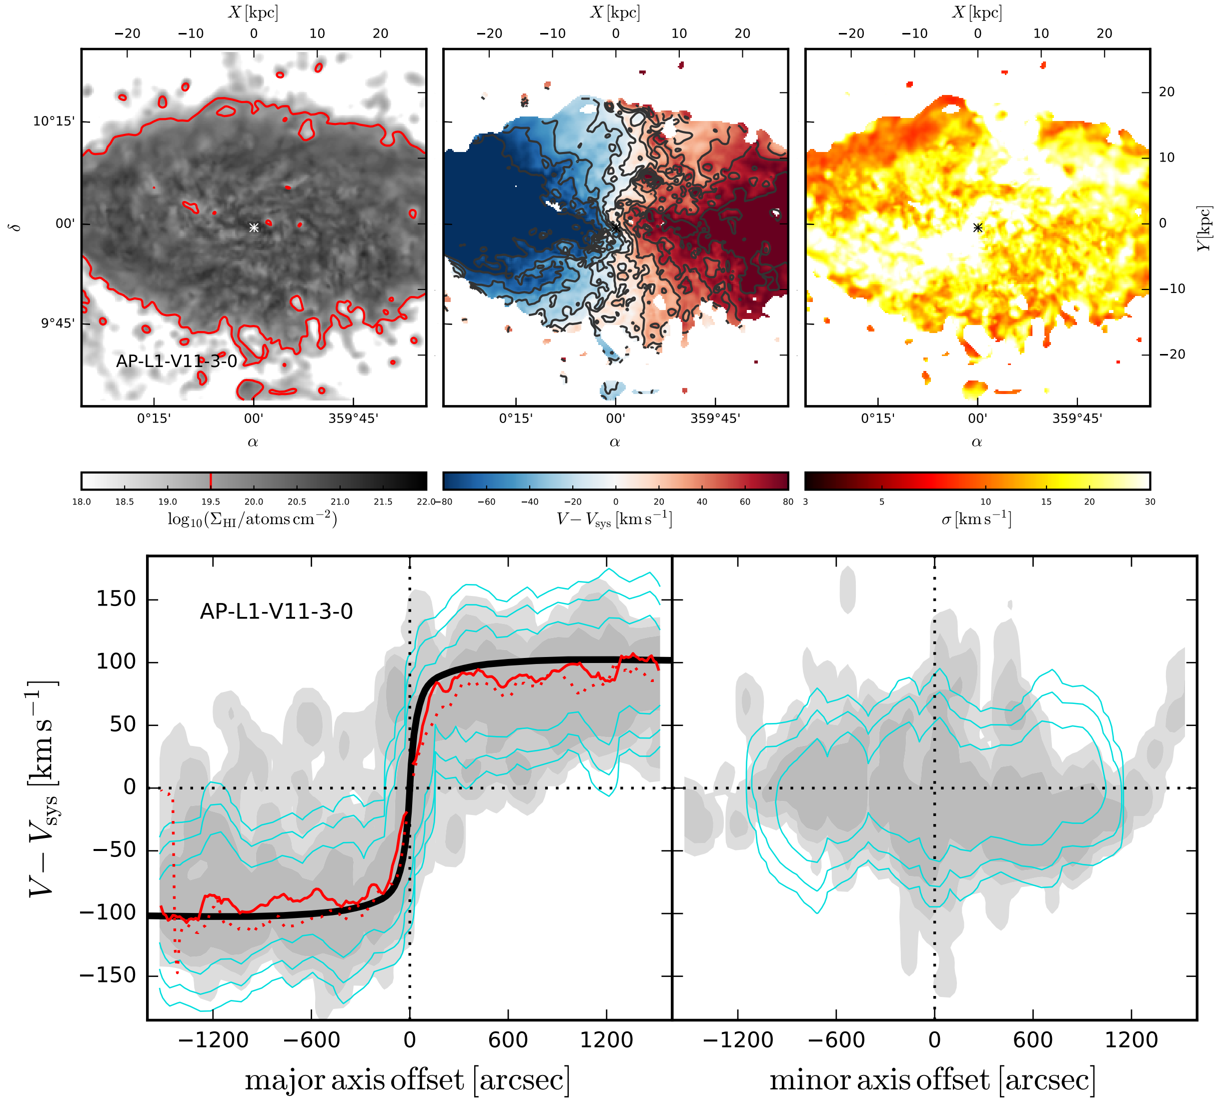


**Figure 31.** Moment maps, position-velocity diagrams and rotation curve fit summary (next page) for AP-L1-V11-3-0. See text for detailed description.

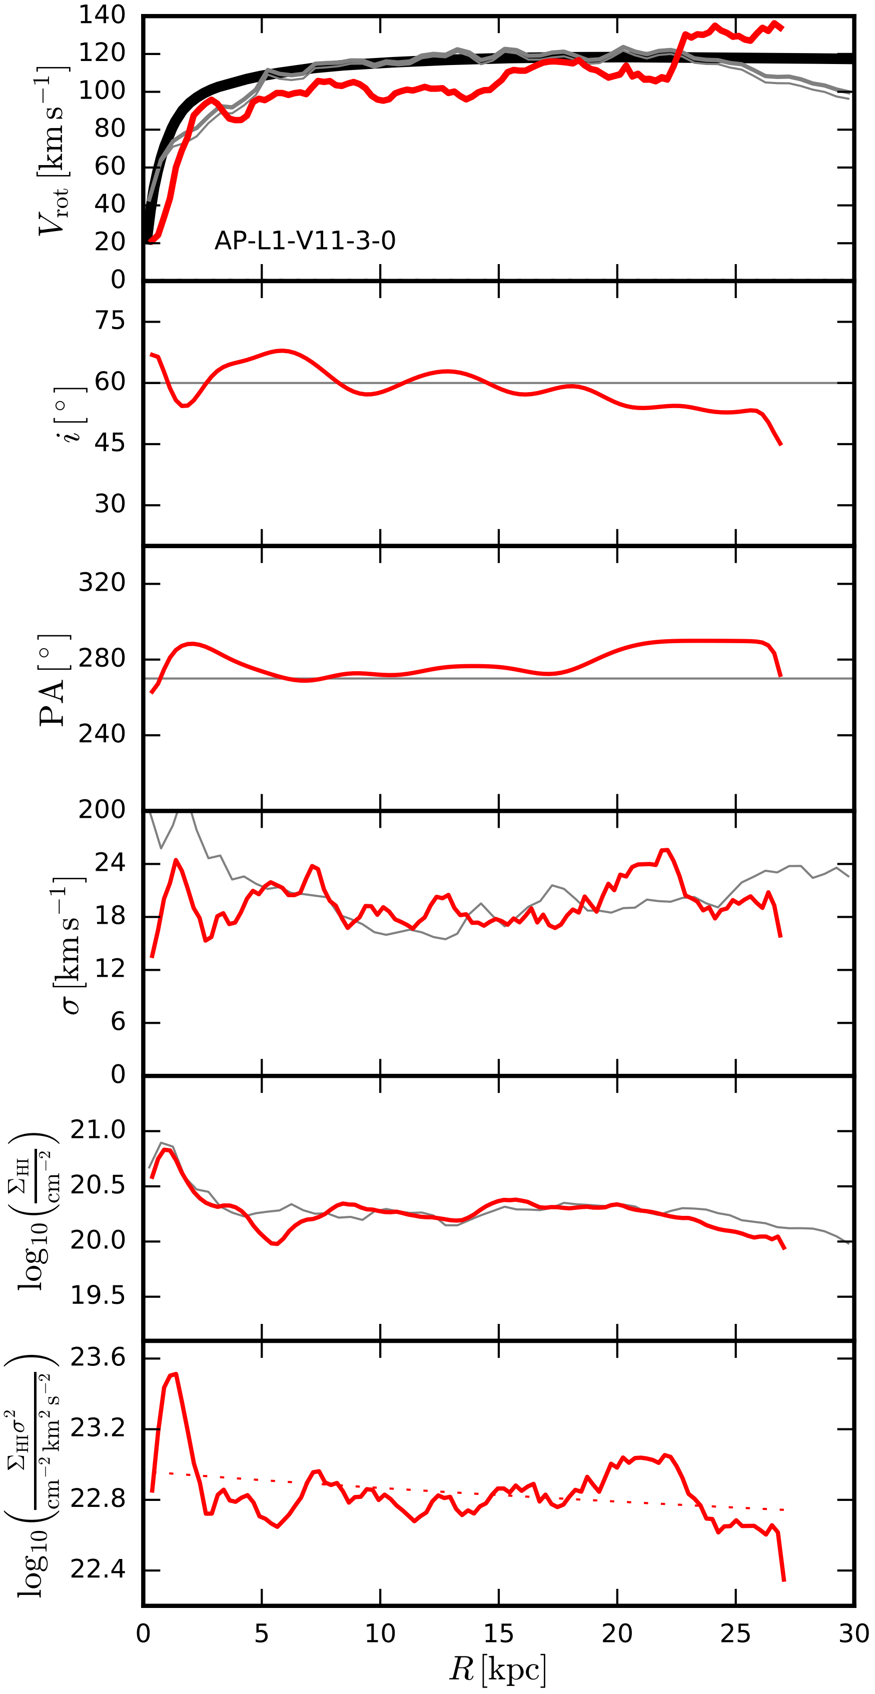


**Figure 31** – *continued*

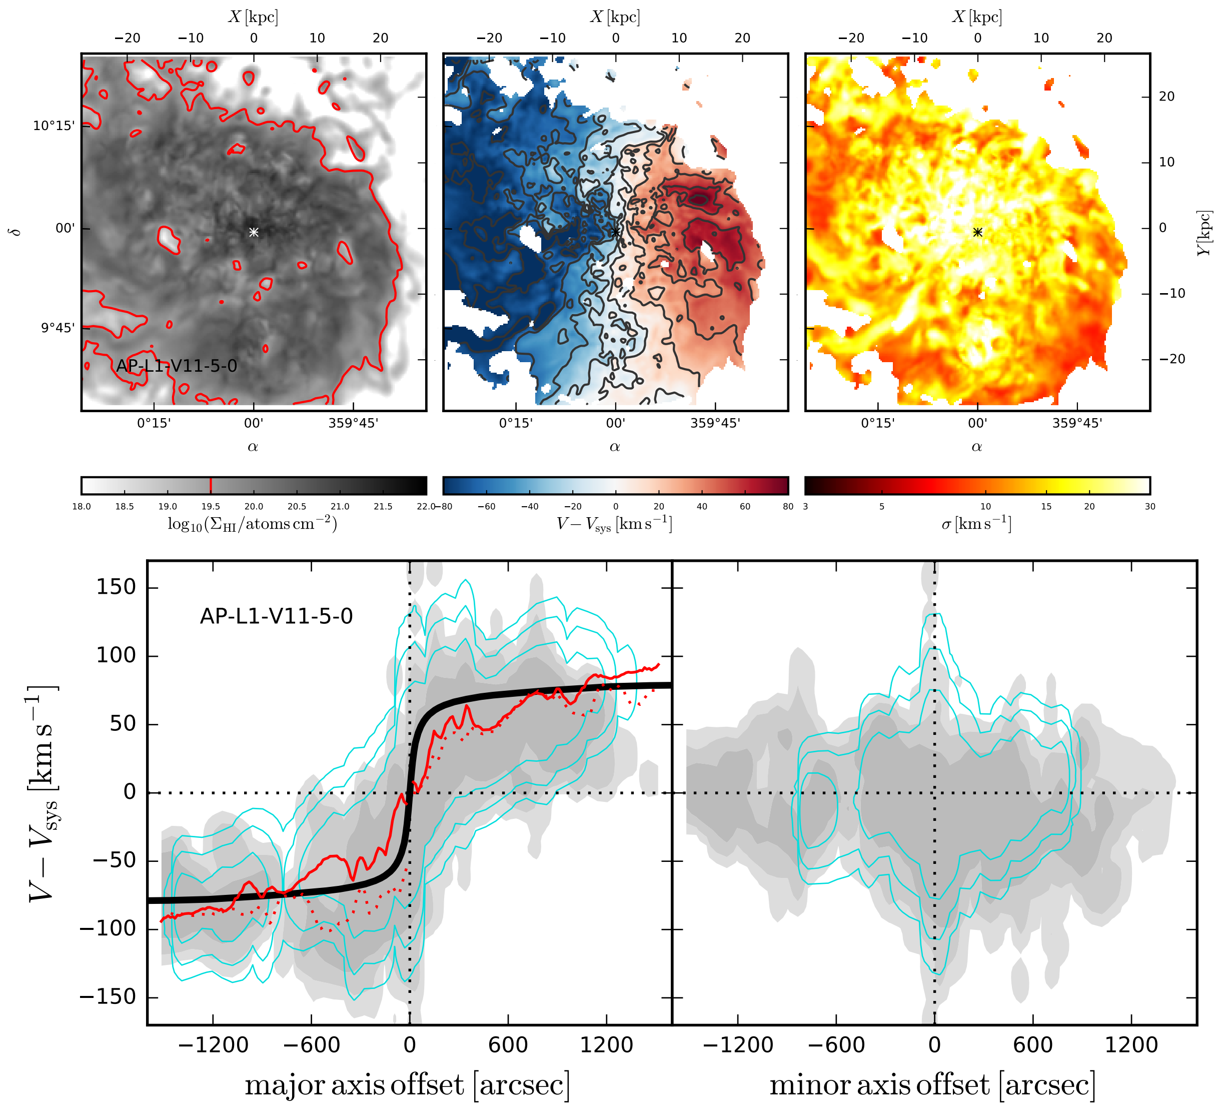


**Figure 32.** Moment maps, position-velocity diagrams and rotation curve fit summary (next page) for AP-L1-V11-5-0. See text for detailed description.

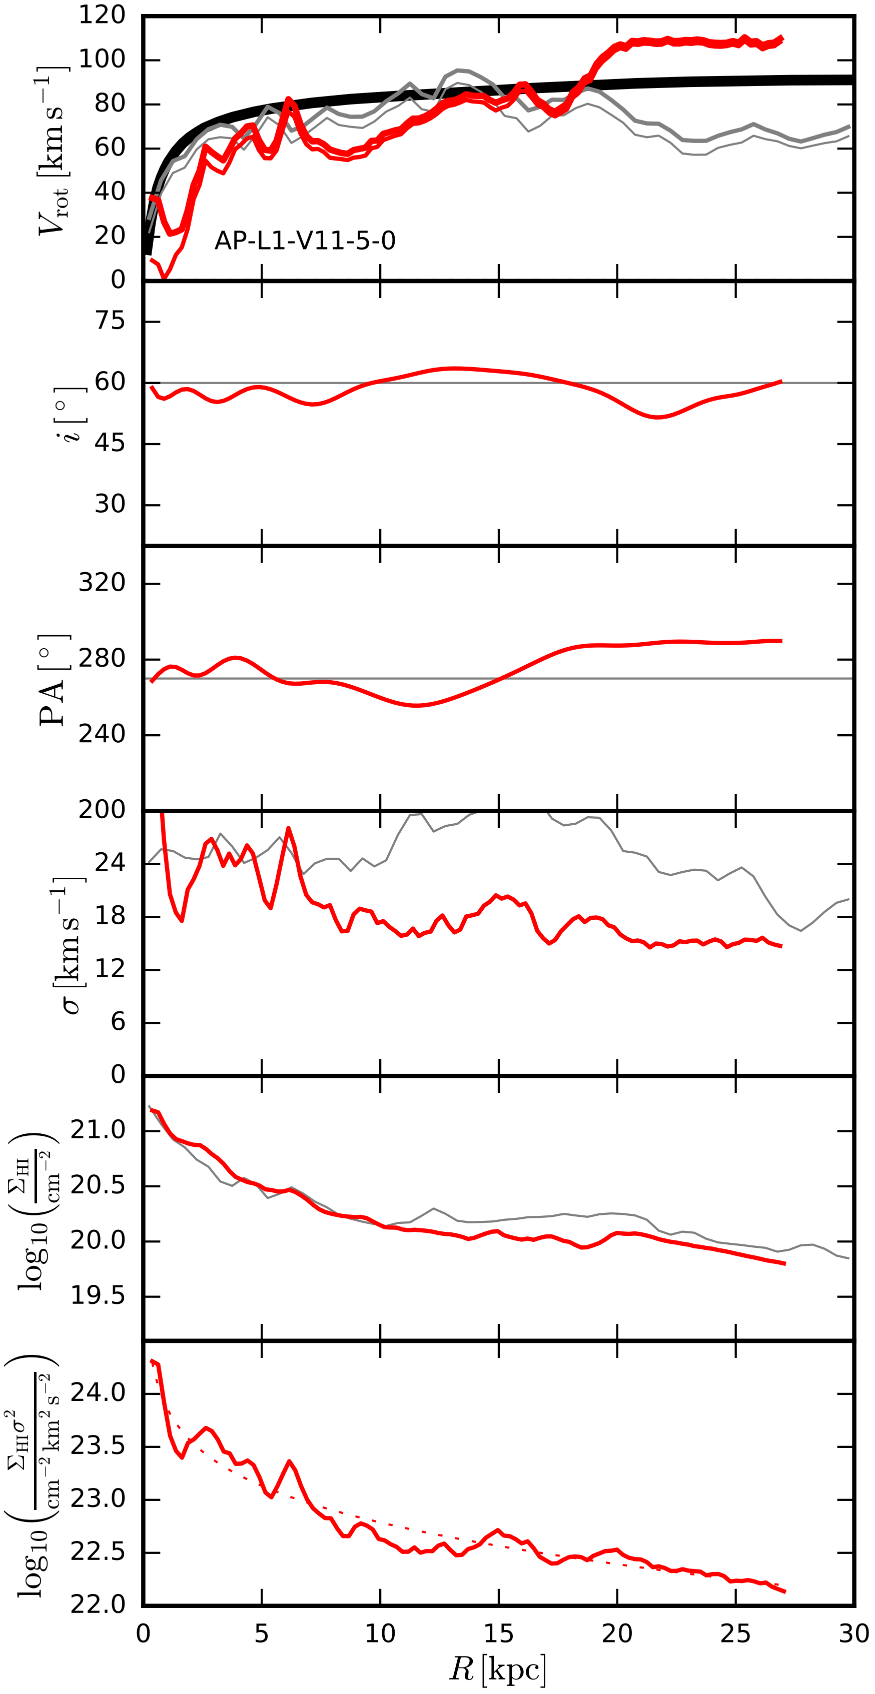


**Figure 32** – *continued*

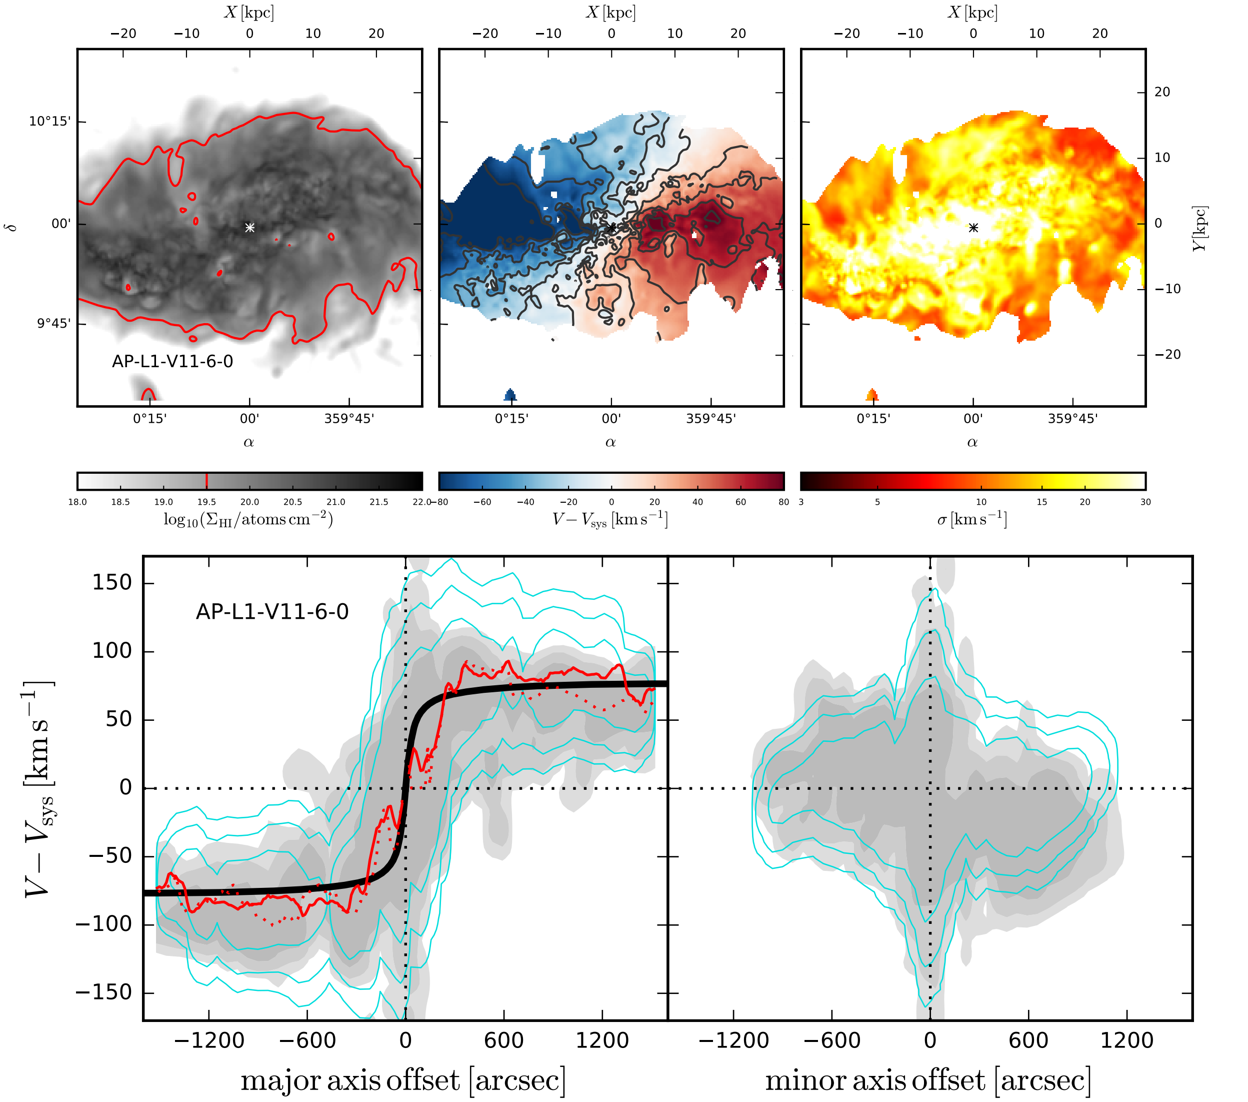


**Figure 33.** Moment maps, position-velocity diagrams and rotation curve fit summary (next page) for AP-L1-V11-6-0. See text for detailed description.

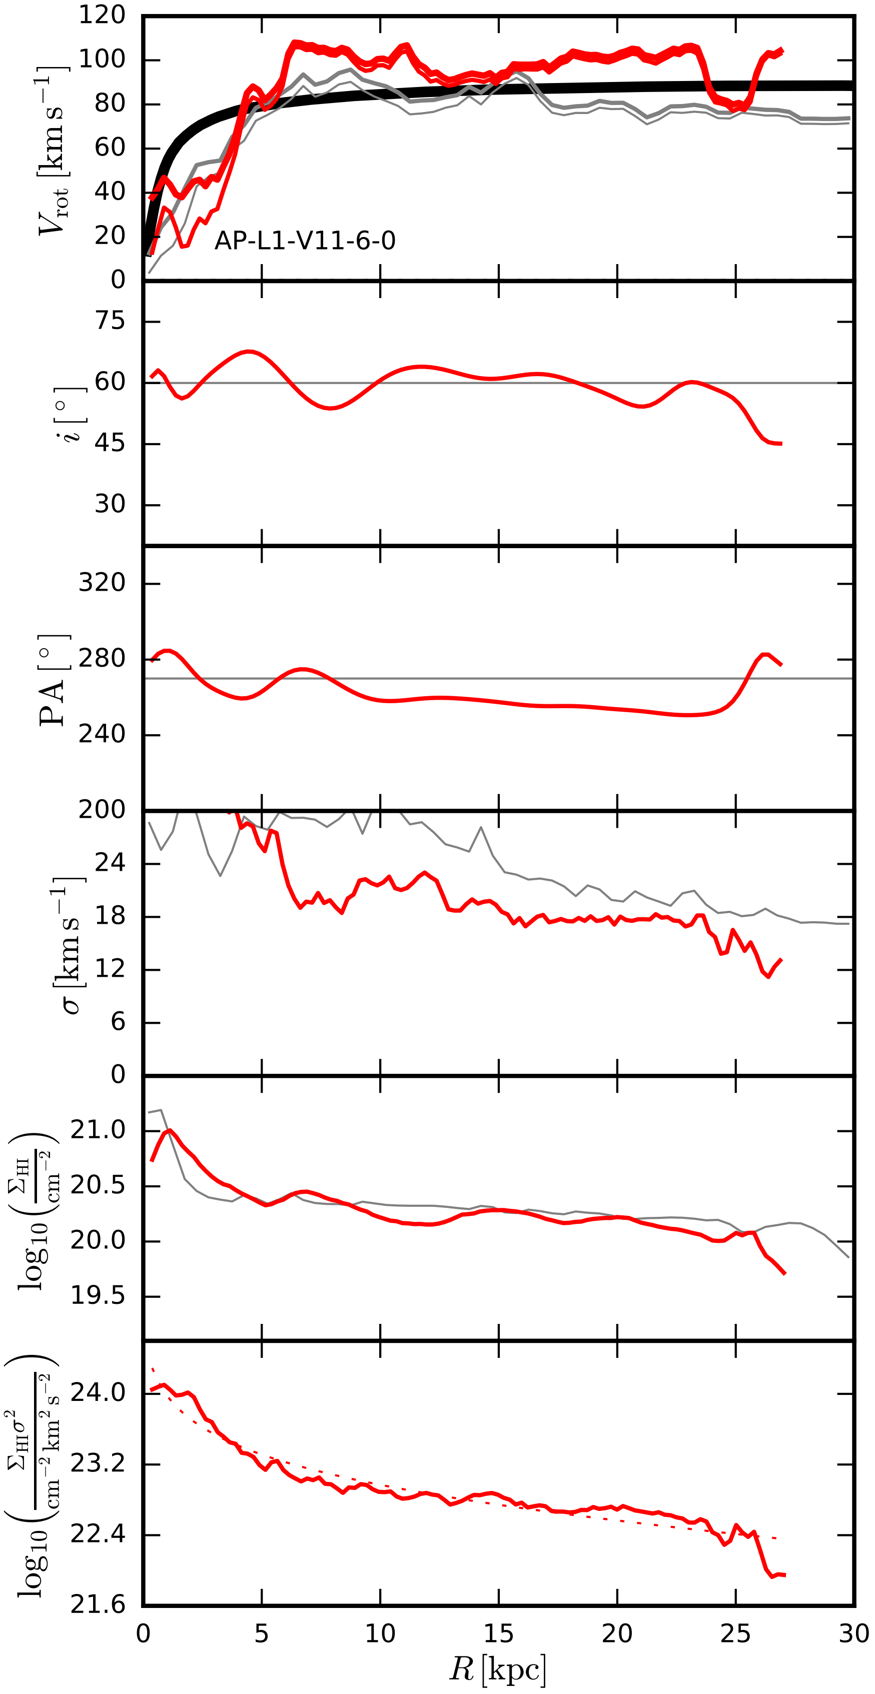


**Figure 33** – *continued*
